# Supplementary material for: Parquet theory for molecular systems: Formalism and static kernel parquet approximation
Source: arXiv:2509.03253 ancillary file (2025-11-05)
Supplement: Supplementary file 1 [file si.pdf]

# Supporting information for “Parquet theory for molecular systems. I. Formalism and static kernel parquet approximation”

Antoine Marie<sup>a)</sup> and Pierre-François Loos<sup>b)</sup>

*Laboratoire de Chimie et Physique Quantiques (UMR 5626), Université de Toulouse, CNRS, UPS, France*

This document contains the detailed derivations of the equations reported in the associated main manuscript, where missing notations can be found. The first three sections set the stage for the parquet formalism that is discussed in the remaining sections. Section I defines the time and Fourier transform conventions that are used in this work. The electron-hole (eh) and the particle-particle (pp) Bethe-Salpeter equations (BSEs) are presented in detail in Secs. II and III, respectively. In particular, these include their transformation to frequency space, their solution in a basis of spin-orbitals, as well as their spin adaptation. The presentation of parquet formalism starts with the Fourier transform of all its equations performed in Sec. IV. These equations are then projected in a basis of spin orbitals in Sec. V. Finally, Sec. VI reports the spin-adapted parquet equations.

## CONTENTS

|                                                       |    |
|-------------------------------------------------------|----|
| <b>I. Fourier transform</b>                           | 2  |
| A. Single-time convention                             | 2  |
| B. Three-time electron-hole convention                | 2  |
| C. Three-time particle-particle convention            | 2  |
| D. Link between conventions                           | 3  |
| <b>II. Electron-hole Bethe-Salpeter equation</b>      | 3  |
| A. Fourier transform                                  | 3  |
| B. Independent-particle propagator                    | 4  |
| C. Spin-orbital expression                            | 5  |
| D. Spin adaptation                                    | 6  |
| E. Spatial-orbital expression                         | 7  |
| <b>III. Particle-particle Bethe-Salpeter equation</b> | 8  |
| A. Fourier transform                                  | 8  |
| B. Independent-particle propagator                    | 9  |
| C. Spin-orbital expression                            | 10 |
| D. Spin adaptation                                    | 12 |
| E. Spatial-orbital expression                         | 13 |
| <b>IV. Fourier transform</b>                          | 14 |
| A. Bethe-Salpeter equations                           | 14 |
| B. Self-energy                                        | 14 |
| <b>V. Projection in spin-orbital basis</b>            | 15 |
| A. Link with common BSE kernels                       | 15 |
| B. Self-energy                                        | 16 |
| <b>VI. Spin-adapted Parquet theory</b>                | 23 |
| A. Bethe-Salpeter equations                           | 23 |
| B. Irreducible vertices                               | 25 |
| C. Self-energy                                        | 26 |

---

<sup>a)</sup>Electronic mail: [amarie@irsamc.ups-tlse.fr](mailto:amarie@irsamc.ups-tlse.fr)

<sup>b)</sup>Electronic mail: [loos@irsamc.ups-tlse.fr](mailto:loos@irsamc.ups-tlse.fr)

## I. FOURIER TRANSFORM

### A. Single-time convention

The electronic structure Hamiltonian is time-independent, which means that the 2-point quantities depend on a single time variable. The Fourier transform is defined as

$$G(\omega) = \int d\tau e^{i\omega\tau} G(\tau), \quad (1)$$

and the inverse Fourier transform is given by

$$G(\tau) = \frac{1}{2\pi} \int d\omega e^{-i\omega\tau} G(\omega). \quad (2)$$

### B. Three-time electron-hole convention

Once again, because the electronic structure Hamiltonian is time-independent, the 4-point quantities depend on only three time variables. There are multiple possible choices for these three independent time variables, some of which simplify the Fourier transforms of the quantities involved. However, a key challenge arises because different channels naturally favour different choices of time variables, and these channels become intertwined in the parquet decomposition of  $F$ . In this section and the next, we will define two distinct conventions.

The eh time-dependence convention is set to be

$$F(12; 34) = F(\mathbf{x}_1\mathbf{x}_2; \mathbf{x}_3\mathbf{x}_4; \tau_{13}, \tau_{24}, \tau_{23}), \quad (3)$$

and the associated three-time Fourier transform is defined as

$$F(\mathbf{x}_1\mathbf{x}_2; \mathbf{x}_3\mathbf{x}_4; \nu, \nu', \omega) = \int d(\tau_{13}\tau_{24}\tau_{23}) e^{i\nu\tau_{13} + i\nu'\tau_{24} + i\omega\tau_{23}} F(\mathbf{x}_1\mathbf{x}_2; \mathbf{x}_3\mathbf{x}_4; \tau_{13}, \tau_{24}, \tau_{23}). \quad (4)$$

In Matsubara terms, both  $\nu$  and  $\nu'$  are fermionic frequencies, whereas  $\omega$  is a bosonic frequency. This distinction arises because  $G_2$ , and consequently  $F$ , is antisymmetric with respect to the time arguments  $\tau_{13}$  and  $\tau_{24}$ , while it remains symmetric with respect to  $\tau_{23}$ .

The eh scattering corresponding to this convention is drawn in Fig. 1.<sup>1</sup> The pair of ingoing (blue) and outgoing (red) particles both have a total energy  $\omega$ , which is preserved through scattering. However, the energy difference between the two particles is allowed to vary.

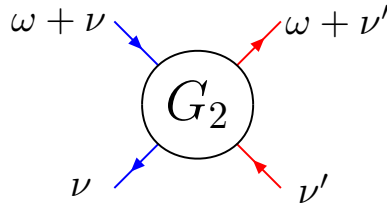

FIG. 1. Scattering of an eh pair of energy  $\omega$ . The blue (red) lines represent the ingoing (outgoing) particles.

### C. Three-time particle-particle convention

The pp time-dependence convention is set to be

$$F_P(12; 34) = F_P(\mathbf{x}_1\mathbf{x}_2; \mathbf{x}_3\mathbf{x}_4; \tau_{12}, \tau_{43}, \tau_{13}), \quad (5)$$

where the index P is here to indicate that the alternative convention has been used. The associated three-time Fourier transform is defined as

$$F_P(\mathbf{x}_1\mathbf{x}_2; \mathbf{x}_3\mathbf{x}_4; \nu, \nu', \omega) = \int d(\tau_{12}\tau_{43}\tau_{13}) e^{i\nu\tau_{12} + i\nu'\tau_{43} + i\omega\tau_{13}} F_P(\mathbf{x}_1\mathbf{x}_2; \mathbf{x}_3\mathbf{x}_4; \tau_{12}, \tau_{43}, \tau_{13}). \quad (6)$$

The electron-electron scattering corresponding to this convention is drawn in Fig. 2.<sup>1</sup> The pair of ingoing (blue) and outgoing (red) particles both have a total energy  $\omega$ , which is preserved through scattering. However, the energy difference between the two particles is allowed to vary.

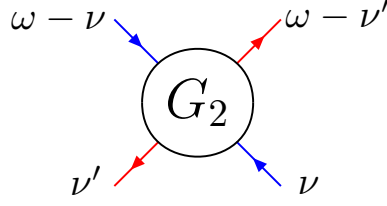

FIG. 2. Scattering of an ee pair of energy  $\omega$ . The blue (red) lines represent the ingoing (outgoing) particles.

#### D. Link between conventions

One can link these two conventions

$$\begin{aligned}
 F(\mathbf{x}_1 \mathbf{x}_2; \mathbf{x}_3 \mathbf{x}_4; \nu, \nu', \omega) &= \int d(\tau_{13} \tau_{24} \tau_{23}) e^{i\nu\tau_{13} + i\nu'\tau_{24} + i\omega\tau_{23}} F_P(\mathbf{x}_1 \mathbf{x}_2; \mathbf{x}_3 \mathbf{x}_4; \tau_{13} - \tau_{23}, -\tau_{24} + \tau_{23}, \tau_{13}) \\
 &= \frac{1}{(2\pi)^3} \int d(\omega_1 \omega_2 \omega_3) F_P(\mathbf{x}_1 \mathbf{x}_2; \mathbf{x}_3 \mathbf{x}_4; \omega_1, \omega_2, \omega_3) \\
 &\quad \times \int d(\tau_{13} \tau_{24} \tau_{23}) e^{i\nu\tau_{13} + i\nu'\tau_{24} + i\omega\tau_{23}} e^{-i\omega_1(\tau_{13} - \tau_{23})} e^{-i\omega_2(-\tau_{24} + \tau_{23})} e^{-i\omega_3\tau_{13}} \\
 &= \int d(\omega_1 \omega_2 \omega_3) F_P(\mathbf{x}_1 \mathbf{x}_2; \mathbf{x}_3 \mathbf{x}_4; \omega_1, \omega_2, \omega_3) \delta(\nu - \omega_1 - \omega_3) \delta(\nu' + \omega_2) \delta(\omega + \omega_1 - \omega_2),
 \end{aligned} \tag{7}$$

through a mere frequency shift

$$F(\mathbf{x}_1 \mathbf{x}_2; \mathbf{x}_3 \mathbf{x}_4; \nu, \nu', \omega) = F_P(\mathbf{x}_1 \mathbf{x}_2; \mathbf{x}_3 \mathbf{x}_4; -\omega - \nu', -\nu', \omega + \nu + \nu'). \tag{8}$$

This relation can be inverted to give

$$F_P(\mathbf{x}_1 \mathbf{x}_2; \mathbf{x}_3 \mathbf{x}_4; \nu, \nu', \omega) = F(\mathbf{x}_1 \mathbf{x}_2; \mathbf{x}_3 \mathbf{x}_4; \omega + \nu, -\nu', \nu' - \nu). \tag{9}$$

## II. ELECTRON-HOLE BETHE-SALPETER EQUATION

This section will discuss the solution of the eh-BSE

$$L(12; 1'2') = L_0(12; 1'2') + \int d(343'4') L_0(13'; 1'3) \Gamma^{\text{eh}}(34; 3'4') L(4'2; 42'), \tag{10}$$

in a finite basis of orbitals.

#### A. Fourier transform

Once the time indices are explicitly written down (in the eh convention of Sec. IB), the eh-BSE becomes

$$L(\tau_{11'}, \tau_{22'}, \tau_{21'}) = L_0(\tau_{11'}, \tau_{22'}, \tau_{21'}) + \int d(t_1' t_2' t_3' t_4') L_0(\tau_{11'}, \tau_{3'3}, \tau_{3'1'}) \Gamma^{\text{eh}}(\tau_{33'}, \tau_{44'}, \tau_{43'}) L(\tau_{4'4}, \tau_{22'}, \tau_{24}). \tag{11}$$

The spin-space indices are not written for the sake of conciseness. This can be Fourier transformed as

$$\begin{aligned}
L(\nu, \nu', \omega) &= L_0(\nu, \nu', \omega) + \int d\tau_{21'} e^{i\omega\tau_{21'}} \int d(t_3 t_4 t_3' t_4') L_0(\nu, \tau_{3'3}, \tau_{3'1'}) \Gamma^{\text{eh}}(\tau_{33'}, \tau_{44'}, \tau_{43'}) L(\tau_{4'4}, \nu', \tau_{24}) \\
&= L_0(\nu, \nu', \omega) + \frac{1}{(2\pi)^2} \int d(\nu_1 \nu_2) \int d\tau_{21'} e^{i\omega\tau_{21'}} \int d(t_4 t_3') L_0(\nu, \nu_1, \tau_{3'1'}) \Gamma^{\text{eh}}(\nu_1, \nu_2, \tau_{43'}) L(\nu_2, \nu', \tau_{24}) \quad (12) \\
&= L_0(\nu, \nu', \omega) + \frac{1}{(2\pi)^2} \int d(\nu_1 \nu_2) L_0(\nu, \nu_1, \omega) \Gamma^{\text{eh}}(\nu_1, \nu_2, \omega) L(\nu_2, \nu', \omega),
\end{aligned}$$

and this yields

$$\begin{aligned}
L(\mathbf{x}_1 \mathbf{x}_2; \mathbf{x}_1' \mathbf{x}_2'; \omega) &= L_0(\mathbf{x}_1 \mathbf{x}_2; \mathbf{x}_1' \mathbf{x}_2'; \omega) \\
&+ \frac{1}{(2\pi)^2} \int d(\nu_1 \nu_2) L_0(\mathbf{x}_1 \mathbf{x}_3'; \mathbf{x}_1' \mathbf{x}_3; \nu_1, \omega) \Gamma^{\text{eh}}(\mathbf{x}_3 \mathbf{x}_4; \mathbf{x}_3' \mathbf{x}_4'; \nu_1, \nu_2, \omega) L(\mathbf{x}_4' \mathbf{x}_2; \mathbf{x}_4 \mathbf{x}_2'; \nu_2, \omega), \quad (13)
\end{aligned}$$

once the eh pair is assumed to be created and annihilated instantaneously.<sup>2</sup>

Unfortunately, because the kernel depends on three frequencies, the above equation cannot be inverted. Following the methodology introduced for the usual eh-BSE case,<sup>3</sup> an effective dynamic kernel is defined as

$$\tilde{\Gamma}^{\text{eh}}(\omega) = \frac{1}{(2\pi)^2} \int d(\nu_1 \nu_2) (L_0^{-1})(\omega) L_0(\nu_1, \omega) \Gamma^{\text{eh}}(\nu_1, \nu_2, \omega) L(\nu_2, \omega) (L^{-1})(\omega), \quad (14)$$

such that the eh-BSE becomes

$$L(\omega) = L_0(\omega) + L_0(\omega) \tilde{\Gamma}^{\text{eh}}(\omega) L(\omega), \quad (15)$$

and is now easily invertible, as follows

$$L^{-1}(\mathbf{x}_1 \mathbf{x}_2; \mathbf{x}_1' \mathbf{x}_2'; \omega) = L_0^{-1}(\mathbf{x}_1 \mathbf{x}_2; \mathbf{x}_1' \mathbf{x}_2'; \omega) - \tilde{\Gamma}^{\text{eh}}(\mathbf{x}_1 \mathbf{x}_2; \mathbf{x}_1' \mathbf{x}_2'; \omega). \quad (16)$$

However, as readily seen in Eq. (14), its kernel self-consistently depends on  $L$ . In order to suppress this dependency, the effective kernel is approximated as

$$\tilde{\Gamma}^{\text{eh}}(\omega) = \frac{1}{(2\pi)^2} \int d(\nu_1 \nu_2) (L_0^{-1})(\omega) L_0(\nu_1, \omega) \Gamma^{\text{eh}}(\nu_1, \nu_2, \omega) L_0(\nu_2, \omega) (L_0^{-1})(\omega), \quad (17)$$

where one simply replaces the kernel  $L$  by its independent-particle version  $L_0$  in Eq. (14). Finally, note that if the kernel is static, or is assumed to be static, *i.e.*  $\Gamma^{\text{eh}}(\nu_1, \nu_2, \omega) = \Gamma^{\text{eh}}$ , the approximate dynamic kernel remains unchanged, *i.e.*  $\tilde{\Gamma}^{\text{eh}}(\omega) = \Gamma^{\text{eh}}$ .

## B. Independent-particle propagator

The eh non-interacting propagator is defined as

$$L_0(12; 1'2') = G(12') G(21'), \quad (18)$$

and its time-dependence (in the eh convention of Sec. IB) is

$$\begin{aligned}
L_0(\mathbf{x}_1 \mathbf{x}_2; \mathbf{x}_1' \mathbf{x}_2'; \tau_{11'}, \tau_{22'}, \tau_{21'}) &= G(\mathbf{x}_1 \mathbf{x}_2'; \tau_{12'}) G(\mathbf{x}_2 \mathbf{x}_1'; \tau_{21'}) \\
&= G(\mathbf{x}_1 \mathbf{x}_2'; \tau_{11'} - \tau_{21'} + \tau_{22'}) G(\mathbf{x}_2 \mathbf{x}_1'; \tau_{21'}). \quad (19)
\end{aligned}$$

It can be Fourier transformed as

$$\begin{aligned}
&L_0(\mathbf{x}_1 \mathbf{x}_2; \mathbf{x}_1' \mathbf{x}_2'; \nu, \nu', \omega) \\
&= \int d(\tau_{11'} \tau_{22'} \tau_{21'}) e^{i\nu\tau_{11'} + i\nu'\tau_{22'} + i\omega\tau_{21'}} \\
&\quad \times \left( \frac{1}{2\pi} \int d\omega_1 e^{-i\omega_1(\tau_{11'} - \tau_{21'} + \tau_{22'})} G(\mathbf{x}_1 \mathbf{x}_2'; \omega_1) \right) \left( \frac{1}{2\pi} \int d\omega_2 e^{-i\omega_2\tau_{21'}} G(\mathbf{x}_2 \mathbf{x}_1'; \omega_2) \right) \\
&= \frac{1}{(2\pi)^2} \int d(\omega_1 \omega_2) G(\mathbf{x}_1 \mathbf{x}_2'; \omega_1) G(\mathbf{x}_2 \mathbf{x}_1'; \omega_2) \\
&\quad \times \left( \int d\tau_{13} e^{i\nu\tau_{11'}} e^{-i\omega_1\tau_{11'}} \right) \left( \int d\tau_{22'} e^{i\nu'\tau_{22'}} e^{-i\omega_1\tau_{22'}} \right) \left( \int d\tau_{21'} e^{i\omega\tau_{21'}} e^{i\omega_1\tau_{21'}} e^{-i\omega_2\tau_{21'}} \right) \\
&= 2\pi G(\mathbf{x}_1 \mathbf{x}_2'; \nu) G(\mathbf{x}_2 \mathbf{x}_1'; \omega + \nu) \delta(\nu - \nu'). \quad (20)
\end{aligned}$$

The single-frequency propagator is obtained by integrating out the two fermionic frequencies

$$L_0(\mathbf{x}_1\mathbf{x}_2; \mathbf{x}_{1'}\mathbf{x}_{2'}; \omega) = \frac{1}{2\pi} \int d\nu G(\mathbf{x}_1\mathbf{x}_{2'}; \nu + \omega) G(\mathbf{x}_2\mathbf{x}_{1'}; \nu), \quad (21)$$

and can be computed as

$$\begin{aligned} L_0(\mathbf{x}_1\mathbf{x}_2; \mathbf{x}_{1'}\mathbf{x}_{2'}; \omega) &= \frac{1}{2\pi} \int d\nu \left( \sum_i \frac{\varphi_i(\mathbf{x}_1)\varphi_i^*(\mathbf{x}_{2'})}{\nu - (\epsilon_i - \omega + i\eta)} + \sum_a \frac{\varphi_a(\mathbf{x}_1)\varphi_a^*(\mathbf{x}_{2'})}{\nu - (\epsilon_a - \omega - i\eta)} \right) \left( \sum_j \frac{\varphi_j(\mathbf{x}_2)\varphi_j^*(\mathbf{x}_{1'})}{\nu - (\epsilon_j + i\eta)} + \sum_b \frac{\varphi_b(\mathbf{x}_2)\varphi_b^*(\mathbf{x}_{1'})}{\nu - (\epsilon_b - i\eta)} \right) \\ &= \frac{1}{2\pi} \int d\nu \sum_{ib} \frac{\varphi_i(\mathbf{x}_1)\varphi_i^*(\mathbf{x}_{2'})}{\nu - (\epsilon_i - \omega + i\eta)} \frac{\varphi_b(\mathbf{x}_2)\varphi_b^*(\mathbf{x}_{1'})}{\nu - (\epsilon_b - i\eta)} + \frac{1}{2\pi} \int d\nu \sum_{ja} \frac{\varphi_a(\mathbf{x}_1)\varphi_a^*(\mathbf{x}_{2'})}{\nu - (\epsilon_a - \omega - i\eta)} \frac{\varphi_j(\mathbf{x}_2)\varphi_j^*(\mathbf{x}_{1'})}{\nu - (\epsilon_j + i\eta)} \\ &= i \sum_{ib} \frac{\varphi_i(\mathbf{x}_1)\varphi_i^*(\mathbf{x}_{2'})\varphi_b(\mathbf{x}_2)\varphi_b^*(\mathbf{x}_{1'})}{(\epsilon_i - \omega + i\eta) - (\epsilon_b - i\eta)} + i \sum_{ja} \frac{\varphi_a(\mathbf{x}_1)\varphi_a^*(\mathbf{x}_{2'})\varphi_j(\mathbf{x}_2)\varphi_j^*(\mathbf{x}_{1'})}{(\epsilon_j + i\eta) - (\epsilon_a - \omega - i\eta)} \\ &= -i \sum_{ib} \frac{\varphi_i(\mathbf{x}_1)\varphi_i^*(\mathbf{x}_{2'})\varphi_b(\mathbf{x}_2)\varphi_b^*(\mathbf{x}_{1'})}{\omega - (\epsilon_i - \epsilon_b + 2i\eta)} + i \sum_{ja} \frac{\varphi_a(\mathbf{x}_1)\varphi_a^*(\mathbf{x}_{2'})\varphi_j(\mathbf{x}_2)\varphi_j^*(\mathbf{x}_{1'})}{\omega - (\epsilon_a - \epsilon_j - 2i\eta)}. \end{aligned} \quad (22)$$

Once projected in a basis, this yields

$$(L_0)_{pqrs}(\omega) = i \sum_{ia} \frac{\delta_{pa}\delta_{sa}\delta_{qi}\delta_{ri}}{\omega - (\epsilon_a - \epsilon_i - 2i\eta)} - i \sum_{ia} \frac{\delta_{pi}\delta_{si}\delta_{qa}\delta_{ra}}{\omega - (\epsilon_i - \epsilon_a + 2i\eta)}. \quad (23)$$

### C. Spin-orbital expression

Once projected in a basis set, the eh-BSE reads

$$(L)_{pqrs}(\omega) = (L_0)_{pqrs}(\omega) + (L_0)_{ptru}(\omega) \tilde{\Gamma}_{uvtw}^{\text{eh}}(\omega) L_{wqvs}(\omega), \quad (24)$$

or

$$(L)_{pqrs}^{-1}(\omega) = (L_0)_{pqrs}^{-1}(\omega) - \tilde{\Gamma}_{pqrs}^{\text{eh}}(\omega), \quad (25)$$

where the independent-particle propagator tensor can be transformed into a diagonal matrix by defining composite indices  $\mathbf{L}_0 = (L_0)_{rp,qs}$

$$\begin{aligned} (\mathbf{L}_0)^{-1} &= \begin{pmatrix} (L_0)_{ia,ia} & \mathbf{0} \\ \mathbf{0} & (L_0)_{ai,ai} \end{pmatrix}^{-1} = \begin{pmatrix} -i \text{diag}[\omega - (\epsilon_a - \epsilon_i)] & \mathbf{0} \\ \mathbf{0} & i \text{diag}[\omega + (\epsilon_a - \epsilon_i)] \end{pmatrix} \\ &= -i \begin{pmatrix} \boldsymbol{\omega} & \mathbf{0} \\ \mathbf{0} & -\boldsymbol{\omega} \end{pmatrix} + i \begin{pmatrix} \epsilon_{ai} & \mathbf{0} \\ \mathbf{0} & \epsilon_{ai} \end{pmatrix}, \end{aligned} \quad (26)$$

where  $\epsilon_{ai} = \text{diag}(\epsilon_a - \epsilon_i)$  and  $\boldsymbol{\omega} = \omega \mathbf{1}$ . Hence, the BSE can be written as

$$\mathbf{L}^{-1}(\omega) = \mathbf{L}_0^{-1}(\omega) - \tilde{\Gamma}^{\text{eh}}(\omega) = -i \left[ \begin{pmatrix} \boldsymbol{\omega} & \mathbf{0} \\ \mathbf{0} & -\boldsymbol{\omega} \end{pmatrix} - \begin{pmatrix} \epsilon_{ai} & \mathbf{0} \\ \mathbf{0} & \epsilon_{ai} \end{pmatrix} - i \tilde{\Gamma}^{\text{eh}}(\omega) \right] = -i \mathcal{M} \cdot [\omega \mathbf{1} - \mathcal{H}^{\text{eh}}(\omega)], \quad (27)$$

where the metric  $\mathcal{M}$  and the effective Hamiltonian matrix  $\mathcal{H}^{\text{eh}}(\omega)$  are defined as

$$\mathcal{M} = \begin{pmatrix} \mathbf{1} & \mathbf{0} \\ \mathbf{0} & -\mathbf{1} \end{pmatrix}, \quad \mathcal{H}^{\text{eh}}(\omega) = \begin{pmatrix} \mathbf{A}^{\text{eh}}(\omega) & \mathbf{B}^{\text{eh}} \\ -(\mathbf{B}^{\text{eh}})^\dagger & -(\mathbf{A}^{\text{eh}})^\dagger(\omega) \end{pmatrix}, \quad (28)$$

in terms of the blocks given by

$$A_{ia,jb}^{\text{eh}}(\omega) = (\epsilon_a - \epsilon_i) \delta_{ab} \delta_{ij} + i \tilde{\Gamma}_{ajib}^{\text{eh}}(\omega), \quad (29a)$$

$$B_{ia,bj}^{\text{eh}} = i \tilde{\Gamma}_{abij}^{\text{eh}}. \quad (29b)$$

The eigenvalue decomposition of the latter is written as  $(\mathcal{L}^{\text{eh}})^\dagger \cdot \mathcal{E}^{\text{eh}} \cdot \mathcal{R}^{\text{eh}}$ , where the diagonal matrix  $\mathcal{E}^{\text{eh}}$  gathers the eigenvalues, and the left and right eigenvectors are given by

$$\mathcal{H}^{\text{eh}} \cdot \mathcal{R}^{\text{eh}} = \mathcal{R}^{\text{eh}} \cdot \mathcal{E}^{\text{eh}}, \quad (\mathcal{H}^{\text{eh}})^\dagger \cdot \mathcal{L}^{\text{eh}} = \mathcal{L}^{\text{eh}} \cdot \mathcal{E}^{\text{eh}}, \quad (30)$$

and fulfil the orthonormality condition  $(\mathcal{L}^{\text{eh}})^\dagger \cdot \mathcal{R}^{\text{eh}} = \mathbf{1}$ . More precisely, the eigenvectors can be written as

$$\mathcal{L}^{\text{eh}} = \begin{pmatrix} (\mathbf{X}^{\text{eh}})^\dagger & -\mathbf{Y}^{\text{eh}} \\ -(\mathbf{Y}^{\text{eh}})^\dagger & \mathbf{X}^{\text{eh}} \end{pmatrix}, \quad \mathcal{R}^{\text{eh}} = \begin{pmatrix} \mathbf{X}^{\text{eh}} & (\mathbf{Y}^{\text{eh}})^\dagger \\ \mathbf{Y}^{\text{eh}} & (\mathbf{X}^{\text{eh}})^\dagger \end{pmatrix}, \quad (31)$$

and the eigenvalue matrix is

$$\mathcal{E}^{\text{eh}} = \begin{pmatrix} \Omega^{\text{eh}} & \mathbf{0} \\ \mathbf{0} & -\Omega^{\text{eh}} \end{pmatrix}. \quad (32)$$

The inverse propagator can be written as

$$\mathbf{L}^{-1}(\omega) = -i\mathcal{M} \cdot (\mathcal{L}^{\text{eh}})^\dagger \cdot [\omega\mathbf{1} - \mathcal{E}^{\text{eh}}] \cdot \mathcal{R}^{\text{eh}}, \quad (33)$$

and then inverted

$$\mathbf{L}(\omega) = i\mathcal{R}^{\text{eh}} \cdot [\omega\mathbf{1} - \mathcal{E}^{\text{eh}}]^{-1} \cdot (\mathcal{L}^{\text{eh}})^\dagger \cdot \mathcal{M}, \quad (34)$$

to finally give

$$\mathbf{L}(\omega) = i \begin{pmatrix} L_1(\omega) & L_2(\omega) \\ L_3(\omega) & L_4(\omega) \end{pmatrix}, \quad (35)$$

with

$$L_1(\omega) = \mathbf{X}^{\text{eh}} \cdot [\omega\mathbf{1} - \Omega^{\text{eh}}]^{-1} \cdot (\mathbf{X}^{\text{eh}})^\dagger - (\mathbf{Y}^{\text{eh}})^* \cdot [\omega\mathbf{1} + \Omega^{\text{eh}}]^{-1} \cdot (\mathbf{Y}^{\text{eh}})^\dagger, \quad (36a)$$

$$L_2(\omega) = \mathbf{X}^{\text{eh}} \cdot [\omega\mathbf{1} - \Omega^{\text{eh}}]^{-1} \cdot (\mathbf{Y}^{\text{eh}})^\dagger - (\mathbf{Y}^{\text{eh}})^* \cdot [\omega\mathbf{1} + \Omega^{\text{eh}}]^{-1} \cdot (\mathbf{X}^{\text{eh}})^\dagger, \quad (36b)$$

$$L_3(\omega) = \mathbf{Y}^{\text{eh}} \cdot [\omega\mathbf{1} - \Omega^{\text{eh}}]^{-1} \cdot (\mathbf{X}^{\text{eh}})^\dagger - (\mathbf{X}^{\text{eh}})^* \cdot [\omega\mathbf{1} + \Omega^{\text{eh}}]^{-1} \cdot (\mathbf{X}^{\text{eh}})^\dagger, \quad (36c)$$

$$L_4(\omega) = \mathbf{Y}^{\text{eh}} \cdot [\omega\mathbf{1} - \Omega^{\text{eh}}]^{-1} \cdot (\mathbf{Y}^{\text{eh}})^\dagger - (\mathbf{X}^{\text{eh}})^* \cdot [\omega\mathbf{1} + \Omega^{\text{eh}}]^{-1} \cdot (\mathbf{X}^{\text{eh}})^\dagger. \quad (36d)$$

This matrix can be written as

$$L_{rp,qs}(\omega) = i \sum_n \frac{\rho_{rp,n}^{\text{eh}} \rho_{qs,n}^{\text{eh},*}}{\omega - (\Omega_n^{\text{eh}} - i\eta)} - i \sum_n \frac{\rho_{pr,n}^{\text{eh},*} \rho_{sq,n}^{\text{eh}}}{\omega - (-\Omega_n^{\text{eh}} + i\eta)}, \quad (37)$$

where

$$\rho_{rp,n}^{\text{eh}} = \sum_{jb} \left[ X_{jb,n}^{\text{eh}} \delta_{rb} \delta_{pj} + Y_{bj,n}^{\text{eh}} \delta_{rj} \delta_{pb} \right]. \quad (38)$$

#### D. Spin adaptation

The eh-BSE for the three different spin combination reads

$$L(1\uparrow 2\uparrow; 1'\uparrow 2'\uparrow) = L_0(1\uparrow 2\uparrow; 1'\uparrow 2'\uparrow) + \sum_{\substack{\sigma_3 \sigma_4 \\ \sigma_3' \sigma_4'}} L_0(1\uparrow 3'_{\sigma_3}; 1'\uparrow 3_{\sigma_3}) \Gamma^{\text{eh}}(3_{\sigma_3} 4_{\sigma_4}; 3'_{\sigma_3'} 4'_{\sigma_4'}) L(4'_{\sigma_4'} 2\uparrow; 4_{\sigma_4} 2'\uparrow), \quad (39a)$$

$$L(1\uparrow 2\downarrow; 1'\uparrow 2'\downarrow) = L_0(1\uparrow 2\downarrow; 1'\uparrow 2'\downarrow) + \sum_{\substack{\sigma_3 \sigma_4 \\ \sigma_3' \sigma_4'}} L_0(1\uparrow 3'_{\sigma_3}; 1'\uparrow 3_{\sigma_3}) \Gamma^{\text{eh}}(3_{\sigma_3} 4_{\sigma_4}; 3'_{\sigma_3'} 4'_{\sigma_4'}) L(4'_{\sigma_4'} 2\downarrow; 4_{\sigma_4} 2'\downarrow), \quad (39b)$$

$$L(1\uparrow 2\downarrow; 1'\downarrow 2'\uparrow) = L_0(1\uparrow 2\downarrow; 1'\downarrow 2'\uparrow) + \sum_{\substack{\sigma_3 \sigma_4 \\ \sigma_3' \sigma_4'}} L_0(1\uparrow 3'_{\sigma_3}; 1'\downarrow 3_{\sigma_3}) \Gamma^{\text{eh}}(3_{\sigma_3} 4_{\sigma_4}; 3'_{\sigma_3'} 4'_{\sigma_4'}) L(4'_{\sigma_4'} 2\downarrow; 4_{\sigma_4} 2'\uparrow), \quad (39c)$$

where we have made explicit the sum over integrated spin variables. The spin independence of  $G$  can be used to simplify these sums

$$L(1\uparrow 2\uparrow; 1'2\uparrow) = L_0(1\uparrow 2\uparrow; 1'2\uparrow) + \sum_{\sigma_4 \sigma_{4'}} L_0(1\uparrow 3\uparrow; 1'3\uparrow) \Gamma^{\text{eh}}(3\uparrow 4\sigma_4; 3'\uparrow 4'\sigma_{4'}) L(4'\sigma_{4'} 2\uparrow; 4\sigma_4 2\uparrow), \quad (40a)$$

$$L(1\uparrow 2\downarrow; 1'2\downarrow) = L_0(1\uparrow 2\downarrow; 1'2\downarrow) + \sum_{\sigma_4 \sigma_{4'}} L_0(1\uparrow 3\uparrow; 1'3\uparrow) \Gamma^{\text{eh}}(3\uparrow 4\sigma_4; 3'\uparrow 4'\sigma_{4'}) L(4'\sigma_{4'} 2\downarrow; 4\sigma_4 2\downarrow), \quad (40b)$$

$$L(1\uparrow 2\downarrow; 1'2\uparrow) = L_0(1\uparrow 2\downarrow; 1'2\uparrow) + \sum_{\sigma_4 \sigma_{4'}} L_0(1\uparrow 3\downarrow; 1'3\uparrow) \Gamma^{\text{eh}}(3\uparrow 4\sigma_{4'}; 3'\downarrow 4'\sigma_{4'}) L(4'\sigma_{4'} 2\downarrow; 4\sigma_4 2\uparrow). \quad (40c)$$

They can be further simplified by considering only the non-zero spin combinations for two-body quantities

$$\begin{aligned} L(1\uparrow 2\uparrow; 1'2\uparrow) &= L_0(\mathbf{rt}_1 \mathbf{rt}_2; \mathbf{rt}_1' \mathbf{rt}_2') \\ &+ L_0(\mathbf{rt}_1 \mathbf{rt}_{3'}; \mathbf{rt}_1' \mathbf{rt}_3) \left[ \Gamma^{\text{eh}}(3\uparrow 4\uparrow; 3'\uparrow 4'\uparrow) L(4'\uparrow 2\uparrow; 4\uparrow 2\uparrow) + \Gamma^{\text{eh}}(3\uparrow 4\downarrow; 3'\uparrow 4'\downarrow) L(4'\downarrow 2\uparrow; 4\downarrow 2\uparrow) \right], \end{aligned} \quad (41a)$$

$$\begin{aligned} L(1\uparrow 2\downarrow; 1'2\downarrow) &= 0 \\ &+ L_0(\mathbf{rt}_1 \mathbf{rt}_{3'}; \mathbf{rt}_1' \mathbf{rt}_3) \left[ \Gamma^{\text{eh}}(3\uparrow 4\uparrow; 3'\uparrow 4'\uparrow) L(4'\uparrow 2\downarrow; 4\uparrow 2\downarrow) + \Gamma^{\text{eh}}(3\uparrow 4\downarrow; 3'\uparrow 4'\downarrow) L(4'\downarrow 2\downarrow; 4\downarrow 2\downarrow) \right], \end{aligned} \quad (41b)$$

$$L(1\uparrow 2\downarrow; 1'2\uparrow) = L_0(\mathbf{rt}_1 \mathbf{rt}_2; \mathbf{rt}_1' \mathbf{rt}_2') + L_0(\mathbf{rt}_1 \mathbf{rt}_{3'}; \mathbf{rt}_1' \mathbf{rt}_3) \left[ \Gamma^{\text{eh}}(3\uparrow 4\downarrow; 3'\downarrow 4'\uparrow) L(4'\uparrow 2\downarrow; 4\downarrow 2\uparrow) \right]. \quad (41c)$$

For an eh propagator, the incoming electron and hole have indices 2 and 2', respectively. The corresponding outgoing particles have indices 1' and 1. The eh pair with spin  $S_z = -1$  is  $\downarrow\uparrow$  and the corresponding propagator  $L_{\uparrow\downarrow\uparrow}$  is decoupled from the other propagators and, therefore, is already spin-adapted. It corresponds to the propagation of a  $S_z = -1$  triplet eh pair. The remaining two components  $L_{\uparrow\uparrow\uparrow}$  and  $L_{\uparrow\downarrow\downarrow}$  are coupled. They correspond to the propagation of  $S_z = 0$  eh pairs and can be spin-adapted through

$$L^{\text{d}}(\mathbf{rt}_1 \mathbf{rt}_2; \mathbf{rt}_1' \mathbf{rt}_2') = L(1\uparrow 2\uparrow; 1'2\uparrow) + L(1\uparrow 2\downarrow; 1'2\downarrow), \quad (42a)$$

$$L^{\text{m}}(\mathbf{rt}_1 \mathbf{rt}_2; \mathbf{rt}_1' \mathbf{rt}_2') = L(1\uparrow 2\uparrow; 1'2\uparrow) - L(1\uparrow 2\downarrow; 1'2\downarrow), \quad (42b)$$

leading to two decoupled BSEs

$$L^{\text{d}}(\mathbf{rt}_1 \mathbf{rt}_2; \mathbf{rt}_1' \mathbf{rt}_2') = L_0(\mathbf{rt}_1 \mathbf{rt}_2; \mathbf{rt}_1' \mathbf{rt}_2') + L_0(\mathbf{rt}_1 \mathbf{rt}_{3'}; \mathbf{rt}_1' \mathbf{rt}_3) \Gamma^{\text{d}}(\mathbf{rt}_3 \mathbf{rt}_4; \mathbf{rt}_3' \mathbf{rt}_{4'}) L^{\text{d}}(\mathbf{rt}_4' \mathbf{rt}_2; \mathbf{rt}_4 \mathbf{rt}_2'), \quad (43a)$$

$$L^{\text{m}}(\mathbf{rt}_1 \mathbf{rt}_2; \mathbf{rt}_1' \mathbf{rt}_2') = L_0(\mathbf{rt}_1 \mathbf{rt}_2; \mathbf{rt}_1' \mathbf{rt}_2') + L_0(\mathbf{rt}_1 \mathbf{rt}_{3'}; \mathbf{rt}_1' \mathbf{rt}_3) \Gamma^{\text{m}}(\mathbf{rt}_3 \mathbf{rt}_4; \mathbf{rt}_3' \mathbf{rt}_{4'}) L^{\text{m}}(\mathbf{rt}_4' \mathbf{rt}_2; \mathbf{rt}_4 \mathbf{rt}_2'). \quad (43b)$$

These two spin-adapted propagators are referred to as the density  $L^{\text{d}}$  and magnetic  $L^{\text{m}}$  propagators, respectively, and they correspond to the propagation of  $S_z = 0/S = 0$  and  $S_z = 0/S = 1$  eh pairs.

## E. Spatial-orbital expression

The BSEs for the density and magnetic eh propagators can be solved in the exact same way as the BSE for the full eh propagator, but in spatial orbital basis rather than in spin-orbital basis. Hence, solving the density channel BSE is equivalent to diagonalizing an effective Hamiltonian matrix  $\mathcal{H}^{\text{d}}(\omega)$  defined as

$$\mathcal{H}^{\text{d}}(\omega) = \begin{pmatrix} \mathbf{A}^{\text{d}}(\omega) & \mathbf{B}^{\text{d}} \\ -\mathbf{B}^{\text{d},\dagger} & -\mathbf{A}^{\text{d},\dagger}(\omega) \end{pmatrix}, \quad (44)$$

in terms of

$$A_{ia,jb}^{\text{d}}(\omega) = (\epsilon_a - \epsilon_i) \delta_{ab} \delta_{ij} + i \tilde{\Gamma}_{ajib}^{\text{d}}(\omega), \quad (45a)$$

$$B_{ia,bj}^{\text{d}} = i \tilde{\Gamma}_{abij}^{\text{d}}, \quad (45b)$$

where the tensor elements of the kernel are given by

$$\tilde{\Gamma}_{pqrs}^{\text{d}}(\omega) = \tilde{\Gamma}_{p\uparrow q\uparrow r\uparrow s\uparrow}^{\text{eh}}(\omega) + \tilde{\Gamma}_{p\uparrow q\downarrow r\uparrow s\downarrow}^{\text{eh}}(\omega). \quad (46)$$

On the other hand, the effective Hamiltonian matrix  $\mathcal{H}^m(\omega)$  to diagonalize for the magnetic channel BSE is given by

$$\mathcal{H}^m(\omega) = \begin{pmatrix} \mathbf{A}^m(\omega) & \mathbf{B}^m \\ -\mathbf{B}^{m,\dagger} & -\mathbf{A}^{m,\dagger}(\omega) \end{pmatrix}, \quad (47)$$

in terms of

$$A_{ia,jb}^m(\omega) = (\epsilon_a - \epsilon_i)\delta_{ab}\delta_{ij} + i\tilde{\Gamma}_{ajib}^m(\omega), \quad (48a)$$

$$B_{ia,bj}^m = +i\tilde{\Gamma}_{abij}^m, \quad (48b)$$

where the tensor elements of the kernel are given by

$$\tilde{\Gamma}_{pqrs}^m(\omega) = \tilde{\Gamma}_{p\uparrow q\downarrow r\downarrow s\uparrow}^{\text{eh}}(\omega). \quad (49)$$

### III. PARTICLE-PARTICLE BETHE-SALPETER EQUATION

This section will discuss the solution of the pp-BSE

$$K(12; 1'2') = K_0(12; 1'2') - \frac{1}{2} \int d(33'44') K_0(12; 33') \Gamma^{\text{pp}}(33'; 44') K_0(44'; 1'2'), \quad (50)$$

in a finite basis of orbitals.

#### A. Fourier transform

In the pp time convention, the pp-BSE is

$$K_{\text{P}}(\tau_{12}, \tau_{2'1'}, \tau_{11'}) = K_{0,\text{P}}(\tau_{12}, \tau_{2'1'}, \tau_{11'}) - \frac{1}{2} \int d(t_3 t_4 t_{3'} t_{4'}) K_{0,\text{P}}(\tau_{12}, \tau_{33'}, \tau_{13}) \Gamma_{\text{P}}^{\text{pp}}(\tau_{3'3}, \tau_{44'}, \tau_{34}) K_{\text{P}}(\tau_{4'4}, \tau_{2'1'}, \tau_{41'}), \quad (51)$$

where the pp non-interacting propagator has been defined in Eq. (58). The pp time convention will be used throughout this section and will be dropped for the sake of conciseness. Once Fourier transformed, it becomes

$$K(\nu, \nu', \omega) = K_0(\nu, \nu', \omega) - \frac{1}{2(2\pi)^2} \int d(\nu_1 \nu_2) K_0(\nu, \nu_1, \omega) \Gamma^{\text{pp}}(\nu_1, \nu_2, \omega) K(\nu_2, \nu', \omega), \quad (52)$$

which simplifies as

$$K(\mathbf{x}_1 \mathbf{x}_2; \mathbf{x}_1' \mathbf{x}_2'; \omega) = K_0(\mathbf{x}_1 \mathbf{x}_2; \mathbf{x}_1' \mathbf{x}_2'; \omega) - \frac{1}{2(2\pi)^2} \int d(\nu_1 \nu_2) K_0(\mathbf{x}_1 \mathbf{x}_2; \mathbf{x}_3 \mathbf{x}_3'; -\eta, \nu_1, \omega) \Gamma^{\text{pp}}(\mathbf{x}_3 \mathbf{x}_3'; \mathbf{x}_4 \mathbf{x}_4'; \nu_1, \nu_2, \omega) K(\mathbf{x}_4 \mathbf{x}_4'; \mathbf{x}_1' \mathbf{x}_2'; \nu_2, \eta, \omega), \quad (53)$$

once the pp pair is assumed to be created and annihilated instantaneously.<sup>2</sup>

Unfortunately, because the kernel depends on three frequencies, the above equation cannot be inverted. Following the methodology introduced for the usual eh-BSE case,<sup>3</sup> an effective dynamic kernel is defined as<sup>4</sup>

$$\tilde{\Gamma}^{\text{pp}}(\omega) = \frac{1}{(2\pi)^2} \int d(\nu_1 \nu_2) (K^{-1})(\omega) K(-\eta, \nu_1, \omega) \Gamma^{\text{pp}}(\nu_1, \nu_2, \omega) K_0(\nu_2, \eta, \omega) (K_0^{-1})(\omega), \quad (54)$$

such that the pp-BSE becomes

$$K(\omega) = K_0(\omega) - \frac{1}{2} K(\omega) \tilde{\Gamma}^{\text{pp}}(\omega) K_0(\omega), \quad (55)$$

and is now easily invertible, as follows

$$K^{-1}(\mathbf{x}_1 \mathbf{x}_2; \mathbf{x}_1' \mathbf{x}_2'; \omega) = K_0^{-1}(\mathbf{x}_1 \mathbf{x}_2; \mathbf{x}_1' \mathbf{x}_2'; \omega) + \frac{1}{2} \tilde{\Gamma}^{\text{pp}}(\mathbf{x}_1 \mathbf{x}_2; \mathbf{x}_1' \mathbf{x}_2'; \omega). \quad (56)$$



However, as readily seen in Eq. (54), its kernel self-consistently depends on  $K$ . In order to suppress this dependency, the effective kernel is approximated as

$$\tilde{\Gamma}^{\text{pp}}(\omega) \approx \frac{1}{(2\pi)^2} \int d(\nu_1 \nu_2) (K_0^{-1})(\omega) K_0(-\eta, \nu_1, \omega) \Gamma^{\text{pp}}(\nu_1, \nu_2, \omega) K_0(\nu_2, \eta, \omega) (K_0^{-1})(\omega), \quad (57)$$

where one simply replaces the kernel  $K$  by its independent-particle version  $K_0$  in Eq. (54). Finally, note that if the kernel is static, or is assumed to be static, *i.e.*  $\Gamma^{\text{pp}}(\nu_1, \nu_2, \omega) = \Gamma^{\text{pp}}$ , the approximate dynamic kernel remains unchanged, *i.e.*  $\tilde{\Gamma}^{\text{pp}}(\omega) = \Gamma^{\text{pp}}$ .

## B. Independent-particle propagator

The pp non-interacting propagator is defined as

$$K_0(12; 1'2') = \frac{1}{2} [G(11')G(22') - G(12')G(21')], \quad (58)$$

and its time-dependence (in the pp convention of Sec. IC) is

$$\begin{aligned} & K_0(\mathbf{x}_1 \mathbf{x}_2; \mathbf{x}'_1 \mathbf{x}'_2; \tau_{12}, \tau_{2'1'}, \tau_{11'}) \\ &= \frac{1}{2} G(\mathbf{x}_1 \mathbf{x}_{1'}; \tau_{11'}) G(\mathbf{x}_2 \mathbf{x}_{2'}; \tau_{22'}) - \frac{1}{2} G(\mathbf{x}_1 \mathbf{x}_{2'}; \tau_{12'}) G(\mathbf{x}_2 \mathbf{x}_{1'}; \tau_{21'}) \\ &= \frac{1}{2} G(\mathbf{x}_1 \mathbf{x}_{1'}; \tau_{11'}) G(\mathbf{x}_2 \mathbf{x}_{2'}; -\tau_{12} + \tau_{11'} - \tau_{2'1'}) - \frac{1}{2} G(\mathbf{x}_1 \mathbf{x}_{2'}; \tau_{11'} - \tau_{2'1'}) G(\mathbf{x}_2 \mathbf{x}_{1'}; -\tau_{12} + \tau_{11'}) \\ &= K_0^{\text{I}}(\mathbf{x}_1 \mathbf{x}_2; \mathbf{x}_1' \mathbf{x}_2'; \tau_{12}, \tau_{2'1'}, \tau_{11'}) + K_0^{\text{II}}(\mathbf{x}_1 \mathbf{x}_2; \mathbf{x}_3 \mathbf{x}_4; \tau_{12}, \tau_{2'1'}, \tau_{11'}). \end{aligned} \quad (59)$$

The first term can be Fourier transformed as

$$\begin{aligned} & K_0^{\text{I}}(\mathbf{x}_1 \mathbf{x}_2; \mathbf{x}_1' \mathbf{x}_2'; \nu, \nu', \omega) \\ &= \frac{1}{2} \int d(\tau_{12} \tau_{2'1'} \tau_{11'}) e^{i\nu\tau_{12} + i\nu'\tau_{2'1'} + i\omega\tau_{11'}} \\ &\quad \times \left( \frac{1}{2\pi} \int d\omega_1 e^{-i\tau_{11'}\omega_1} G(\mathbf{x}_1 \mathbf{x}_{1'}; \omega_1) \right) \left( \frac{1}{2\pi} \int d\omega_2 e^{-i(-\tau_{12} + \tau_{11'} - \tau_{2'1'})\omega_2} G(\mathbf{x}_2 \mathbf{x}_{2'}; \omega_2) \right) \\ &= \frac{1}{2(2\pi)^2} \int d(\omega_1 \omega_2) G(\mathbf{x}_1 \mathbf{x}_{1'}; \omega_1) G(\mathbf{x}_2 \mathbf{x}_{2'}; \omega_2) \\ &\quad \times \left( \int d\tau_{12} e^{i\nu\tau_{12}} e^{i\tau_{12}\omega_2} \right) \left( \int d\tau_{2'1'} e^{i\nu'\tau_{2'1'}} e^{i\tau_{2'1'}\omega_2} \right) \left( \int d\tau_{11'} e^{i\omega\tau_{11'}} e^{-i\tau_{11'}\omega_1} e^{-i\tau_{11'}\omega_2} \right) \\ &= \frac{1}{2(2\pi)} \int d\omega_1 G(\mathbf{x}_1 \mathbf{x}_{1'}; \omega_1) G(\mathbf{x}_2 \mathbf{x}_{2'}; -\nu) \left( \int d\tau_{1'2'} e^{i\nu'\tau_{2'1'}} e^{i\tau_{2'1'}\omega_2} \right) \left( \int d\tau_{11'} e^{i\omega\tau_{11'}} e^{-i\tau_{11'}\omega_1} e^{i\tau_{11'}\nu} \right) \\ &= \frac{2\pi}{2} G(\mathbf{x}_1 \mathbf{x}_{1'}; \omega + \nu) G(\mathbf{x}_2 \mathbf{x}_{2'}; -\nu) \delta(\nu - \nu'), \end{aligned} \quad (60)$$

while the Fourier transform of the second term reads

$$\begin{aligned} & K_0^{\text{II}}(\mathbf{x}_1 \mathbf{x}_2; \mathbf{x}_1' \mathbf{x}_2'; \nu, \nu', \omega) = \\ & \frac{1}{2} \int d(\tau_{12} \tau_{2'1'} \tau_{11'}) e^{i\nu\tau_{12} + i\nu'\tau_{2'1'} + i\omega\tau_{11'}} \\ &\quad \times \left( \frac{1}{2\pi} \int d\omega_1 e^{-i(\tau_{11'} - \tau_{2'1'})\omega_1} G(\mathbf{x}_1 \mathbf{x}_{2'}; \omega_1) \right) \left( \frac{1}{2\pi} \int d\omega_2 e^{-i(-\tau_{12} + \tau_{11'})\omega_2} G(\mathbf{x}_2 \mathbf{x}_{1'}; \omega_2) \right) \\ &= \frac{1}{2(2\pi)^2} \int d(\omega_1 \omega_2) G(\mathbf{x}_1 \mathbf{x}_{2'}; \omega_1) G(\mathbf{x}_2 \mathbf{x}_{1'}; \omega_2) \\ &\quad \times \left( \int d\tau_{12} e^{i\nu\tau_{12}} e^{i\tau_{12}\omega_2} \right) \left( \int d\tau_{2'1'} e^{i\nu'\tau_{2'1'}} e^{i\tau_{2'1'}\omega_1} \right) \left( \int d\tau_{11'} e^{i\omega\tau_{11'}} e^{-i\tau_{11'}\omega_1} e^{-i\tau_{11'}\omega_2} \right) \\ &= \frac{1}{2(2\pi)} \int d\omega_1 G(\mathbf{x}_1 \mathbf{x}_{2'}; \omega_1) G(\mathbf{x}_2 \mathbf{x}_{1'}; -\nu) \left( \int d\tau_{2'1'} e^{i\nu'\tau_{2'1'}} e^{i\tau_{2'1'}\omega_1} \right) \left( \int d\tau_{11'} e^{i\omega\tau_{11'}} e^{-i\tau_{11'}\omega_1} e^{i\tau_{11'}\nu} \right) \\ &= \frac{2\pi}{2} G(\mathbf{x}_1 \mathbf{x}_{2'}; \omega + \nu) G(\mathbf{x}_2 \mathbf{x}_{1'}; -\nu) \delta(\nu + \omega + \nu'). \end{aligned} \quad (61)$$

The single-frequency propagator is obtained by integrating out the two fermionic frequencies

$$K_0(\mathbf{x}_1\mathbf{x}_2; \mathbf{x}_1'\mathbf{x}_2'; \omega) = \frac{1}{4\pi} \int d\nu [G(\mathbf{x}_1\mathbf{x}_1'; \omega + \nu)G(\mathbf{x}_2\mathbf{x}_2'; -\nu) - G(\mathbf{x}_1\mathbf{x}_2'; \omega + \nu)G(\mathbf{x}_2\mathbf{x}_1'; -\nu)]. \quad (62)$$

The first term is computed as

$$\begin{aligned} K_0^I(\omega) &= \frac{1}{4\pi} \int d\nu G(\mathbf{x}_1\mathbf{x}_1'; \omega + \nu)G(\mathbf{x}_2\mathbf{x}_2'; -\nu) \\ &= \frac{1}{4\pi} \int d\nu \left( \sum_i \frac{\varphi_i(\mathbf{x}_1)\varphi_i^*(\mathbf{x}_1')}{\nu - (-\omega + \epsilon_i + i\eta)} + \sum_a \frac{\varphi_a(\mathbf{x}_1)\varphi_a^*(\mathbf{x}_1')}{\nu - (-\omega + \epsilon_a - i\eta)} \right) \left( -\sum_j \frac{\varphi_j(\mathbf{x}_2)\varphi_j^*(\mathbf{x}_2')}{\nu - (-\epsilon_j - i\eta)} - \sum_b \frac{\varphi_b(\mathbf{x}_2)\varphi_b^*(\mathbf{x}_2')}{\nu - (-\epsilon_b + i\eta)} \right) \\ &= -\frac{1}{4\pi} \int d\omega' \sum_{ij} \frac{\varphi_i(\mathbf{x}_1)\varphi_i^*(\mathbf{x}_1')}{\nu - (-\omega + \epsilon_i + i\eta)} \frac{\varphi_j(\mathbf{x}_2)\varphi_j^*(\mathbf{x}_2')}{\nu - (-\epsilon_j - i\eta)} - \frac{1}{4\pi} \int d\omega' \sum_{ab} \frac{\varphi_a(\mathbf{x}_1)\varphi_a^*(\mathbf{x}_1')}{\nu - (-\omega + \epsilon_a - i\eta)} \frac{\varphi_b(\mathbf{x}_2)\varphi_b^*(\mathbf{x}_2')}{\nu - (-\epsilon_b + i\eta)} \\ &= -\frac{2\pi i}{4\pi} \sum_{ij} \frac{\varphi_i(\mathbf{x}_1)\varphi_i^*(\mathbf{x}_1')\varphi_j(\mathbf{x}_2)\varphi_j^*(\mathbf{x}_2')}{(-\omega + \epsilon_i + i\eta) - (-\epsilon_j - i\eta)} - \frac{2\pi i}{4\pi} \sum_{ab} \frac{\varphi_a(\mathbf{x}_1)\varphi_a^*(\mathbf{x}_1')\varphi_b(\mathbf{x}_2)\varphi_b^*(\mathbf{x}_2')}{(-\epsilon_b + i\eta) - (-\omega + \epsilon_a - i\eta)} \\ &= \frac{i}{2} \sum_{ij} \frac{\varphi_i(\mathbf{x}_1)\varphi_i^*(\mathbf{x}_1')\varphi_j(\mathbf{x}_2)\varphi_j^*(\mathbf{x}_2')}{\omega - (\epsilon_i + \epsilon_j + 2i\eta)} - \frac{i}{2} \sum_{ab} \frac{\varphi_a(\mathbf{x}_1)\varphi_a^*(\mathbf{x}_1')\varphi_b(\mathbf{x}_2)\varphi_b^*(\mathbf{x}_2')}{\omega - (\epsilon_a + \epsilon_b - 2i\eta)}, \end{aligned} \quad (63)$$

and, once projected in the finite basis set, reads

$$(K_0^I)_{pqrs}(\omega) = \frac{i}{2} \left( \sum_{ij} \frac{\delta_{pi}\delta_{qj}\delta_{ri}\delta_{sj}}{\omega - (\epsilon_j + \epsilon_i + 2i\eta)} - \sum_{ab} \frac{\delta_{pa}\delta_{qb}\delta_{ra}\delta_{sb}}{\omega - (\epsilon_a + \epsilon_b - 2i\eta)} \right). \quad (64)$$

The second term is computed similarly

$$K_0^{II}(\omega) = \frac{i}{2} \sum_{ij} \frac{\varphi_i(\mathbf{x}_1)\varphi_i^*(\mathbf{x}_2')\varphi_j(\mathbf{x}_2)\varphi_j^*(\mathbf{x}_1')}{\omega - (\epsilon_i + \epsilon_j + 2i\eta)} - \frac{i}{2} \sum_{ab} \frac{\varphi_a(\mathbf{x}_1)\varphi_a^*(\mathbf{x}_2')\varphi_b(\mathbf{x}_2)\varphi_b^*(\mathbf{x}_1')}{\omega - (\epsilon_a + \epsilon_b - 2i\eta)}, \quad (65)$$

and, once projected in the finite basis set, reads

$$(K_0^{II})_{pqrs}(\omega) = \frac{i}{2} \left( -\sum_{ij} \frac{\delta_{qi}\delta_{pj}\delta_{ri}\delta_{sj}}{\omega - (\epsilon_j + \epsilon_i + 2i\eta)} + \sum_{ab} \frac{\delta_{qa}\delta_{pb}\delta_{ra}\delta_{sb}}{\omega - (\epsilon_a + \epsilon_b - 2i\eta)} \right). \quad (66)$$

These two expressions are gathered to form the tensor elements of  $K_0$

$$\begin{aligned} (K_0)_{pqrs}(\omega) &= (K_0^I)_{pqrs}(\omega) + (K_0^{II})_{pqrs}(\omega) \\ &= \frac{i}{2} \left( \sum_{ij} \frac{\delta_{qj}\delta_{pi}\delta_{ri}\delta_{sj}}{\omega - (\epsilon_j + \epsilon_i + 2i\eta)} - \sum_{ab} \frac{\delta_{qb}\delta_{pa}\delta_{ra}\delta_{sb}}{\omega - (\epsilon_a + \epsilon_b - 2i\eta)} \right) \\ &\quad - \frac{i}{2} \left( \sum_{ij} \frac{\delta_{pj}\delta_{qi}\delta_{ri}\delta_{sj}}{\omega - (\epsilon_j + \epsilon_i + 2i\eta)} - \sum_{ab} \frac{\delta_{pb}\delta_{qa}\delta_{ra}\delta_{sb}}{\omega - (\epsilon_a + \epsilon_b - 2i\eta)} \right). \end{aligned} \quad (67)$$

Therefore,  $K_0$  has the following antisymmetric properties  $(K_0)_{pqrs} = -(K_0)_{qprs} = -(K_0)_{pqsr} = (K_0)_{qpsr}$ , which can be used to reduce the size of the space that one must consider (see below).

### C. Spin-orbital expression

Once projected in a basis set, the pp-BSE reads

$$K_{pqrs}(\omega) = (K_0)_{pqrs}(\omega) + \frac{1}{2}(K_0)_{pqtu}(\omega)\tilde{\Gamma}_{tuvw}^{\text{pp}}(\omega)K_{vwrs}(\omega), \quad (68)$$

but it cannot be inverted yet. To do so one must first recast the two-electron basis set  $\{\varphi_p(\mathbf{x}_1)\varphi_q(\mathbf{x}_2)\}_{\{p,q\}\in[1,K]^2}$  (where  $K$  is the size of the basis set) as

$$\left\{ \frac{\varphi_p(\mathbf{x}_1)\varphi_q(\mathbf{x}_2) - \varphi_q(\mathbf{x}_1)\varphi_p(\mathbf{x}_2)}{\sqrt{2}} \right\}_{p < q, q \in [1, K]} \cup \left\{ \varphi_p(\mathbf{x}_1)\varphi_p(\mathbf{x}_2) \right\}_{p \in [1, K]} \cup \left\{ \frac{\varphi_p(\mathbf{x}_1)\varphi_q(\mathbf{x}_2) + \varphi_q(\mathbf{x}_1)\varphi_p(\mathbf{x}_2)}{\sqrt{2}} \right\}_{p < q, q \in [1, K]}. \quad (69)$$

In other words, the basis set is decomposed into its antisymmetric and symmetric parts. Because of their antisymmetric nature,  $K$ ,  $K_0$  and  $\tilde{\Gamma}^{\text{pp}}$  are non-zero only in the first subset. We denote the matrix elements in the antisymmetric (resp. symmetric) basis set as  $K_{\overline{pqrs}}$  (resp.  $K_{\overline{pqrs}}$ ). Note that, in this subset, we have  $p < q$  and  $r < s$  (resp.  $p \leq q$  and  $r \leq s$ ). Hence, due to these restrictions on  $p$ ,  $q$ ,  $r$ , and  $s$ , only the second term in Eq. (67) is non-zero, and the matrix elements in the antisymmetric basis are

$$(K_0)_{\overline{pqrs}}(\omega) = i \sum_{i < j} \frac{\delta_{ri}\delta_{sj}\delta_{pi}\delta_{qj}}{\omega - (\epsilon_i + \epsilon_j + 2i\eta)} - i \sum_{a < b} \frac{\delta_{ra}\delta_{sb}\delta_{pa}\delta_{qb}}{\omega - (\epsilon_a + \epsilon_b - 2i\eta)}, \quad (70)$$

and, for the kernel, we have  $\Gamma_{\overline{pqrs}}^{\text{pp}}(\omega) = 2\tilde{\Gamma}_{\overline{pqrs}}^{\text{pp}}(\omega)$ . In the antisymmetric basis, the BSE can be inverted and reads

$$(K)^{-1}_{\overline{pqrs}}(\omega) = (K_0)^{-1}_{\overline{pqrs}}(\omega) + \frac{1}{2}\tilde{\Gamma}_{\overline{pqrs}}^{\text{pp}}(\omega). \quad (71)$$

The independent-particle propagator tensor can be transformed into a diagonal matrix by defining composite indices  $\mathbf{K}_0 = (K_0)_{pq,rs}$

$$\begin{aligned} (\mathbf{K}_0)^{-1} &= \begin{pmatrix} (K_0)_{ab,ab} & \mathbf{0} \\ \mathbf{0} & (K_0)_{ij,ij} \end{pmatrix}^{-1} = \begin{pmatrix} i \text{diag}[\omega - (\epsilon_a + \epsilon_b)] & \mathbf{0} \\ \mathbf{0} & i \text{diag}[(\epsilon_i + \epsilon_j) - \omega] \end{pmatrix} \\ &= i \begin{pmatrix} \omega & \mathbf{0} \\ \mathbf{0} & -\omega \end{pmatrix} + i \begin{pmatrix} -\epsilon_{ab} & \mathbf{0} \\ \mathbf{0} & \epsilon_{ij} \end{pmatrix}, \end{aligned} \quad (72)$$

where  $\epsilon_{ij} = \text{diag}(\epsilon_i + \epsilon_j)$  and  $\epsilon_{ab} = \text{diag}(\epsilon_a + \epsilon_b)$ . Hence, the BSE can be written as

$$\mathbf{K}^{-1}(\omega) = \mathbf{K}_0^{-1}(\omega) + \frac{1}{2}\tilde{\Gamma}^{\text{pp}}(\omega) = i \left[ \begin{pmatrix} \omega & \mathbf{0} \\ \mathbf{0} & -\omega \end{pmatrix} - \begin{pmatrix} \epsilon_{ab} & \mathbf{0} \\ \mathbf{0} & -\epsilon_{ij} \end{pmatrix} - \frac{i}{2}\tilde{\Gamma}^{\text{pp}}(\omega) \right] = i\mathcal{M} \cdot [\omega\mathbf{1} - \mathcal{H}^{\text{pp}}(\omega)], \quad (73)$$

with an effective Hamiltonian matrix  $\mathcal{H}^{\text{pp}}(\omega)$  defined as

$$\mathcal{H}^{\text{pp}}(\omega) = \begin{pmatrix} \mathbf{C}^{\text{pp}}(\omega) & \mathbf{B}^{\text{pp}} \\ -(\mathbf{B}^{\text{pp}})^\dagger & -\mathbf{D}^{\text{pp}}(\omega) \end{pmatrix}, \quad (74)$$

in terms of the blocks given by

$$\mathbf{C}_{ab,cd}^{\text{pp}}(\omega) = (\epsilon_a + \epsilon_b)\delta_{ac}\delta_{bd} + i\tilde{\Gamma}_{abcd}^{\text{pp}}(\omega), \quad (75a)$$

$$\mathbf{B}_{ab,ij}^{\text{pp}} = +i\tilde{\Gamma}_{abij}^{\text{pp}}, \quad (75b)$$

$$\mathbf{D}_{ij,kl}^{\text{pp}}(\omega) = -(\epsilon_i + \epsilon_j)\delta_{ik}\delta_{jl} + i\tilde{\Gamma}_{ijkl}^{\text{pp}}(\omega). \quad (75c)$$

In this case, the eigenvectors are

$$\mathcal{L}^{\text{pp}} = \begin{pmatrix} \mathbf{X}^{\text{ee}} & -\mathbf{Y}^{\text{hh}} \\ -\mathbf{Y}^{\text{ee}} & \mathbf{X}^{\text{hh}} \end{pmatrix}, \quad \mathcal{R}^{\text{pp}} = \begin{pmatrix} \mathbf{X}^{\text{ee}} & \mathbf{Y}^{\text{hh}} \\ \mathbf{Y}^{\text{ee}} & \mathbf{X}^{\text{hh}} \end{pmatrix}, \quad (76)$$

and the eigenvalue matrix is

$$\mathcal{E}^{\text{pp}} = \begin{pmatrix} \Omega^{\text{ee}} & \mathbf{0} \\ \mathbf{0} & -\Omega^{\text{hh}} \end{pmatrix}. \quad (77)$$

The inverse propagator can be written as

$$\mathbf{K}^{-1}(\omega) = i\mathcal{M} \cdot (\mathcal{L}^{\text{pp}})^\dagger \cdot [\omega\mathbf{1} - \mathcal{E}^{\text{pp}}] \cdot \mathcal{R}^{\text{pp}}, \quad (78)$$

and then inverted

$$\mathbf{K}(\omega) = -i\mathcal{R}^{\text{pp}} \cdot [\omega\mathbf{1} - \mathcal{E}^{\text{pp}}]^{-1} \cdot (\mathcal{L}^{\text{pp}})^\dagger \cdot \mathcal{M}. \quad (79)$$

In terms of the eigenvectors and eigenvalues, the pp propagator is written

$$\mathbf{K}(\omega) = -i \begin{pmatrix} \mathbf{K}_1(\omega) & \mathbf{K}_2(\omega) \\ \mathbf{K}_3(\omega) & \mathbf{K}_4(\omega) \end{pmatrix}, \quad (80)$$

with

$$\mathbf{K}_1(\omega) = \mathbf{X}^{\text{ee}} \cdot [\omega\mathbf{1} - \mathbf{\Omega}^{\text{ee}}]^{-1} \cdot (\mathbf{X}^{\text{ee}})^\dagger - \mathbf{Y}^{\text{hh}} \cdot [\omega\mathbf{1} - \mathbf{\Omega}^{\text{hh}}]^{-1} \cdot (\mathbf{Y}^{\text{hh}})^\dagger, \quad (81a)$$

$$\mathbf{K}_2(\omega) = \mathbf{X}^{\text{ee}} \cdot [\omega\mathbf{1} - \mathbf{\Omega}^{\text{ee}}]^{-1} \cdot (\mathbf{Y}^{\text{ee}})^\dagger - \mathbf{Y}^{\text{hh}} \cdot [\omega\mathbf{1} - \mathbf{\Omega}^{\text{hh}}]^{-1} \cdot (\mathbf{X}^{\text{hh}})^\dagger, \quad (81b)$$

$$\mathbf{K}_3(\omega) = \mathbf{Y}^{\text{ee}} \cdot [\omega\mathbf{1} - \mathbf{\Omega}^{\text{ee}}]^{-1} \cdot (\mathbf{X}^{\text{ee}})^\dagger - \mathbf{X}^{\text{hh}} \cdot [\omega\mathbf{1} - \mathbf{\Omega}^{\text{hh}}]^{-1} \cdot (\mathbf{Y}^{\text{hh}})^\dagger, \quad (81c)$$

$$\mathbf{K}_4(\omega) = \mathbf{Y}^{\text{ee}} \cdot [\omega\mathbf{1} - \mathbf{\Omega}^{\text{ee}}]^{-1} \cdot (\mathbf{Y}^{\text{ee}})^\dagger - \mathbf{X}^{\text{hh}} \cdot [\omega\mathbf{1} - \mathbf{\Omega}^{\text{hh}}]^{-1} \cdot (\mathbf{X}^{\text{hh}})^\dagger, \quad (81d)$$

or alternatively

$$K_{\overline{pq}, \overline{rs}}(\omega) = -i \sum_m \left[ \frac{\rho_{pq,m}^{\text{ee}} \rho_{rs,m}^{\text{ee},*}}{\omega - (\Omega_m^{\text{ee}} - i\eta)} - \frac{\rho_{pq,m}^{\text{hh},*} \rho_{rs,m}^{\text{hh}}}{\omega - (\Omega_m^{\text{hh}} + i\eta)} \right], \quad (82)$$

where

$$\rho_{pq,m}^{\text{ee}} = \sum_{a < b} X_{ab,m}^{\text{ee}} \delta_{pa} \delta_{qb} + \sum_{i < j} Y_{ij,m}^{\text{ee}} \delta_{pi} \delta_{qj}, \quad (83a)$$

$$\rho_{pq,m}^{\text{hh}} = \sum_{i < j} X_{ij,m}^{\text{hh}} \delta_{pi} \delta_{qj} + \sum_{a < b} Y_{ab,m}^{\text{hh}} \delta_{pa} \delta_{qb}. \quad (83b)$$

#### D. Spin adaptation

The pp-BSE for the three different spin combination reads

$$K(1_\uparrow 2_\uparrow; 1'_\uparrow 2'_\uparrow) = K_0(1_\uparrow 2_\uparrow; 1'_\uparrow 2'_\uparrow) - \frac{1}{2} \sum_{\substack{\sigma_3 \sigma_4 \\ \sigma_{3'} \sigma_{4'}}} G(1_\uparrow 3_{\sigma_3}) G(2_\uparrow 3'_{\sigma_{3'}}) \Gamma^{\text{pp}}(3_{\sigma_3} 3'_{\sigma_{3'}}; 4_{\sigma_4} 4'_{\sigma_{4'}}) K(4_{\sigma_4} 4'_{\sigma_{4'}}; 1'_\uparrow 2'_\uparrow), \quad (84a)$$

$$K(1_\uparrow 2_\downarrow; 1'_\uparrow 2'_\downarrow) = K_0(1_\uparrow 2_\downarrow; 1'_\uparrow 2'_\downarrow) - \frac{1}{2} \sum_{\substack{\sigma_3 \sigma_4 \\ \sigma_{3'} \sigma_{4'}}} G(1_\uparrow 3_{\sigma_3}) G(2_\downarrow 3'_{\sigma_{3'}}) \Gamma^{\text{pp}}(3_{\sigma_3} 3'_{\sigma_{3'}}; 4_{\sigma_4} 4'_{\sigma_{4'}}) K(4_{\sigma_4} 4'_{\sigma_{4'}}; 1'_\uparrow 2'_\downarrow), \quad (84b)$$

$$K(1_\uparrow 2_\downarrow; 1'_\downarrow 2'_\uparrow) = K_0(1_\uparrow 2_\downarrow; 1'_\downarrow 2'_\uparrow) - \frac{1}{2} \sum_{\substack{\sigma_3 \sigma_4 \\ \sigma_{3'} \sigma_{4'}}} G(1_\uparrow 3_{\sigma_3}) G(2_\downarrow 3'_{\sigma_{3'}}) \Gamma^{\text{pp}}(3_{\sigma_3} 3'_{\sigma_{3'}}; 4_{\sigma_4} 4'_{\sigma_{4'}}) K(4_{\sigma_4} 4'_{\sigma_{4'}}; 1'_\downarrow 2'_\uparrow), \quad (84c)$$

where we have used the antisymmetry of  $\Gamma^{\text{pp}}$  to simplify one of the term of  $K_0$ . The spin independence of  $G$  can be used to simplify these sums

$$K(1_\uparrow 2_\uparrow; 1'_\uparrow 2'_\uparrow) = K_0(1_\uparrow 2_\uparrow; 1'_\uparrow 2'_\uparrow) - \frac{1}{2} \sum_{\sigma_{3'} \sigma_{4'}} G(1_\uparrow 3_\uparrow) G(2_\uparrow 3'_\uparrow) \Gamma^{\text{pp}}(3_\uparrow 3'_\uparrow; 4_{\sigma_4} 4'_{\sigma_{4'}}) K(4_{\sigma_4} 4'_{\sigma_{4'}}; 3_\uparrow 4_\uparrow), \quad (85a)$$

$$K(1_\uparrow 2_\downarrow; 1'_\uparrow 2'_\downarrow) = \frac{1}{2} G(1_\uparrow 1'_\uparrow) G(2_\downarrow 2'_\downarrow) - \frac{1}{2} \sum_{\sigma_{3'} \sigma_{4'}} G(1_\uparrow 3_\uparrow) G(2_\downarrow 3'_\downarrow) \Gamma^{\text{pp}}(3_\uparrow 3'_\downarrow; 4_{\sigma_4} 4'_{\sigma_{4'}}) K(4_{\sigma_4} 4'_{\sigma_{4'}}; 1'_\uparrow 2'_\downarrow), \quad (85b)$$

$$K(1_\uparrow 2_\downarrow; 1'_\downarrow 2'_\uparrow) = -\frac{1}{2} G(1_\uparrow 2'_\uparrow) G(2_\downarrow 1'_\downarrow) - \frac{1}{2} \sum_{\sigma_{3'} \sigma_{4'}} G(1_\uparrow 3_\uparrow) G(2_\downarrow 3'_\downarrow) \Gamma^{\text{pp}}(3_\uparrow 3'_\downarrow; 4_{\sigma_4} 4'_{\sigma_{4'}}) K(4_{\sigma_4} 4'_{\sigma_{4'}}; 1'_\downarrow 2'_\uparrow). \quad (85c)$$

They can be further simplified by considering only the non-zero spin combinations for two-body quantities

$$K(1\uparrow 2\uparrow; 1'\uparrow 2'\uparrow) = K_0(\mathbf{r}t_1\mathbf{r}t_2; \mathbf{r}t_1'\mathbf{r}t_2') - \frac{1}{2}G(\mathbf{r}t_1\mathbf{r}t_3)G(\mathbf{r}t_2\mathbf{r}t_{3'})\Gamma^{\text{pp}}(3\uparrow 3'\downarrow; 4\uparrow 4'\downarrow)K(4\uparrow 4'; 1'\uparrow 2'\uparrow), \quad (86a)$$

$$K(1\uparrow 2\downarrow; 1'\uparrow 2'\downarrow) = \frac{1}{2}G(\mathbf{r}t_1\mathbf{r}t_{1'})G(\mathbf{r}t_2\mathbf{r}t_{2'}) - \frac{1}{2}G(\mathbf{r}t_1\mathbf{r}t_3)G(\mathbf{r}t_2\mathbf{r}t_{3'}) \left[ \Gamma^{\text{pp}}(3\uparrow 3'\downarrow; 4\uparrow 4'\downarrow)K(4\uparrow 4'; 1'\uparrow 2'\downarrow) + \Gamma^{\text{pp}}(3\uparrow 3'\downarrow; 4\downarrow 4'\uparrow)K(4\downarrow 4'; 1'\uparrow 2'\downarrow) \right], \quad (86b)$$

$$K(1\uparrow 2\downarrow; 1'\downarrow 2'\uparrow) = -\frac{1}{2}G(\mathbf{r}t_1\mathbf{r}t_{2'})G(\mathbf{r}t_2\mathbf{r}t_{1'}) - \frac{1}{2}G(\mathbf{r}t_1\mathbf{r}t_3)G(\mathbf{r}t_2\mathbf{r}t_{3'}) \left[ \Gamma^{\text{pp}}(3\uparrow 3'\downarrow; 4\uparrow 4'\downarrow)K(4\uparrow 4'; 1'\downarrow 2'\uparrow) + \Gamma^{\text{pp}}(3\uparrow 3'\downarrow; 4\downarrow 4'\uparrow)K(4\downarrow 4'; 1'\downarrow 2'\uparrow) \right]. \quad (86c)$$

For a pp propagator, the two incoming particles are labeled with indices 1' and 2', while the outgoing particles are labeled 1 and 2. Hence,  $K(1\uparrow 2\uparrow; 1'\uparrow 2'\uparrow)$  corresponds to the propagation of a  $S_z = 1$  triplet pair of electrons and is already spin-adapted. The  $S_z = 0$  pairs of electrons, with spin  $\uparrow\downarrow$  or  $\downarrow\uparrow$ , are not eigenfunctions of the spin operator  $\hat{S}^2$ . As a consequence, in this basis,  $\Gamma^{\text{pp}}(1\uparrow 2\downarrow; 1'\uparrow 2'\downarrow)$  and  $\Gamma^{\text{pp}}(1\uparrow 2\downarrow; 1'\downarrow 2'\uparrow)$  are coupled. These two propagators can be spin-adapted by introducing the singlet and triplet propagators

$$K^s(\mathbf{r}t_1\mathbf{r}t_2; \mathbf{r}t_1'\mathbf{r}t_2') = K(1\uparrow 2\downarrow; 1'\uparrow 2'\downarrow) - K(1\uparrow 2\downarrow; 1'\downarrow 2'\uparrow), \quad (87a)$$

$$K^t(\mathbf{r}t_1\mathbf{r}t_2; \mathbf{r}t_1'\mathbf{r}t_2') = K(1\uparrow 2\downarrow; 1'\uparrow 2'\downarrow) + K(1\uparrow 2\downarrow; 1'\downarrow 2'\uparrow) = K(1\uparrow 2\uparrow; 1'\uparrow 2'\uparrow), \quad (87b)$$

which correspond to propagation of  $S_z = 0$  pairs of electrons with total spin  $S = 0$  for the singlet and  $S = 1$  for the triplet. In terms of these spin-adapted vertices, the last two pp-BSEs in Eqs. (86) become

$$K^s(\mathbf{r}t_1\mathbf{r}t_2; \mathbf{r}t_1'\mathbf{r}t_2') = \bar{K}_0(\mathbf{r}t_1\mathbf{r}t_2; \mathbf{r}t_1'\mathbf{r}t_2') - \frac{1}{2}\bar{K}_0(\mathbf{r}t_1\mathbf{r}t_2; \mathbf{r}t_3\mathbf{r}t_{3'})\Gamma^s(\mathbf{r}t_3\mathbf{r}t_{3'}; \mathbf{r}t_4\mathbf{r}t_{4'})K^s(\mathbf{r}t_4\mathbf{r}t_{4'}; \mathbf{r}t_1'\mathbf{r}t_2'), \quad (88a)$$

$$K^t(\mathbf{r}t_1\mathbf{r}t_2; \mathbf{r}t_1'\mathbf{r}t_2') = K_0(\mathbf{r}t_1\mathbf{r}t_2; \mathbf{r}t_1'\mathbf{r}t_2') - \frac{1}{2}K_0(\mathbf{r}t_1\mathbf{r}t_2; \mathbf{r}t_3\mathbf{r}t_{3'})\Gamma^t(\mathbf{r}t_3\mathbf{r}t_{3'}; \mathbf{r}t_4\mathbf{r}t_{4'})K^t(\mathbf{r}t_4\mathbf{r}t_{4'}; \mathbf{r}t_1'\mathbf{r}t_2'), \quad (88b)$$

where we have introduced

$$\bar{K}_0 = \frac{1}{2}[G(11')G(22') + G(12')G(21')]. \quad (89)$$

These two spin-adapted propagators are referred to as the singlet  $K^s$  and triplet  $K^t$  propagators, respectively.

## E. Spatial-orbital expression

The BSE for the triplet pp propagator can be solved in the exact same way as the BSE for the full pp-BSE, but in a spatial orbital basis rather than in a spin-orbital basis. Hence, solving the triplet channel BSE is equivalent to diagonalizing an effective Hamiltonian matrix  $\mathcal{H}^t(\omega)$  defined as

$$\mathcal{H}^t(\omega) = \begin{pmatrix} C^t(\omega) & B^t \\ -(B^t)^\dagger & -D^t(\omega) \end{pmatrix}, \quad (90)$$

in terms of

$$C_{ab,cd}^t(\omega) = (\epsilon_a + \epsilon_b)\delta_{ac}\delta_{bd} + i\tilde{\Gamma}_{abcd}^t(\omega), \quad (91a)$$

$$B_{ab,ij}^t = +i\tilde{\Gamma}_{abij}^t, \quad (91b)$$

$$D_{ij,kl}^t(\omega) = -(\epsilon_i + \epsilon_j)\delta_{ik}\delta_{jl} + i\tilde{\Gamma}_{ijkl}^t(\omega), \quad (91c)$$

where  $p < q$  in each spatial orbital composite indices  $pq$  and the tensor elements of the kernel are given by

$$\tilde{\Gamma}_{pqrs}^t(\omega) = \tilde{\Gamma}_{p\uparrow q\uparrow r\uparrow s\uparrow}^{\text{pp}}(\omega). \quad (92)$$

The procedure to solve the BSE for the singlet pp propagator has to be slightly adapted because  $\bar{K}_0$  and  $\tilde{\Gamma}_s^{\text{pp}}$  are now symmetric. The Fourier transform is the same, but now the BSE is non-zero only in the symmetric subsets of Eq. (69). This yield an effective Hamiltonian matrix  $\mathcal{H}_s^{\text{pp}}(\omega)$  to diagonalize given by

$$\mathcal{H}^s(\omega) = \begin{pmatrix} \mathbf{C}^s(\omega) & \mathbf{B}^s \\ -(\mathbf{B}^s)^\dagger & -\mathbf{D}^s(\omega) \end{pmatrix}, \quad (93)$$

in terms of

$$C_{ab,cd}^s(\omega) = (\epsilon_a + \epsilon_b)\delta_{ac}\delta_{bd} + i\tilde{\Gamma}_{abcd}^s(\omega), \quad (94a)$$

$$B_{ab,ij}^s = +i\tilde{\Gamma}_{abij}^s, \quad (94b)$$

$$D_{ij,kl}^s(\omega) = -(\epsilon_i + \epsilon_j)\delta_{ik}\delta_{jl} + i\tilde{\Gamma}_{ijkl}^s(\omega), \quad (94c)$$

where  $p \leq q$  in each composite indices  $pq$  and the tensor elements of the kernel are given by

$$\tilde{\Gamma}_{pqrs}^s(\omega) = \frac{1}{\sqrt{1 + \delta_{pq}}\sqrt{1 + \delta_{rs}}} \left[ \tilde{\Gamma}_{p\uparrow q\downarrow r\uparrow s\downarrow}^{\text{pp}}(\omega) - \tilde{\Gamma}_{p\uparrow q\downarrow r\downarrow s\uparrow}^{\text{pp}}(\omega) \right]. \quad (95)$$

#### IV. FOURIER TRANSFORM

The aim of this section is to obtain the set of parquet equations in frequency space. The Fourier transform of the Dyson equation is well-known, while the parquet decomposition of  $F$  in frequency space is simply given by the definitions of the three-time Fourier transform (see Sec. I). Hence, only the BSEs and the self-energy have to be Fourier transformed.

##### A. Bethe-Salpeter equations

The Fourier-transformed BSEs for the two-body propagators have already been discussed in the previous Sections. Hence, the frequency-space form of the BSEs for the full two-body vertex can be easily deduced and read

$$F(\mathbf{x}_1\mathbf{x}_2; \mathbf{x}_3\mathbf{x}_4; \nu, \nu', \omega) = \Gamma^{\text{eh}}(\mathbf{x}_1\mathbf{x}_2; \mathbf{x}_3\mathbf{x}_4; \nu, \nu', \omega) + \int \frac{d(\nu_1\nu_2)}{(2\pi)^2} \Gamma^{\text{eh}}(\mathbf{x}_1\mathbf{x}_{3'}; \mathbf{x}_3\mathbf{x}_{1'}; \nu, \nu_1, \omega) L(\mathbf{x}_1'\mathbf{x}_{2'}; \mathbf{x}_{3'}\mathbf{x}_{4'}; \nu_1, \nu_2, \omega) \Gamma^{\text{eh}}(\mathbf{x}_4'\mathbf{x}_2; \mathbf{x}_{2'}\mathbf{x}_4; \nu_2, \nu', \omega), \quad (96)$$

and

$$F_P(\mathbf{x}_1\mathbf{x}_2; \mathbf{x}_3\mathbf{x}_4; \nu, \nu', \omega) = \Gamma_P^{\text{pp}}(\mathbf{x}_1\mathbf{x}_2; \mathbf{x}_3\mathbf{x}_4; \nu, \nu', \omega) - \int \frac{d(\nu_1\nu_2)}{2(2\pi)^2} \Gamma_P^{\text{pp}}(\mathbf{x}_1\mathbf{x}_2; \mathbf{x}_{1'}\mathbf{x}_{2'}; \nu, \nu_1, \omega) K_P(\mathbf{x}_{1'}\mathbf{x}_{2'}; \mathbf{x}_{3'}\mathbf{x}_{4'}; \nu_1, \nu_2, \omega) \Gamma_P^{\text{pp}}(\mathbf{x}_{3'}\mathbf{x}_{4'}; \mathbf{x}_3\mathbf{x}_4; \nu_2, \nu', \omega). \quad (97)$$

##### B. Self-energy

The Fourier transform of the correlation part of the self-energy is now performed. First, the time-dependence can be simplified thanks to the instantaneous nature of the Coulomb interaction

$$\begin{aligned} \Sigma_c(\mathbf{x}_1\mathbf{x}_{1'}; \tau_{11'}) &= -iv(\mathbf{x}_1\mathbf{x}_2; \mathbf{x}_3\mathbf{x}_{2'}) \int d(t_2t_3t_4t_{2'}t_{3'}t_{4'}) \delta(\tau_{12})\delta(\tau_{13'})\delta(\tau_{22'}) \\ &\quad \times G(\mathbf{x}_3'\mathbf{x}_3; \tau_{3'3})G(\mathbf{x}_4'\mathbf{x}_2; \tau_{4'2})G(\mathbf{x}_2'\mathbf{x}_4; \tau_{2'4})F(\mathbf{x}_3\mathbf{x}_4; \mathbf{x}_4'\mathbf{x}_{1'}; \tau_{34'}, \tau_{41'}, \tau_{44'}) \\ &= -iv(\mathbf{x}_1\mathbf{x}_2; \mathbf{x}_3\mathbf{x}_{2'}) \int d(t_2t_3t_4t_{4'}) \delta(\tau_{12})G(\mathbf{x}_3'\mathbf{x}_3; \tau_{13})G(\mathbf{x}_4'\mathbf{x}_2; \tau_{4'2})G(\mathbf{x}_2'\mathbf{x}_4; \tau_{24})F(\mathbf{x}_3\mathbf{x}_4; \mathbf{x}_4'\mathbf{x}_{1'}; \tau_{34'}, \tau_{41'}, \tau_{44'}) \\ &= -iv(\mathbf{x}_1\mathbf{x}_2; \mathbf{x}_3\mathbf{x}_{2'}) \int d(t_3t_4t_{4'}) G(\mathbf{x}_3'\mathbf{x}_3; \tau_{13})G(\mathbf{x}_4'\mathbf{x}_2; \tau_{4'1})G(\mathbf{x}_2'\mathbf{x}_4; \tau_{14})F(\mathbf{x}_3\mathbf{x}_4; \mathbf{x}_4'\mathbf{x}_{1'}; \tau_{34'}, \tau_{41'}, \tau_{44'}). \end{aligned} \quad (98)$$

The self-energy is transformed to frequency space as

$$\begin{aligned}
& \Sigma_c(\mathbf{x}_1\mathbf{x}_{1'}; \omega) \\
&= -iv(\mathbf{x}_1\mathbf{x}_2; \mathbf{x}_3'\mathbf{x}_{2'}) \int d\tau_{11'} e^{i\omega\tau_{11'}} \\
&\quad \times \int d(t_3t_4t_{4'}) G(\mathbf{x}_3'\mathbf{x}_3; \tau_{13})G(\mathbf{x}_4'\mathbf{x}_2; \tau_{4'1})G(\mathbf{x}_2'\mathbf{x}_4; \tau_{14})F(\mathbf{x}_3\mathbf{x}_4; \mathbf{x}_4'\mathbf{x}_{1'}; \tau_{34'}, \tau_{41'}, \tau_{44'}) \\
&= \frac{-i}{(2\pi)^6} v(\mathbf{x}_1\mathbf{x}_2; \mathbf{x}_3'\mathbf{x}_{2'}) \int d(\omega_1\omega_2\omega_3\omega_4\omega_5\omega_6) \int d(\tau_{11'}t_3t_4t_{4'}) G(\mathbf{x}_3'\mathbf{x}_3; \omega_1)G(\mathbf{x}_4'\mathbf{x}_2; \omega_2) \\
&\quad \times G(\mathbf{x}_2'\mathbf{x}_4; \omega_3)F(\mathbf{x}_3\mathbf{x}_4; \mathbf{x}_4'\mathbf{x}_{1'}; \omega_4, \omega_5, \omega_6) e^{i\omega\tau_{11'}} e^{-i\omega_1\tau_{13}} e^{-i\omega_2\tau_{4'1}} e^{-i\omega_3\tau_{14}} e^{-i\omega_4\tau_{34'}} e^{-i\omega_5\tau_{41'}} e^{-i\omega_6\tau_{44'}} \\
&= \frac{-i}{(2\pi)^6} v(\mathbf{x}_1\mathbf{x}_2; \mathbf{x}_3'\mathbf{x}_{2'}) \int d(\omega_1\omega_2\omega_3\omega_4\omega_5\omega_6) \int d(\tau_{11'}t_3t_4t_{4'}) G(\mathbf{x}_3'\mathbf{x}_3; \omega_1)G(\mathbf{x}_4'\mathbf{x}_2; \omega_2) \\
&\quad \times G(\mathbf{x}_2'\mathbf{x}_4; \omega_3)F(\mathbf{x}_3\mathbf{x}_4; \mathbf{x}_4'\mathbf{x}_{1'}; \omega_4, \omega_5, \omega_6) e^{i(\omega-\omega_1+\omega_2-\omega_3)\tau_{11'}} e^{i(\omega_1-\omega_4)\tau_{31'}} e^{i(\omega_3-\omega_5-\omega_6)\tau_{41'}} e^{i(\omega_4+\omega_6-\omega_2)\tau_{4'1'}} \\
&= \frac{-i}{(2\pi)^5} v(\mathbf{x}_1\mathbf{x}_2; \mathbf{x}_3'\mathbf{x}_{2'}) \int d(\omega_1\omega_2\omega_3\omega_5\omega_6) \int d(\tau_{11'}t_4t_{4'}) G(\mathbf{x}_3'\mathbf{x}_3; \omega_1)G(\mathbf{x}_4'\mathbf{x}_2; \omega_2) \\
&\quad \times G(\mathbf{x}_2'\mathbf{x}_4; \omega_3)F(\mathbf{x}_3\mathbf{x}_4; \mathbf{x}_4'\mathbf{x}_{1'}; \omega_1, \omega_5, \omega_6) e^{i(\omega-\omega_1+\omega_2-\omega_3)\tau_{11'}} e^{i(\omega_3-\omega_5-\omega_6)\tau_{41'}} e^{i(\omega_1+\omega_6-\omega_2)\tau_{4'1'}} \\
&= \frac{-i}{(2\pi)^4} v(\mathbf{x}_1\mathbf{x}_2; \mathbf{x}_3'\mathbf{x}_{2'}) \int d(\omega_1\omega_2\omega_3\omega_5) \int d(\tau_{11'}t_4) G(\mathbf{x}_3'\mathbf{x}_3; \omega_1)G(\mathbf{x}_4'\mathbf{x}_2; \omega_2) \\
&\quad \times G(\mathbf{x}_2'\mathbf{x}_4; \omega_3)F(\mathbf{x}_3\mathbf{x}_4; \mathbf{x}_4'\mathbf{x}_{1'}; \omega_1, \omega_5, \omega_2 - \omega_1) e^{i(\omega-\omega_1+\omega_2-\omega_3)\tau_{11'}} e^{i(\omega_1-\omega_2+\omega_3-\omega_5)\tau_{41'}} \\
&= \frac{-i}{(2\pi)^3} v(\mathbf{x}_1\mathbf{x}_2; \mathbf{x}_3'\mathbf{x}_{2'}) \int d(\omega_1\omega_2\omega_3) \int d(\tau_{11'}) G(\mathbf{x}_3'\mathbf{x}_3; \omega_1)G(\mathbf{x}_4'\mathbf{x}_2; \omega_2) \\
&\quad \times G(\mathbf{x}_2'\mathbf{x}_4; \omega_3)F(\mathbf{x}_3\mathbf{x}_4; \mathbf{x}_4'\mathbf{x}_{1'}; \omega_1, \omega_1 - \omega_2 + \omega_3, \omega_2 - \omega_1) e^{i(\omega-\omega_1+\omega_2-\omega_3)\tau_{11'}} \\
&= \frac{-i}{(2\pi)^2} v(\mathbf{x}_1\mathbf{x}_2; \mathbf{x}_3'\mathbf{x}_{2'}) \int d(\omega_1\omega_2) G(\mathbf{x}_3'\mathbf{x}_3; \omega_1)G(\mathbf{x}_4'\mathbf{x}_2; \omega_2) \\
&\quad \times G(\mathbf{x}_2'\mathbf{x}_4; \omega - \omega_1 + \omega_2)F(\mathbf{x}_3\mathbf{x}_4; \mathbf{x}_4'\mathbf{x}_{1'}; \omega_1, \omega, \omega_2 - \omega_1).
\end{aligned} \tag{99}$$

This expression can be decomposed into the three components of the self-energy defined in the main text

$$\begin{aligned}
\Sigma^{(2)}(\mathbf{x}_1\mathbf{x}_{1'}; \omega) &= -\frac{1}{2(2\pi)^2} \bar{v}(\mathbf{x}_1\mathbf{x}_2; \mathbf{x}_3'\mathbf{x}_{2'}) \bar{v}(\mathbf{x}_3\mathbf{x}_4; \mathbf{x}_4'\mathbf{x}_{1'}) \\
&\quad \times \int d(\omega_1\omega_2) G(\mathbf{x}_3'\mathbf{x}_3; \omega_1)G(\mathbf{x}_4'\mathbf{x}_2; \omega_2)G(\mathbf{x}_2'\mathbf{x}_4; \omega - \omega_1 + \omega_2),
\end{aligned} \tag{100a}$$

$$\begin{aligned}
\Sigma^{\text{eh}}(\mathbf{x}_1\mathbf{x}_{1'}; \omega) &= -\frac{i}{(2\pi)^2} \bar{v}(\mathbf{x}_1\mathbf{x}_2; \mathbf{x}_3'\mathbf{x}_{2'}) \int d(\omega_1\omega_2) G(\mathbf{x}_3'\mathbf{x}_3; \omega_1)G(\mathbf{x}_4'\mathbf{x}_2; \omega_2) \\
&\quad \times G(\mathbf{x}_2'\mathbf{x}_4; \omega - \omega_1 + \omega_2)\Phi^{\text{eh}}(\mathbf{x}_3\mathbf{x}_4; \mathbf{x}_4'\mathbf{x}_{1'}; \omega_1, \omega, \omega_2 - \omega_1),
\end{aligned} \tag{100b}$$

$$\begin{aligned}
\Sigma^{\text{pp}}(\mathbf{x}_1\mathbf{x}_{1'}; \omega) &= -\frac{i}{2(2\pi)^2} \bar{v}(\mathbf{x}_1\mathbf{x}_2; \mathbf{x}_3'\mathbf{x}_{2'}) \int d(\omega_1\omega_2) G(\mathbf{x}_3'\mathbf{x}_3; \omega_1)G(\mathbf{x}_4'\mathbf{x}_2; \omega_2) \\
&\quad \times G(\mathbf{x}_2'\mathbf{x}_4; \omega - \omega_1 + \omega_2)\Phi_{\text{P}}^{\text{pp}}(\mathbf{x}_3\mathbf{x}_4; \mathbf{x}_4'\mathbf{x}_{1'}; \omega, -\omega_2 + \omega_1 - \omega, \omega_2 + \omega).
\end{aligned} \tag{100c}$$

## V. PROJECTION IN SPIN-ORBITAL BASIS

### A. Link with common BSE kernels

The spin-orbital expressions for the reducible and irreducible vertices have already been reported in the main manuscript. In addition, we provide a discussion on the relation between these expressions and the commonly used BSE kernels.

The expression for the kernel of the eh-BSE given in the main text is

$$i\Gamma_{pqrs}^{\text{eh}} = \langle pq||rs \rangle - i\Phi_{pqsr}^{\text{eh}} + i\Phi_{pqrs}^{\text{pp}}. \tag{101}$$

Hence, the eh eigenvalue problem is

$$A_{ia,jb}^{\text{eh}} = (\epsilon_a - \epsilon_i)\delta_{ab}\delta_{ij} + i\Lambda_{ajib} - i\Phi_{ajbi}^{\text{eh}} + i\Phi_{ajib}^{\text{pp}}, \quad (102a)$$

$$B_{ia,bj}^{\text{eh}} = i\Lambda_{abij} - i\Phi_{abji}^{\text{eh}} + i\Phi_{abij}^{\text{pp}}, \quad (102b)$$

while the effective interaction becomes

$$M_{pq,n}^{\text{eh}} = \sum_{ia} [i\Lambda_{paqi} - i\Phi_{paiq}^{\text{eh}} + i\Phi_{paqi}^{\text{pp}}] X_{ia,n}^{\text{eh}} + \sum_{ai} [i\Lambda_{piqa} - i\Phi_{piaq}^{\text{eh}} + i\Phi_{piqa}^{\text{pp}}] Y_{ai,n}^{\text{eh}}. \quad (103)$$

If  $\Phi^{\text{pp}}$  is set to zero, the kernel of the eigenvalue problem becomes

$$i\Lambda_{ajib} - i\Phi_{ajbi}^{\text{eh}} = \langle aj||ib \rangle + \sum_n \frac{M_{ab,n}^{\text{eh}} M_{ij,n}^{\text{eh},*} + M_{ba,n}^{\text{eh},*} M_{ji,n}^{\text{eh}}}{\Omega_n^{\text{eh}} - i\eta}, \quad (104)$$

and the usual first-order static  $GW$  kernel of the eh-BSE is recovered.<sup>5</sup> Alternatively, one can set  $\Phi^{\text{eh}} = 0$  to get

$$i\Lambda_{ajib} + i\Phi_{ajib}^{\text{pp}} = \langle aj||ib \rangle + \sum_m \left[ -\frac{M_{aj,m}^{\text{ee}} M_{ib,m}^{\text{ee},*}}{\Omega_m^{\text{ee}} - i\eta} + \frac{M_{aj,m}^{\text{hh},*} M_{ib,m}^{\text{hh}}}{\Omega_m^{\text{hh}} + i\eta} \right]. \quad (105)$$

In this case, the kernel is found to be equal to the first-order static pp  $T$ -matrix kernel of the eh-BSE.<sup>6</sup>

As shown in the main text, in a spin-orbital basis set, the pp irreducible kernel is given by

$$i\Gamma_{pqrs}^{\text{pp}} = \langle pq||rs \rangle + i\Phi_{pqrs}^{\text{eh}} - i\Phi_{pqsr}^{\text{eh}}, \quad (106)$$

which leads to the following eigenvalue problem

$$C_{ab,cd}^{\text{pp}} = (\epsilon_a + \epsilon_b)\delta_{ac}\delta_{bd} + i\Lambda_{abcd} + i\Phi_{abcd}^{\text{eh}} - i\Phi_{abdc}^{\text{eh}}, \quad (107a)$$

$$B_{ab,ij}^{\text{pp}} = +i\Lambda_{abij} + i\Phi_{abij}^{\text{eh}} - i\Phi_{abji}^{\text{eh}}, \quad (107b)$$

$$D_{ij,kl}^{\text{pp}} = -(\epsilon_i + \epsilon_j)\delta_{ik}\delta_{jl} + i\Lambda_{ijkl} + i\Phi_{ijkl}^{\text{eh}} - i\Phi_{ijlk}^{\text{eh}}, \quad (107c)$$

and the effective interactions

$$M_{pq,m}^{\text{ee}} = \sum_{a<b} [i\Lambda_{pqab} + i\Phi_{pqab}^{\text{eh}} - i\Phi_{pqba}^{\text{eh}}] X_{ab,m}^{\text{ee}} + \sum_{i<j} [i\Lambda_{pqij} + i\Phi_{pqij}^{\text{eh}} - i\Phi_{pqji}^{\text{eh}}] Y_{ij,m}^{\text{ee}}, \quad (108a)$$

$$M_{pq,m}^{\text{hh}} = \sum_{i<j} [i\Lambda_{pqij} + i\Phi_{pqij}^{\text{eh}} - i\Phi_{pqji}^{\text{eh}}] X_{ij,m}^{\text{hh}} + \sum_{a<b} [i\Lambda_{pqab} + i\Phi_{pqab}^{\text{eh}} - i\Phi_{pqba}^{\text{eh}}] Y_{ab,m}^{\text{hh}}. \quad (108b)$$

Once again, a sanity check can be performed by comparing the kernel

$$i\Lambda_{ijkl} + i\Phi_{ijkl}^{\text{eh}} - i\Phi_{ijlk}^{\text{eh}} = \langle ij||kl \rangle - \sum_n \frac{M_{ki,n}^{\text{eh}} M_{lj,n}^{\text{eh},*} + M_{ik,n}^{\text{eh},*} M_{jl,n}^{\text{eh}}}{\Omega_n^{\text{eh}} - i\eta} + \sum_n \frac{M_{li,n}^{\text{eh}} M_{kj,n}^{\text{eh},*} + M_{il,n}^{\text{eh},*} M_{jk,n}^{\text{eh}}}{\Omega_n^{\text{eh}} - i\eta}, \quad (109)$$

with the static  $GW$  kernel of the pp-BSE reported in Ref. 4.

## B. Self-energy

The matrix elements of the three components of the self-energy are

$$\Sigma_{pq}^{(2)}(\omega) = -\frac{1}{2(2\pi)^2} \sum_{rst} \langle pr||st \rangle \langle st||rq \rangle \int d(\omega_1\omega_2) G_{ss}(\omega_1) G_{rr}(\omega_2) G_{tt}(\omega - \omega_1 + \omega_2), \quad (110a)$$

$$\Sigma_{pq}^{\text{eh}}(\omega) = -\frac{i}{(2\pi)^2} \sum_{rst} \langle pr||st \rangle \int d(\omega_1\omega_2) G_{ss}(\omega_1) G_{rr}(\omega_2) G_{tt}(\omega - \omega_1 + \omega_2) (\Phi^{\text{eh}})_{strq}(\omega_2 - \omega_1), \quad (110b)$$

$$\Sigma_{pq}^{\text{pp}}(\omega) = -\frac{i}{2(2\pi)^2} \sum_{rst} \langle pr||st \rangle \int d(\omega_1\omega_2) G_{ss}(\omega_1) G_{rr}(\omega_2) G_{tt}(\omega - \omega_1 + \omega_2) (\Phi_{\text{P}}^{\text{pp}})_{strq}(\omega_2 + \omega) \quad (110c)$$



Upon change of variables

$$\Sigma_{pq}^{(2)}(\omega) = -\frac{1}{2(2\pi)^2} \sum_{rst} \langle pr||st \rangle \langle st||rq \rangle \int d(\omega_1 \omega_{2'}) G_{ss}(\omega_1) G_{rr}(\omega_{2'} + \omega_1) G_{tt}(\omega + \omega_{2'}), \quad (111a)$$

$$\Sigma_{pq}^{\text{eh}}(\omega) = -\frac{i}{(2\pi)^2} \sum_{rst} \langle pr||st \rangle \int d(\omega_1 \omega_{2'}) G_{ss}(\omega_1) G_{rr}(\omega_{2'} + \omega_1) G_{tt}(\omega + \omega_{2'}) (\Phi^{\text{eh}})_{strq}(\omega_{2'}), \quad (111b)$$

$$\Sigma_{pq}^{\text{pp}}(\omega) = -\frac{i}{2(2\pi)^2} \sum_{rst} \langle pr||st \rangle \int d(\omega_1 \omega_{2'}) G_{ss}(\omega_1) G_{rr}(\omega_{2'} - \omega) G_{tt}(\omega_{2'} - \omega_1) (\Phi_{\text{P}}^{\text{pp}})_{strq}(\omega_{2'}), \quad (111c)$$

they can be rearranged into

$$\Sigma_{pq}^{(2)}(\omega) = -\frac{1}{2(2\pi)} \sum_{rst} \langle pr||st \rangle \langle st||rq \rangle \int d\omega_{2'} (L_0)_{rssr}(\omega_{2'}) G_{tt}(\omega + \omega_{2'}), \quad (112a)$$

$$\Sigma_{pq}^{\text{eh}}(\omega) = -\frac{i}{(2\pi)} \sum_{rst} \langle pr||st \rangle \int d\omega_{2'} (L_0)_{rssr}(\omega_{2'}) G_{tt}(\omega + \omega_{2'}) (\Phi^{\text{eh}})_{strq}(\omega_{2'}), \quad (112b)$$

$$\Sigma_{pq}^{\text{pp}}(\omega) = -\frac{i}{2(2\pi)} \sum_{rst} \langle pr||st \rangle \int d\omega_{2'} (K_{0,\text{P}}^{\text{I}})_{tsts}(\omega_{2'}) G_{rr}(\omega_{2'} - \omega) (\Phi_{\text{P}}^{\text{pp}})_{strq}(\omega_{2'}). \quad (112c)$$

### 1. eh self-energy

The eh part is derived as

$$\begin{aligned} \Sigma_{pq}^{\text{eh}}(\omega) &= -\frac{i}{(2\pi)} \langle pr||st \rangle \int d\omega_{2'} (L_0)_{rssr}(\omega_{2'}) G_{tt}(\omega + \omega_{2'}) (\Phi^{\text{eh}})_{strq}(\omega_{2'}) \\ &= -\frac{i}{(2\pi)} \langle pr||st \rangle \int d\omega_{2'} \left[ i \sum_{ia} \frac{\delta_{ra} \delta_{si}}{\omega_{2'} - (\epsilon_a - \epsilon_i - 2i\eta)} - i \sum_{ia} \frac{\delta_{ri} \delta_{sa}}{\omega_{2'} - (\epsilon_i - \epsilon_a + 2i\eta)} \right] \\ &\quad \times \left[ \sum_j \frac{\delta_{tj}}{\omega + \omega_{2'} - (\epsilon_j + i\eta)} + \sum_b \frac{\delta_{tb}}{\omega + \omega_{2'} - (\epsilon_b - i\eta)} \right] \left[ -i \sum_n \frac{M_{sr,n}^{\text{eh}} M_{qt,n}^{\text{eh},*}}{\omega_{2'} - (\Omega_n^{\text{eh}} - i\eta)} + i \sum_n \frac{M_{rs,n}^{\text{eh},*} M_{tq,n}^{\text{eh}}}{\omega_{2'} - (-\Omega_n^{\text{eh}} + i\eta)} \right] \\ &= -\frac{i}{(2\pi)} \langle pr||st \rangle \int d\omega_{2'} \left[ \sum_{ia} \frac{\delta_{ra} \delta_{si}}{\omega_{2'} - (\epsilon_a - \epsilon_i - 2i\eta)} - \sum_{ia} \frac{\delta_{ri} \delta_{sa}}{\omega_{2'} - (\epsilon_i - \epsilon_a + 2i\eta)} \right] \\ &\quad \times \left[ \sum_j \frac{\delta_{tj}}{\omega_{2'} - (\epsilon_j - \omega + i\eta)} + \sum_b \frac{\delta_{tb}}{\omega_{2'} - (\epsilon_b - \omega - i\eta)} \right] \left[ \sum_n \frac{M_{sr,n}^{\text{eh}} M_{qt,n}^{\text{eh},*}}{\omega_{2'} - (\Omega_n^{\text{eh}} - i\eta)} - \sum_n \frac{M_{rs,n}^{\text{eh},*} M_{tq,n}^{\text{eh}}}{\omega_{2'} - (-\Omega_n^{\text{eh}} + i\eta)} \right] \\ &= -\frac{i}{(2\pi)} \langle pr||st \rangle \int d\omega_{2'} \left[ -\sum_{iabn} \frac{\delta_{ri} \delta_{sa}}{\omega_{2'} - (\epsilon_i - \epsilon_a + 2i\eta)} \frac{\delta_{tb}}{\omega_{2'} - (\epsilon_b - \omega - i\eta)} \frac{M_{sr,n}^{\text{eh}} M_{qt,n}^{\text{eh},*}}{\omega_{2'} - (\Omega_n^{\text{eh}} - i\eta)} \right. \\ &\quad + \sum_{ijan} \frac{\delta_{ra} \delta_{si}}{\omega_{2'} - (\epsilon_a - \epsilon_i - 2i\eta)} \frac{\delta_{tj}}{\omega_{2'} - (\epsilon_j - \omega + i\eta)} \frac{M_{sr,n}^{\text{eh}} M_{qt,n}^{\text{eh},*}}{\omega_{2'} - (\Omega_n^{\text{eh}} - i\eta)} \\ &\quad - \sum_{iabn} \frac{\delta_{ra} \delta_{si}}{\omega_{2'} - (\epsilon_a - \epsilon_i - 2i\eta)} \frac{\delta_{tb}}{\omega_{2'} - (\epsilon_b - \omega - i\eta)} \frac{M_{rs,n}^{\text{eh},*} M_{tq,n}^{\text{eh}}}{\omega_{2'} - (-\Omega_n^{\text{eh}} + i\eta)} \\ &\quad - \sum_{ijan} \frac{\delta_{ra} \delta_{si}}{\omega_{2'} - (\epsilon_a - \epsilon_i - 2i\eta)} \frac{\delta_{tj}}{\omega_{2'} - (\epsilon_j - \omega + i\eta)} \frac{M_{rs,n}^{\text{eh},*} M_{tq,n}^{\text{eh}}}{\omega_{2'} - (-\Omega_n^{\text{eh}} + i\eta)} \\ &\quad + \sum_{iabn} \frac{\delta_{ri} \delta_{sa}}{\omega_{2'} - (\epsilon_i - \epsilon_a + 2i\eta)} \frac{\delta_{tb}}{\omega_{2'} - (\epsilon_b - \omega - i\eta)} \frac{M_{rs,n}^{\text{eh},*} M_{tq,n}^{\text{eh}}}{\omega_{2'} - (-\Omega_n^{\text{eh}} + i\eta)} \\ &\quad \left. - \sum_{ijan} \frac{\delta_{ri} \delta_{sa}}{\omega_{2'} - (\epsilon_i - \epsilon_a + 2i\eta)} \frac{\delta_{tj}}{\omega_{2'} - (\epsilon_j - \omega + i\eta)} \frac{M_{sr,n}^{\text{eh}} M_{qt,n}^{\text{eh},*}}{\omega_{2'} - (\Omega_n^{\text{eh}} - i\eta)} \right] \end{aligned} \quad (113)$$

$$\begin{aligned}
&= - \sum_{iabn} \frac{\langle pr||st \rangle \delta_{ri} \delta_{sa} \delta_{tb}}{(\epsilon_i - \epsilon_a + 2i\eta) - (\epsilon_b - \omega - i\eta)} \frac{M_{sr,n}^{\text{eh}} M_{qt,n}^{\text{eh},*}}{(\epsilon_i - \epsilon_a + 2i\eta) - (\Omega_n^{\text{eh}} - i\eta)} \\
&\quad + \sum_{ijan} \frac{\langle pr||st \rangle \delta_{ra} \delta_{si} \delta_{tj}}{(\epsilon_j - \omega + i\eta) - (\epsilon_a - \epsilon_i - 2i\eta)} \frac{M_{sr,n}^{\text{eh}} M_{qt,n}^{\text{eh},*}}{(\epsilon_j - \omega + i\eta) - (\Omega_n^{\text{eh}} - i\eta)} \\
&\quad - \sum_{iabn} \frac{\langle pr||st \rangle \delta_{ra} \delta_{si} \delta_{tb}}{(-\Omega_n^{\text{eh}} + i\eta) - (\epsilon_a - \epsilon_i - 2i\eta)} \frac{M_{rs,n}^{\text{eh},*} M_{tq,n}^{\text{eh}}}{(-\Omega_n^{\text{eh}} + i\eta) - (\epsilon_b - \omega - i\eta)} \\
&\quad + \sum_{ijan} \frac{\langle pr||st \rangle \delta_{ra} \delta_{si} \delta_{tj}}{(\epsilon_a - \epsilon_i - 2i\eta) - (\epsilon_j - \omega + i\eta)} \frac{M_{rs,n}^{\text{eh},*} M_{tq,n}^{\text{eh}}}{(\epsilon_a - \epsilon_i - 2i\eta) - (-\Omega_n^{\text{eh}} + i\eta)} \\
&\quad - \sum_{iabn} \frac{\langle pr||st \rangle \delta_{ri} \delta_{sa} \delta_{tb}}{(\epsilon_b - \omega - i\eta) - (\epsilon_i - \epsilon_a + 2i\eta)} \frac{M_{rs,n}^{\text{eh},*} M_{tq,n}^{\text{eh}}}{(\epsilon_b - \omega - i\eta) - (-\Omega_n^{\text{eh}} + i\eta)} \\
&\quad + \sum_{ijan} \frac{\langle pr||st \rangle \delta_{ri} \delta_{sa} \delta_{tj}}{(\Omega_n^{\text{eh}} - i\eta) - (\epsilon_i - \epsilon_a + 2i\eta)} \frac{M_{sr,n}^{\text{eh}} M_{qt,n}^{\text{eh},*}}{(\Omega_n^{\text{eh}} - i\eta) - (\epsilon_j - \omega + i\eta)} \\
&= - \sum_{iabn} \frac{\langle pr||sb \rangle \delta_{ri} \delta_{sa}}{\omega - (\epsilon_a + \epsilon_b - \epsilon_i - 3i\eta)} \frac{M_{sr,n}^{\text{eh}} M_{qb,n}^{\text{eh},*}}{\epsilon_i - \epsilon_a - \Omega_n^{\text{eh}} + 3i\eta} \\
&\quad + \sum_{ijan} \frac{\langle pr||sj \rangle \delta_{ra} \delta_{si}}{(\epsilon_i + \epsilon_j - \epsilon_a + 3i\eta) - \omega} \frac{M_{sr,n}^{\text{eh}} M_{qj,n}^{\text{eh},*}}{(\epsilon_j - \Omega_n^{\text{eh}} + 2i\eta) - \omega} \\
&\quad - \sum_{iabn} \frac{\langle pr||sb \rangle \delta_{ra} \delta_{si}}{-\Omega_n^{\text{eh}} - \epsilon_a + \epsilon_i + 3i\eta} \frac{M_{rs,n}^{\text{eh},*} M_{bq,n}^{\text{eh}}}{\omega - (\epsilon_b + \Omega_n^{\text{eh}} - 2i\eta)} \\
&\quad + \sum_{ijan} \frac{\langle pr||sj \rangle \delta_{ra} \delta_{si}}{\omega - (\epsilon_i + \epsilon_j - \epsilon_a + 3i\eta)} \frac{M_{rs,n}^{\text{eh},*} M_{jq,n}^{\text{eh}}}{\epsilon_a - \epsilon_i + \Omega_n^{\text{eh}} - 3i\eta} \\
&\quad - \sum_{iabn} \frac{\langle pr||sb \rangle \delta_{ri} \delta_{sa}}{(\epsilon_a + \epsilon_b - \epsilon_i - 3i\eta) - \omega} \frac{M_{rs,n}^{\text{eh},*} M_{bq,n}^{\text{eh}}}{(\epsilon_b + \Omega_n^{\text{eh}} - 2i\eta) - \omega} \\
&\quad + \sum_{ijan} \frac{\langle pr||sj \rangle \delta_{ri} \delta_{sa}}{\Omega_n^{\text{eh}} - \epsilon_i + \epsilon_a - 3i\eta} \frac{M_{sr,n}^{\text{eh}} M_{qj,n}^{\text{eh},*}}{\omega - (\epsilon_j - \Omega_n^{\text{eh}} + 2i\eta)} \\
&= \sum_{iabn} \frac{\langle pi||ab \rangle}{\omega - (\epsilon_a + \epsilon_b - \epsilon_i - 3i\eta)} \frac{M_{ai,n}^{\text{eh}} M_{qb,n}^{\text{eh},*}}{\epsilon_a - \epsilon_i + \Omega_n^{\text{eh}} - 3i\eta} \\
&\quad + \sum_{ijan} \frac{\langle pa||ij \rangle}{\omega - (\epsilon_i + \epsilon_j - \epsilon_a + 3i\eta)} \frac{M_{ia,n}^{\text{eh}} M_{qj,n}^{\text{eh},*}}{\omega - (\epsilon_j - \Omega_n^{\text{eh}} + 2i\eta)} \\
&\quad + \sum_{iabn} \frac{\langle pa||ib \rangle}{\epsilon_a - \epsilon_i + \Omega_n^{\text{eh}} - 3i\eta} \frac{M_{ai,n}^{\text{eh},*} M_{bq,n}^{\text{eh}}}{\omega - (\epsilon_b + \Omega_n^{\text{eh}} - 2i\eta)} \\
&\quad + \sum_{ijan} \frac{\langle pa||ij \rangle}{\omega - (\epsilon_i + \epsilon_j - \epsilon_a + 3i\eta)} \frac{M_{ai,n}^{\text{eh},*} M_{jq,n}^{\text{eh}}}{\epsilon_a - \epsilon_i + \Omega_n^{\text{eh}} - 3i\eta} \\
&\quad - \sum_{iabn} \frac{\langle pi||ab \rangle}{\omega - (\epsilon_a + \epsilon_b - \epsilon_i - 3i\eta)} \frac{M_{ia,n}^{\text{eh},*} M_{bq,n}^{\text{eh}}}{\omega - (\epsilon_b + \Omega_n^{\text{eh}} - 2i\eta)} \\
&\quad + \sum_{ijan} \frac{\langle pi||aj \rangle}{\epsilon_a - \epsilon_i + \Omega_n^{\text{eh}} - 3i\eta} \frac{M_{ai,n}^{\text{eh}} M_{qj,n}^{\text{eh},*}}{\omega - (\epsilon_j - \Omega_n^{\text{eh}} + 2i\eta)}
\end{aligned}$$

This finally yields

$$\begin{aligned}
\Sigma_{pq}^{\text{eh}}(\omega) = & \\
& + \sum_{ijan} \frac{\langle pa||ij \rangle}{\epsilon_a - \epsilon_i - \Omega_n^{\text{eh}} - i\eta} \frac{M_{ia,n}^{\text{eh}} M_{jq,n}^{\text{eh},*}}{\omega - (\epsilon_j - \Omega_n^{\text{eh}} + 2i\eta)} - \sum_{ijan} \frac{\langle pa||ij \rangle}{\epsilon_a - \epsilon_i - \Omega_n^{\text{eh}} - i\eta} \frac{M_{ia,n}^{\text{eh}} M_{jq,n}^{\text{eh},*}}{\omega - (\epsilon_i + \epsilon_j - \epsilon_a + 3i\eta)} \\
& + \sum_{ijan} \frac{\langle pa||ij \rangle}{\epsilon_a - \epsilon_i + \Omega_n^{\text{eh}} - 3i\eta} \frac{M_{ai,n}^{\text{eh},*} M_{jq,n}^{\text{eh}}}{\omega - (\epsilon_i + \epsilon_j - \epsilon_a + 3i\eta)} + \sum_{ijan} \frac{\langle pi||aj \rangle}{\epsilon_a - \epsilon_i + \Omega_n^{\text{eh}} - 3i\eta} \frac{M_{ai,n}^{\text{eh}} M_{jq,n}^{\text{eh},*}}{\omega - (\epsilon_j - \Omega_n^{\text{eh}} + 2i\eta)} \\
& + \sum_{iabn} \frac{\langle pi||ab \rangle}{\epsilon_a - \epsilon_i - \Omega_n^{\text{eh}} - i\eta} \frac{M_{ia,n}^{\text{eh},*} M_{bq,n}^{\text{eh}}}{\omega - (\epsilon_b + \Omega_n^{\text{eh}} - 2i\eta)} - \sum_{iabn} \frac{\langle pi||ab \rangle}{\epsilon_a - \epsilon_i - \Omega_n^{\text{eh}} - i\eta} \frac{M_{ia,n}^{\text{eh},*} M_{bq,n}^{\text{eh}}}{\omega - (\epsilon_a + \epsilon_b - \epsilon_i - 3i\eta)} \\
& + \sum_{iabn} \frac{\langle pi||ab \rangle}{\epsilon_a - \epsilon_i + \Omega_n^{\text{eh}} - 3i\eta} \frac{M_{ai,n}^{\text{eh}} M_{qb,n}^{\text{eh},*}}{\omega - (\epsilon_a + \epsilon_b - \epsilon_i - 3i\eta)} + \sum_{iabn} \frac{\langle pa||ib \rangle}{\epsilon_a - \epsilon_i + \Omega_n^{\text{eh}} - 3i\eta} \frac{M_{ai,n}^{\text{eh},*} M_{bq,n}^{\text{eh}}}{\omega - (\epsilon_b + \Omega_n^{\text{eh}} - 2i\eta)},
\end{aligned} \tag{114}$$

This expression can be rewritten in terms of intermediate quantities as

$$\begin{aligned}
\Sigma_{pq}^{\text{eh}}(\omega) = & \\
& + \sum_{jn} \left( \sum_{ia} \frac{\langle pa||ij \rangle M_{ia,n}^{\text{eh}}}{\epsilon_a - \epsilon_i - \Omega_n^{\text{eh}} - i\eta} \right) \frac{M_{jq,n}^{\text{eh},*}}{\omega - (\epsilon_j - \Omega_n^{\text{eh}} + 2i\eta)} - \sum_{ija} \left( \sum_n \frac{M_{ia,n}^{\text{eh}} M_{jq,n}^{\text{eh},*}}{\epsilon_a - \epsilon_i - \Omega_n^{\text{eh}} - i\eta} \right) \frac{\langle pa||ij \rangle}{\omega - (\epsilon_i + \epsilon_j - \epsilon_a + 3i\eta)} \\
& + \sum_{ija} \left( \sum_n \frac{M_{ai,n}^{\text{eh},*} M_{jq,n}^{\text{eh}}}{\epsilon_a - \epsilon_i + \Omega_n^{\text{eh}} - 3i\eta} \right) \frac{\langle pa||ij \rangle}{\omega - (\epsilon_i + \epsilon_j - \epsilon_a + 3i\eta)} + \sum_{jn} \left( \sum_{ia} \frac{\langle pi||aj \rangle M_{ai,n}^{\text{eh}}}{\epsilon_a - \epsilon_i + \Omega_n^{\text{eh}} - 3i\eta} \right) \frac{M_{jq,n}^{\text{eh},*}}{\omega - (\epsilon_j - \Omega_n^{\text{eh}} + 2i\eta)} \\
& + \sum_{bn} \left( \sum_{ia} \frac{\langle pi||ab \rangle M_{ia,n}^{\text{eh},*}}{\epsilon_a - \epsilon_i - \Omega_n^{\text{eh}} - i\eta} \right) \frac{M_{bq,n}^{\text{eh}}}{\omega - (\epsilon_b + \Omega_n^{\text{eh}} - 2i\eta)} - \sum_{iab} \left( \sum_n \frac{M_{ia,n}^{\text{eh},*} M_{bq,n}^{\text{eh}}}{\epsilon_a - \epsilon_i - \Omega_n^{\text{eh}} - i\eta} \right) \frac{\langle pi||ab \rangle}{\omega - (\epsilon_a + \epsilon_b - \epsilon_i - 3i\eta)} \\
& + \sum_{iab} \left( \sum_n \frac{M_{ai,n}^{\text{eh}} M_{qb,n}^{\text{eh},*}}{\epsilon_a - \epsilon_i + \Omega_n^{\text{eh}} - 3i\eta} \right) \frac{\langle pi||ab \rangle}{\omega - (\epsilon_a + \epsilon_b - \epsilon_i - 3i\eta)} + \sum_{bn} \left( \sum_{ia} \frac{\langle pa||ib \rangle M_{ai,n}^{\text{eh},*}}{\epsilon_a - \epsilon_i + \Omega_n^{\text{eh}} - 3i\eta} \right) \frac{M_{bq,n}^{\text{eh}}}{\omega - (\epsilon_b + \Omega_n^{\text{eh}} - 2i\eta)},
\end{aligned} \tag{115}$$

or, more compactly,

$$\begin{aligned}
\Sigma_{pq}^{\text{eh}}(\omega) = & + \sum_{jn} \frac{\tilde{M}_{pj,n}^{\text{eh}} M_{jq,n}^{\text{eh},*}}{\omega - (\epsilon_j - \Omega_n^{\text{eh}} + 2i\eta)} + \sum_{ija} \frac{\tilde{M}_{qj,ia}^{\text{eh}} \langle pa||ij \rangle}{\omega - (\epsilon_i + \epsilon_j - \epsilon_a + 3i\eta)} \\
& + \sum_{bn} \frac{\tilde{M}_{pb,n}^{\text{eh}} M_{bq,n}^{\text{eh}}}{\omega - (\epsilon_b + \Omega_n^{\text{eh}} - 2i\eta)} + \sum_{iab} \frac{\tilde{M}_{qb,ia}^{\text{eh}} \langle pi||ab \rangle}{\omega - (\epsilon_a + \epsilon_b - \epsilon_i - 3i\eta)}
\end{aligned} \tag{116}$$

with

$$\tilde{M}_{pj,n}^{\text{eh}} = \sum_{ia} \frac{\langle pa||ij \rangle M_{ia,n}^{\text{eh}}}{\epsilon_a - \epsilon_i - \Omega_n^{\text{eh}} - i\eta} + \sum_{ia} \frac{\langle pi||aj \rangle M_{ai,n}^{\text{eh}}}{\epsilon_a - \epsilon_i + \Omega_n^{\text{eh}} - 3i\eta} \tag{117a}$$

$$\tilde{M}_{qj,ia}^{\text{eh}} = \sum_n \frac{M_{ai,n}^{\text{eh},*} M_{jq,n}^{\text{eh}}}{\epsilon_a - \epsilon_i + \Omega_n^{\text{eh}} - 3i\eta} - \sum_n \frac{M_{ia,n}^{\text{eh}} M_{jq,n}^{\text{eh},*}}{\epsilon_a - \epsilon_i - \Omega_n^{\text{eh}} - i\eta} \tag{117b}$$

$$\tilde{M}_{pb,n}^{\text{eh}} = \sum_{ia} \frac{\langle pi||ab \rangle M_{ia,n}^{\text{eh},*}}{\epsilon_a - \epsilon_i - \Omega_n^{\text{eh}} - i\eta} + \sum_{ia} \frac{\langle pa||ib \rangle M_{ai,n}^{\text{eh},*}}{\epsilon_a - \epsilon_i + \Omega_n^{\text{eh}} - 3i\eta} \tag{117c}$$

$$\tilde{M}_{qb,ia}^{\text{eh}} = \sum_n \frac{M_{ai,n}^{\text{eh}} M_{qb,n}^{\text{eh},*}}{\epsilon_a - \epsilon_i + \Omega_n^{\text{eh}} - 3i\eta} - \sum_n \frac{M_{ia,n}^{\text{eh},*} M_{bq,n}^{\text{eh}}}{\epsilon_a - \epsilon_i - \Omega_n^{\text{eh}} - i\eta} \tag{117d}$$

Each intermediate tensor is computed in  $\mathcal{O}(K^6)$  operations, while, given the intermediate, the construction of the self-energy matrix costs  $\mathcal{O}(K^5)$ .

## 2. *pp* self-energy

The *pp* part is derived as

$$\begin{aligned}
\Sigma_{pq}^{\text{pp}}(\omega) &= -\frac{i}{2(2\pi)} \langle pr || st \rangle \int d\omega_{2'} G_{rr}(\omega_{2'} - \omega) (K_{0,\text{P}}^I)_{tsts}(\omega_{2'}) (\Phi_{\text{P}}^{\text{pp}})_{strq}(\omega_{2'}) \\
&= -\frac{i}{2(2\pi)} \langle pr || st \rangle \int d\omega_{2'} \left[ \sum_i \frac{\delta_{ri}}{\omega_{2'} - \omega - (\epsilon_i + i\eta)} + \sum_a \frac{\delta_{ra}}{\omega_{2'} - \omega - (\epsilon_a - i\eta)} \right] \\
&\quad \left[ i \sum_{jk} \frac{\delta_{tj} \delta_{sk}}{\omega_{2'} - (\epsilon_j + \epsilon_i + 2i\eta)} - i \sum_{bc} \frac{\delta_{tb} \delta_{sc}}{\omega_{2'} - (\epsilon_b + \epsilon_c - 2i\eta)} \right] \left[ -i \sum_m \frac{M_{st,m}^{\text{ee}} M_{rq,m}^{\text{ee},*}}{\omega_{2'} - (\Omega_m^{\text{ee}} - i\eta)} + i \sum_m \frac{M_{st,m}^{\text{hh},*} M_{rq,m}^{\text{hh}}}{\omega_{2'} - (\Omega_m^{\text{hh}} + i\eta)} \right] \\
&= -\frac{i}{2(2\pi)} \langle pr || st \rangle \int d\omega_{2'} \left[ \sum_i \frac{\delta_{ri}}{\omega_{2'} - (\omega + \epsilon_i + i\eta)} + \sum_a \frac{\delta_{ra}}{\omega_{2'} - (\omega + \epsilon_a - i\eta)} \right] \\
&\quad \left[ \sum_{jk} \frac{\delta_{tj} \delta_{sk}}{\omega_{2'} - (\epsilon_j + \epsilon_i + 2i\eta)} - \sum_{bc} \frac{\delta_{tb} \delta_{sc}}{\omega_{2'} - (\epsilon_b + \epsilon_c - 2i\eta)} \right] \left[ \sum_m \frac{M_{st,m}^{\text{ee}} M_{rq,m}^{\text{ee},*}}{\omega_{2'} - (\Omega_m^{\text{ee}} - i\eta)} - \sum_m \frac{M_{st,m}^{\text{hh},*} M_{rq,m}^{\text{hh}}}{\omega_{2'} - (\Omega_m^{\text{hh}} + i\eta)} \right] \\
&= -\frac{i}{2(2\pi)} \langle pr || st \rangle \int d\omega_{2'} \\
&\quad \left[ - \sum_{ibcm} \frac{\delta_{ri}}{\omega_{2'} - (\omega + \epsilon_i + i\eta)} \frac{\delta_{tb} \delta_{sc}}{\omega_{2'} - (\epsilon_b + \epsilon_c - 2i\eta)} \frac{M_{st,m}^{\text{ee}} M_{rq,m}^{\text{ee},*}}{\omega_{2'} - (\Omega_m^{\text{ee}} - i\eta)} \right. \\
&\quad + \sum_{ajkm} \frac{\delta_{ra}}{\omega_{2'} - (\omega + \epsilon_a - i\eta)} \frac{\delta_{tj} \delta_{sk}}{\omega_{2'} - (\epsilon_j + \epsilon_k + 2i\eta)} \frac{M_{st,m}^{\text{ee}} M_{rq,m}^{\text{ee},*}}{\omega_{2'} - (\Omega_m^{\text{ee}} - i\eta)} \\
&\quad + \sum_{abcm} \frac{\delta_{ra}}{\omega_{2'} - (\omega + \epsilon_a - i\eta)} \frac{\delta_{tb} \delta_{sc}}{\omega_{2'} - (\epsilon_b + \epsilon_c - 2i\eta)} \frac{M_{st,m}^{\text{hh},*} M_{rq,m}^{\text{hh}}}{\omega_{2'} - (\Omega_m^{\text{hh}} + i\eta)} \\
&\quad - \sum_{ajkm} \frac{\delta_{ra}}{\omega_{2'} - (\omega + \epsilon_a - i\eta)} \frac{\delta_{tj} \delta_{sk}}{\omega_{2'} - (\epsilon_j + \epsilon_k + 2i\eta)} \frac{M_{st,m}^{\text{hh},*} M_{rq,m}^{\text{hh}}}{\omega_{2'} - (\Omega_m^{\text{hh}} + i\eta)} \\
&\quad + \sum_{ibcm} \frac{\delta_{ri}}{\omega_{2'} - (\omega + \epsilon_i + i\eta)} \frac{\delta_{tb} \delta_{sc}}{\omega_{2'} - (\epsilon_b + \epsilon_c - 2i\eta)} \frac{M_{st,m}^{\text{hh},*} M_{rq,m}^{\text{hh}}}{\omega_{2'} - (\Omega_m^{\text{hh}} + i\eta)} \\
&\quad \left. + \sum_{ijkm} \frac{\delta_{ri}}{\omega_{2'} - (\omega + \epsilon_i + i\eta)} \frac{\delta_{tj} \delta_{sk}}{\omega_{2'} - (\epsilon_j + \epsilon_k + 2i\eta)} \frac{M_{st,m}^{\text{ee}} M_{rq,m}^{\text{ee},*}}{\omega_{2'} - (\Omega_m^{\text{ee}} - i\eta)} \right] \\
&= \frac{1}{2} \left[ - \sum_{ibcm} \frac{\langle pi || cb \rangle}{(\omega + \epsilon_i + i\eta) - (\epsilon_b + \epsilon_c - 2i\eta)} \frac{M_{cb,m}^{\text{ee}} M_{iq,m}^{\text{ee},*}}{(\omega + \epsilon_i + i\eta) - (\Omega_m^{\text{ee}} - i\eta)} \right. \\
&\quad + \sum_{ajkm} \frac{\langle pa || kj \rangle}{(\epsilon_j + \epsilon_k + 2i\eta) - (\omega + \epsilon_a - i\eta)} \frac{M_{kj,m}^{\text{ee}} M_{aq,m}^{\text{ee},*}}{(\epsilon_j + \epsilon_k + 2i\eta) - (\Omega_m^{\text{ee}} - i\eta)} \\
&\quad + \sum_{abcm} \frac{\langle pa || cb \rangle}{(\Omega_m^{\text{hh}} + i\eta) - (\omega + \epsilon_a - i\eta)} \frac{M_{cb,m}^{\text{hh},*} M_{aq,m}^{\text{hh}}}{(\Omega_m^{\text{hh}} + i\eta) - (\epsilon_b + \epsilon_c - 2i\eta)} \\
&\quad + \sum_{ajkm} \frac{\langle pa || kj \rangle}{(\omega + \epsilon_a - i\eta) - (\epsilon_j + \epsilon_k + 2i\eta)} \frac{M_{kj,m}^{\text{hh},*} M_{aq,m}^{\text{hh}}}{(\omega + \epsilon_a - i\eta) - (\Omega_m^{\text{hh}} + i\eta)} \\
&\quad - \sum_{ibcm} \frac{\langle pi || cb \rangle}{(\epsilon_b + \epsilon_c - 2i\eta) - (\omega + \epsilon_i + i\eta)} \frac{M_{cb,m}^{\text{hh},*} M_{iq,m}^{\text{hh}}}{(\epsilon_b + \epsilon_c - 2i\eta) - (\Omega_m^{\text{hh}} + i\eta)} \\
&\quad \left. - \sum_{ijkm} \frac{\langle pi || kj \rangle}{(\Omega_m^{\text{ee}} - i\eta) - (\omega + \epsilon_i + i\eta)} \frac{M_{kj,m}^{\text{ee}} M_{iq,m}^{\text{ee},*}}{(\Omega_m^{\text{ee}} - i\eta) - (\epsilon_j + \epsilon_k + 2i\eta)} \right]
\end{aligned}$$

$$\begin{aligned}
&= \frac{1}{2} \left[ - \sum_{ibcm} \frac{\langle pi||cb \rangle}{\omega - (\epsilon_b + \epsilon_c - \epsilon_i - 3i\eta)} \frac{M_{cb,m}^{ee} M_{iq,m}^{ee,*}}{\omega - (\Omega_m^{ee} - \epsilon_i - 2i\eta)} \right. \\
&\quad - \sum_{ajkm} \frac{\langle pa||kj \rangle}{\omega - (\epsilon_j + \epsilon_k - \epsilon_a + 3i\eta)} \frac{M_{kj,m}^{ee} M_{aq,m}^{ee,*}}{\epsilon_j + \epsilon_k - \Omega_m^{ee} + 3i\eta} \\
&\quad - \sum_{abcm} \frac{\langle pa||cb \rangle}{\omega - (\Omega_m^{hh} - \epsilon_a + 2i\eta)} \frac{M_{cb,m}^{hh,*} M_{aq,m}^{hh}}{\Omega_m^{hh} - \epsilon_b - \epsilon_c + 3i\eta} \\
&\quad + \sum_{ajkm} \frac{\langle pa||kj \rangle}{\omega - (\epsilon_j + \epsilon_k - \epsilon_a + 3i\eta)} \frac{M_{kj,m}^{hh,*} M_{aq,m}^{hh}}{\omega - (\Omega_m^{hh} - \epsilon_a + 2i\eta)} \\
&\quad + \sum_{ibcm} \frac{\langle pi||cb \rangle}{\omega - (\epsilon_b + \epsilon_c - \epsilon_i - 3i\eta)} \frac{M_{cb,m}^{hh,*} M_{iq,m}^{hh}}{\epsilon_b + \epsilon_c - \Omega_m^{hh} - 3i\eta} \\
&\quad \left. + \sum_{ijkm} \frac{\langle pi||kj \rangle}{\omega - (\Omega_m^{ee} - \epsilon_i - i\eta)} \frac{M_{kj,m}^{ee} M_{iq,m}^{ee,*}}{\Omega_m^{ee} - \epsilon_j - \epsilon_k - 3i\eta} \right] \quad (119)
\end{aligned}$$

This finally yields

$$\begin{aligned}
\Sigma_{pq}^{pp}(\omega) = & \\
& + \frac{1}{2} \sum_{ijam} \frac{\langle pa||ij \rangle}{\Omega_m^{hh} - \epsilon_i - \epsilon_j - i\eta} \frac{M_{ij,m}^{hh,*} M_{aq,m}^{hh}}{\omega - (\Omega_m^{hh} - \epsilon_a + 2i\eta)} - \frac{1}{2} \sum_{ijam} \frac{\langle pa||ij \rangle}{\Omega_m^{hh} - \epsilon_i - \epsilon_j - i\eta} \frac{M_{ij,m}^{hh,*} M_{aq,m}^{hh}}{\omega - (\epsilon_i + \epsilon_j - \epsilon_a + 3i\eta)} \\
& + \frac{1}{2} \sum_{ijam} \frac{\langle pa||ij \rangle}{\Omega_m^{ee} - \epsilon_i - \epsilon_j - 3i\eta} \frac{M_{ij,m}^{ee} M_{aq,m}^{ee,*}}{\omega - (\epsilon_i + \epsilon_j - \epsilon_a + 3i\eta)} + \frac{1}{2} \sum_{abcm} \frac{\langle pa||bc \rangle}{\epsilon_b + \epsilon_c - \Omega_m^{hh} - 3i\eta} \frac{M_{bc,m}^{hh,*} M_{aq,m}^{hh}}{\omega - (\Omega_m^{hh} - \epsilon_a + 2i\eta)} \quad (120) \\
& + \frac{1}{2} \sum_{iabm} \frac{\langle pi||ab \rangle}{\epsilon_a + \epsilon_b - \Omega_m^{ee} - i\eta} \frac{M_{ab,m}^{ee} M_{iq,m}^{ee,*}}{\omega - (\Omega_m^{ee} - \epsilon_i - 2i\eta)} - \frac{1}{2} \sum_{iabm} \frac{\langle pi||ab \rangle}{\epsilon_a + \epsilon_b - \Omega_m^{ee} - i\eta} \frac{M_{ab,m}^{ee} M_{iq,m}^{ee,*}}{\omega - (\epsilon_a + \epsilon_b - \epsilon_i - 3i\eta)} \\
& + \frac{1}{2} \sum_{iabm} \frac{\langle pi||ab \rangle}{\epsilon_a + \epsilon_b - \Omega_m^{hh} - 3i\eta} \frac{M_{ab,m}^{hh,*} M_{iq,m}^{hh}}{\omega - (\epsilon_a + \epsilon_b - \epsilon_i - 3i\eta)} + \frac{1}{2} \sum_{ijkm} \frac{\langle pi||jk \rangle}{\Omega_m^{ee} - \epsilon_j - \epsilon_k - 3i\eta} \frac{M_{jk,m}^{ee} M_{iq,m}^{ee,*}}{\omega - (\Omega_m^{ee} - \epsilon_i - 2i\eta)},
\end{aligned}$$

This expression can be rewritten in terms of intermediate quantities as

$$\begin{aligned}
\Sigma_{pq}^{pp}(\omega) = & \\
& + \frac{1}{2} \sum_{am} \left( \sum_{ij} \frac{\langle pa||ij \rangle M_{ij,m}^{hh,*}}{\Omega_m^{hh} - \epsilon_i - \epsilon_j - i\eta} \right) \frac{M_{aq,m}^{hh}}{\omega - (\Omega_m^{hh} - \epsilon_a + 2i\eta)} - \frac{1}{2} \sum_{ija} \left( \sum_m \frac{M_{ij,m}^{hh,*} M_{aq,m}^{hh}}{\Omega_m^{hh} - \epsilon_i - \epsilon_j - i\eta} \right) \frac{\langle pa||ij \rangle}{\omega - (\epsilon_i + \epsilon_j - \epsilon_a + 3i\eta)} \\
& + \frac{1}{2} \sum_{ija} \left( \sum_m \frac{M_{ij,m}^{ee} M_{aq,m}^{ee,*}}{\Omega_m^{ee} - \epsilon_i - \epsilon_j - 3i\eta} \right) \frac{\langle pa||ij \rangle}{\omega - (\epsilon_i + \epsilon_j - \epsilon_a + 3i\eta)} + \frac{1}{2} \sum_{am} \left( \sum_{bc} \frac{\langle pa||bc \rangle M_{bc,m}^{hh,*}}{\epsilon_b + \epsilon_c - \Omega_m^{hh} - 3i\eta} \right) \frac{M_{aq,m}^{hh}}{\omega - (\Omega_m^{hh} - \epsilon_a + 2i\eta)} \\
& + \frac{1}{2} \sum_{im} \left( \sum_{ab} \frac{\langle pi||ab \rangle M_{ab,m}^{ee}}{\epsilon_a + \epsilon_b - \Omega_m^{ee} - i\eta} \right) \frac{M_{iq,m}^{ee,*}}{\omega - (\Omega_m^{ee} - \epsilon_i - 2i\eta)} - \frac{1}{2} \sum_{iab} \left( \sum_m \frac{M_{ab,m}^{ee} M_{iq,m}^{ee,*}}{\epsilon_a + \epsilon_b - \Omega_m^{ee} - i\eta} \right) \frac{\langle pi||ab \rangle}{\omega - (\epsilon_a + \epsilon_b - \epsilon_i - 3i\eta)} \\
& + \frac{1}{2} \sum_{iab} \left( \sum_m \frac{M_{ab,m}^{hh,*} M_{iq,m}^{hh}}{\epsilon_a + \epsilon_b - \Omega_m^{hh} - 3i\eta} \right) \frac{\langle pi||ab \rangle}{\omega - (\epsilon_a + \epsilon_b - \epsilon_i - 3i\eta)} + \frac{1}{2} \sum_{im} \left( \sum_{jk} \frac{\langle pi||jk \rangle M_{jk,m}^{ee}}{\Omega_m^{ee} - \epsilon_j - \epsilon_k - 3i\eta} \right) \frac{M_{iq,m}^{ee,*}}{\omega - (\Omega_m^{ee} - \epsilon_i - 2i\eta)}, \quad (121)
\end{aligned}$$

or, more compactly,

$$\begin{aligned} \Sigma_{pq}^{\text{pp}}(\omega) = & + \frac{1}{2} \sum_{am} \frac{\tilde{M}_{pa,m}^{\text{hh}} M_{aq,m}^{\text{hh}}}{\omega - (\Omega_m^{\text{hh}} - \epsilon_a + 2i\eta)} + \frac{1}{2} \sum_{ija} \frac{\tilde{M}_{qa,ij}^{\text{hh}} \langle pa||ij \rangle}{\omega - (\epsilon_i + \epsilon_j - \epsilon_a + 3i\eta)} \\ & + \frac{1}{2} \sum_{im} \frac{\tilde{M}_{pi,m}^{\text{ee}} M_{iq,m}^{\text{ee},*}}{\omega - (\Omega_m^{\text{ee}} - \epsilon_i - 2i\eta)} + \frac{1}{2} \sum_{iab} \frac{\tilde{M}_{qi,ab}^{\text{ee}} \langle pi||ab \rangle}{\omega - (\epsilon_a + \epsilon_b - \epsilon_i - 3i\eta)} \end{aligned} \quad (122)$$

with

$$\tilde{M}_{pa,m}^{\text{hh}} = \sum_{ij} \frac{\langle pa||ij \rangle M_{ij,m}^{\text{hh},*}}{\Omega_m^{\text{hh}} - \epsilon_i - \epsilon_j - i\eta} + \sum_{bc} \frac{\langle pa||bc \rangle M_{bc,m}^{\text{hh},*}}{\epsilon_b + \epsilon_c - \Omega_m^{\text{hh}} - 3i\eta} \quad (123a)$$

$$\tilde{M}_{qa,ij}^{\text{hh}} = \sum_m \frac{M_{ij,m}^{\text{ee}} M_{aq,m}^{\text{ee},*}}{\Omega_m^{\text{ee}} - \epsilon_i - \epsilon_j - 3i\eta} - \sum_m \frac{M_{ij,m}^{\text{hh},*} M_{aq,m}^{\text{hh}}}{\Omega_m^{\text{hh}} - \epsilon_i - \epsilon_j - i\eta} \quad (123b)$$

$$\tilde{M}_{pi,m}^{\text{ee}} = \sum_{ab} \frac{\langle pi||ab \rangle M_{ab,m}^{\text{ee}}}{\epsilon_a + \epsilon_b - \Omega_m^{\text{ee}} - i\eta} + \sum_{jk} \frac{\langle pi||jk \rangle M_{jk,m}^{\text{ee}}}{\Omega_m^{\text{ee}} - \epsilon_j - \epsilon_k - 3i\eta} \quad (123c)$$

$$\tilde{M}_{qi,ab}^{\text{ee}} = \sum_m \frac{M_{ab,m}^{\text{hh},*} M_{iq,m}^{\text{hh}}}{\epsilon_a + \epsilon_b - \Omega_m^{\text{hh}} - 3i\eta} - \sum_m \frac{M_{ab,m}^{\text{ee}} M_{iq,m}^{\text{ee},*}}{\epsilon_a + \epsilon_b - \Omega_m^{\text{ee}} - i\eta} \quad (123d)$$

Regarding the computational cost of constructing the pp self-energy, the same conclusions apply as for the eh contribution (see above).

### 3. Static self-energy

The static Hermitian self-energy used in the qsPA scheme is defined as

$$\Sigma_{pq}^{\text{qsPA}} = \Sigma_{pq}^{(2)} + \frac{\Sigma_{pq}^{\text{eh}} + \Sigma_{qp}^{\text{eh}}}{2} + \frac{\Sigma_{pq}^{\text{pp}} + \Sigma_{qp}^{\text{pp}}}{2}. \quad (124)$$

The second-order component reads

$$\begin{aligned} \Sigma_{pq}^{(2)} = & \frac{1}{2} \sum_{ija} \langle pa||ji \rangle \langle ji||qa \rangle \frac{\Delta_{paij} + \Delta_{qaij}}{\Delta_{paij}^2 + \Delta_{qaij}^2} \left[ 1 - e^{-s_{1b}(\Delta_{paij}^2 + \Delta_{qaij}^2)} \right] \\ & + \frac{1}{2} \sum_{iab} \langle pi||ba \rangle \langle ba||qi \rangle \frac{\Delta_{piab} + \Delta_{qiab}}{\Delta_{piab}^2 + \Delta_{qiab}^2} \left[ 1 - e^{-s_{1b}(\Delta_{piab}^2 + \Delta_{qiab}^2)} \right], \end{aligned} \quad (125)$$

where  $\Delta_{pqrs} = \epsilon_p + \epsilon_q - \epsilon_r - \epsilon_s$ . The static eh component is

$$\begin{aligned} \Sigma_{pq}^{\text{eh}} = & + \sum_{jn} \tilde{M}_{pj,n}^{\text{eh}} M_{qj,n}^{\text{eh},*} \frac{\Delta_{pjn} + \Delta_{qjn}}{\Delta_{pjn}^2 + \Delta_{qjn}^2} \left[ 1 - e^{-s_{1b}(\Delta_{pjn}^2 + \Delta_{qjn}^2)} \right] \\ & + \sum_{ija} \tilde{M}_{qj,ia}^{\text{eh}} \langle pa||ij \rangle \frac{\Delta_{paij} + \Delta_{qaij}}{\Delta_{paij}^2 + \Delta_{qaij}^2} \left[ 1 - e^{-s_{1b}(\Delta_{paij}^2 + \Delta_{qaij}^2)} \right] \\ & + \sum_{bn} \tilde{M}_{pb,n}^{\text{eh}} M_{bq,n}^{\text{eh}} \frac{\Delta_{pbn} + \Delta_{qbn}}{\Delta_{pbn}^2 + \Delta_{qbn}^2} \left[ 1 - e^{-s_{1b}(\Delta_{pbn}^2 + \Delta_{qbn}^2)} \right] \\ & + \sum_{iab} \tilde{M}_{qb,ia}^{\text{eh}} \langle pi||ab \rangle \frac{\Delta_{piab} + \Delta_{qiab}}{\Delta_{piab}^2 + \Delta_{qiab}^2} \left[ 1 - e^{-s_{1b}(\Delta_{piab}^2 + \Delta_{qiab}^2)} \right], \end{aligned} \quad (126)$$

where  $\Delta_{pjn} = \epsilon_p - \epsilon_j + \Omega_n^{\text{eh}}$  and  $\Delta_{pbn} = \epsilon_p - \epsilon_b - \Omega_n^{\text{eh}}$ . The  $\eta$  regularization in the intermediates is also replaced by an energy-dependent regularization. For example, the first term in Eq. (117) becomes

$$\sum_{ia} \frac{\langle pa||ij \rangle M_{ia,n}^{\text{eh}}}{\epsilon_a - \epsilon_i - \Omega_n^{\text{eh}}} \left[ 1 - e^{-2s_{1b}(\epsilon_a - \epsilon_i - \Omega_n^{\text{eh}})^2} \right]. \quad (127)$$

Finally, the static pp component is given by

$$\begin{aligned}
\Sigma_{pq}^{\text{pp}} = & + \frac{1}{2} \sum_{am} \tilde{M}_{pa,m}^{\text{hh}} M_{aq,m}^{\text{hh}} \frac{\Delta_{pam} + \Delta_{qam}}{\Delta_{pam}^2 + \Delta_{qam}^2} \left[ 1 - e^{-s_{1b}(\Delta_{pam}^2 + \Delta_{qam}^2)} \right] \\
& + \frac{1}{2} \sum_{ija} \tilde{M}_{qa,ij}^{\text{hh}} \langle pa || ij \rangle \frac{\Delta_{paij} + \Delta_{qaij}}{\Delta_{paij}^2 + \Delta_{qaij}^2} \left[ 1 - e^{-s_{1b}(\Delta_{paij}^2 + \Delta_{qaij}^2)} \right] \\
& + \frac{1}{2} \sum_{im} \tilde{M}_{pi,m}^{\text{ee}} M_{iq,m}^{\text{ee},*} \frac{\Delta_{pim} + \Delta_{qim}}{\Delta_{pim}^2 + \Delta_{qim}^2} \left[ 1 - e^{-s_{1b}(\Delta_{pim}^2 + \Delta_{qim}^2)} \right] \\
& + \frac{1}{2} \sum_{iab} \tilde{M}_{qi,ab}^{\text{ee}} \langle pi || ab \rangle \frac{\Delta_{piab} + \Delta_{qiab}}{\Delta_{piab}^2 + \Delta_{qiab}^2} \left[ 1 - e^{-s_{1b}(\Delta_{piab}^2 + \Delta_{qiab}^2)} \right],
\end{aligned} \tag{128}$$

where  $\Delta_{pam} = \epsilon_p - \epsilon_a - \Omega_m^{\text{hh}}$  and  $\Delta_{pim} = \epsilon_p - \epsilon_i - \Omega_m^{\text{ee}}$ . Once again, the  $\eta$  regularization in the intermediates is replaced by an energy-dependent regularization.

## VI. SPIN-ADAPTED PARQUET THEORY

This section presents a spin-adapted version of the equations necessary to implement the parquet approximation in a spatial orbital basis.

### A. Bethe-Salpeter equations

The eh-BSE for  $L$  and the pp-BSE for  $K$  have already been spin-adapted in Secs. II and III, respectively. Hence, the spin-adaptation of the two BSEs for the full two-body vertex can be easily deduced.

#### 1. Particle-particle vertices

For a pp vertex, the two incoming particles are labeled with indices 3 and 4, while the outgoing particles are labeled 1 and 2. Hence,  $\Gamma^{\text{pp}}(1\uparrow 2\uparrow; 3\uparrow 4\uparrow)$  corresponds to the scattering of a  $S_z = 1$  triplet pair of electrons and is already spin-adapted. The  $S_z = 0$  pairs of electrons, with spin  $\uparrow\downarrow$  or  $\downarrow\uparrow$ , are not eigenfunctions of the spin operator  $\hat{S}^2$ . As a consequence, in this basis,  $\Gamma^{\text{pp}}(1\uparrow 2\downarrow; 3\uparrow 4\downarrow)$  and  $\Gamma^{\text{pp}}(1\uparrow 2\downarrow; 3\downarrow 4\uparrow)$  are coupled. These two vertices can be spin-adapted by introducing the singlet and triplet vertices

$$\Gamma^{\text{s}}(\mathbf{r}_1 \mathbf{r}_2; \mathbf{r}_3 \mathbf{r}_4) = \Gamma^{\text{pp}}(1\uparrow 2\downarrow; 3\uparrow 4\downarrow) - \Gamma^{\text{pp}}(1\uparrow 2\downarrow; 3\downarrow 4\uparrow), \tag{129a}$$

$$\Gamma^{\text{t}}(\mathbf{r}_1 \mathbf{r}_2; \mathbf{r}_3 \mathbf{r}_4) = \Gamma^{\text{pp}}(1\uparrow 2\downarrow; 3\uparrow 4\downarrow) + \Gamma^{\text{pp}}(1\uparrow 2\downarrow; 3\downarrow 4\uparrow), \tag{129b}$$

which correspond to scattering of  $S_z = 0$  pairs of electrons with total spin  $S = 0$  for the singlet and  $S = 1$  for the triplet. In terms of these spin-adapted vertices, the pp-BSE becomes

$$F^{\text{s}}(\mathbf{r}_1 \mathbf{r}_2; \mathbf{r}_3 \mathbf{r}_4) = \Gamma^{\text{s}}(\mathbf{r}_1 \mathbf{r}_2; \mathbf{r}_3 \mathbf{r}_4) - \frac{1}{2} \Gamma^{\text{s}}(\mathbf{r}_1 \mathbf{r}_2; \mathbf{r}_1' \mathbf{r}_2') G(\mathbf{r}_1' \mathbf{r}_3') G(\mathbf{r}_2' \mathbf{r}_4') F^{\text{s}}(\mathbf{r}_3' \mathbf{r}_4'; \mathbf{r}_3 \mathbf{r}_4), \tag{130a}$$

$$F^{\text{t}}(\mathbf{r}_1 \mathbf{r}_2; \mathbf{r}_3 \mathbf{r}_4) = \Gamma^{\text{t}}(\mathbf{r}_1 \mathbf{r}_2; \mathbf{r}_3 \mathbf{r}_4) - \frac{1}{2} \Gamma^{\text{t}}(\mathbf{r}_1 \mathbf{r}_2; \mathbf{r}_1' \mathbf{r}_2') G(\mathbf{r}_1' \mathbf{r}_3') G(\mathbf{r}_2' \mathbf{r}_4') F^{\text{t}}(\mathbf{r}_3' \mathbf{r}_4'; \mathbf{r}_3 \mathbf{r}_4). \tag{130b}$$

These two spin-adapted vertices are referred to as the singlet  $\Gamma^{\text{s}}$  and triplet  $\Gamma^{\text{t}}$  vertices, respectively.

Once the Dyson equations above are expanded, this leads to the following expressions for the spin-adapted reducible vertices

$$\Phi^{\text{s}}(\mathbf{r}_1 \mathbf{r}_2; \mathbf{r}_3 \mathbf{r}_4) = -\frac{1}{2} \Gamma^{\text{s}}(\mathbf{r}_1 \mathbf{r}_2; \mathbf{r}_1' \mathbf{r}_2') K^{\text{s}}(\mathbf{r}_1' \mathbf{r}_2'; \mathbf{r}_3' \mathbf{r}_4') \Gamma^{\text{s}}(\mathbf{r}_3' \mathbf{r}_4'; \mathbf{r}_3 \mathbf{r}_4), \tag{131a}$$

$$\Phi^{\text{t}}(\mathbf{r}_1 \mathbf{r}_2; \mathbf{r}_3 \mathbf{r}_4) = -\frac{1}{2} \Gamma^{\text{t}}(\mathbf{r}_1 \mathbf{r}_2; \mathbf{r}_1' \mathbf{r}_2') K^{\text{t}}(\mathbf{r}_1' \mathbf{r}_2'; \mathbf{r}_3' \mathbf{r}_4') \Gamma^{\text{t}}(\mathbf{r}_3' \mathbf{r}_4'; \mathbf{r}_3 \mathbf{r}_4). \tag{131b}$$

These expressions have the same time-dependence as their non-spin-adapted version, and their Fourier transform is easily deduced

$$\Phi_P^s(\mathbf{r}_1\mathbf{r}_2; \mathbf{r}_3\mathbf{r}_4; \omega) = -\frac{1}{2}\Gamma_P^s(\mathbf{r}_1\mathbf{r}_2; \mathbf{r}_1'\mathbf{r}_2'; \omega = 0)K_P^s(\mathbf{r}_1'\mathbf{r}_2'; \mathbf{r}_3'\mathbf{r}_4'; \omega)\Gamma_P^s(\mathbf{r}_3'\mathbf{r}_4'; \mathbf{r}_3\mathbf{r}_4; \omega = 0), \quad (132a)$$

$$\Phi_P^t(\mathbf{r}_1\mathbf{r}_2; \mathbf{r}_3\mathbf{r}_4; \omega) = -\frac{1}{2}\Gamma_P^t(\mathbf{r}_1\mathbf{r}_2; \mathbf{r}_1'\mathbf{r}_2'; \omega = 0)K_P^t(\mathbf{r}_1'\mathbf{r}_2'; \mathbf{r}_3'\mathbf{r}_4'; \omega)\Gamma_P^t(\mathbf{r}_3'\mathbf{r}_4'; \mathbf{r}_3\mathbf{r}_4; \omega = 0). \quad (132b)$$

Here, the singlet and triplet irreducible vertices have been assumed to be static by analogy with the static kernel approximation discussed in the main text. Finally, once projected in the spatial orbital basis set, they are given by

$$(\Phi_P^s)_{pqrs}(\omega) = \sum_{\substack{t \leq u \\ v \leq w}} (i\Gamma_P^s)_{pqtu}(K_P^s)_{\overline{tuvw}}(\omega)(i\Gamma_P^s)_{vwrs}, \quad (133a)$$

$$(\Phi_P^t)_{pqrs}(\omega) = \sum_{\substack{t < u \\ v < w}} (i\Gamma_P^t)_{pqtu}(K_P^t)_{\overline{tuvw}}(\omega)(i\Gamma_P^t)_{vwrs}. \quad (133b)$$

## 2. Electron-hole vertices

For an eh vertex, the incoming electron and hole have indices 2 and 4, respectively. The corresponding outgoing particles have indices 3 and 1. The eh pair with spin  $S_z = -1$  is  $\downarrow\uparrow$  and the corresponding vertex  $\Gamma_{\uparrow\downarrow\downarrow\uparrow}^{\text{eh}}$  is already spin-adapted and decoupled from other vertices. On the other hand, the two remaining spin components  $F_{\uparrow\uparrow\uparrow\uparrow}$  and  $F_{\uparrow\downarrow\uparrow\downarrow}$  are coupled. They correspond to the scattering of a  $S_z = 0$  eh pair and can be spin-adapted through

$$\Gamma_d^{\text{eh}}(\mathbf{rt}_1\mathbf{rt}_2; \mathbf{rt}_3\mathbf{rt}_4) = \Gamma^{\text{eh}}(1\uparrow 2\uparrow; 3\uparrow 4\uparrow) + \Gamma^{\text{eh}}(1\uparrow 2\downarrow; 3\uparrow 4\downarrow), \quad (134a)$$

$$\Gamma_m^{\text{eh}}(\mathbf{rt}_1\mathbf{rt}_2; \mathbf{rt}_3\mathbf{rt}_4) = \Gamma^{\text{eh}}(1\uparrow 2\uparrow; 3\uparrow 4\uparrow) - \Gamma^{\text{eh}}(1\uparrow 2\downarrow; 3\uparrow 4\downarrow), \quad (134b)$$

leading to two decoupled BSE

$$F^d(\mathbf{rt}_1\mathbf{rt}_2; \mathbf{rt}_3\mathbf{rt}_4) = \Gamma^d(\mathbf{rt}_1\mathbf{rt}_2; \mathbf{rt}_3\mathbf{rt}_4) + \Gamma^d(\mathbf{rt}_1\mathbf{rt}_3'; \mathbf{rt}_3\mathbf{rt}_1')G(\mathbf{rt}_1'\mathbf{rt}_4')G(\mathbf{rt}_2'\mathbf{rt}_3')F^d(\mathbf{rt}_4'\mathbf{rt}_2; \mathbf{rt}_2'\mathbf{rt}_4), \quad (135a)$$

$$F^m(\mathbf{rt}_1\mathbf{rt}_2; \mathbf{rt}_3\mathbf{rt}_4) = \Gamma^m(\mathbf{rt}_1\mathbf{rt}_2; \mathbf{rt}_3\mathbf{rt}_4) + \Gamma^m(\mathbf{rt}_1\mathbf{rt}_3'; \mathbf{rt}_3\mathbf{rt}_1')G(\mathbf{rt}_1'\mathbf{rt}_4')G(\mathbf{rt}_2'\mathbf{rt}_3')F^m(\mathbf{rt}_4'\mathbf{rt}_2; \mathbf{rt}_2'\mathbf{rt}_4). \quad (135b)$$

These two spin-adapted vertices are referred to as the density  $\Gamma^d$  and magnetic  $\Gamma^m$  vertices, respectively.

Once the Dyson equations above are expanded, this leads to the following expressions of the spin-adapted reducible vertices

$$\Phi^d(\mathbf{rt}_1\mathbf{rt}_2; \mathbf{rt}_3\mathbf{rt}_4) = \Gamma^d(\mathbf{rt}_1\mathbf{rt}_3'; \mathbf{rt}_3\mathbf{rt}_1')L^d(\mathbf{rt}_1'\mathbf{rt}_2'; \mathbf{rt}_3'\mathbf{rt}_4')\Gamma^d(\mathbf{rt}_4'\mathbf{rt}_2; \mathbf{rt}_2'\mathbf{rt}_4), \quad (136a)$$

$$\Phi^m(\mathbf{rt}_1\mathbf{rt}_2; \mathbf{rt}_3\mathbf{rt}_4) = \Gamma^m(\mathbf{rt}_1\mathbf{rt}_3'; \mathbf{rt}_3\mathbf{rt}_1')L^m(\mathbf{rt}_1'\mathbf{rt}_2'; \mathbf{rt}_3'\mathbf{rt}_4')\Gamma^m(\mathbf{rt}_4'\mathbf{rt}_2; \mathbf{rt}_2'\mathbf{rt}_4). \quad (136b)$$

These expressions have the same time-dependence as their non-spin-adapted version, and their Fourier transform is easily deduced

$$\Phi^d(\mathbf{x}_1\mathbf{x}_2; \mathbf{x}_3\mathbf{x}_4; \omega) = \Gamma^d(\mathbf{x}_1\mathbf{x}_3'; \mathbf{x}_3\mathbf{x}_1'; \omega = 0)L^d(\mathbf{x}_1'\mathbf{x}_2'; \mathbf{x}_3'\mathbf{x}_4'; \omega)\Gamma^d(\mathbf{x}_4'\mathbf{x}_2; \mathbf{x}_2'\mathbf{x}_4; \omega = 0), \quad (137a)$$

$$\Phi^m(\mathbf{x}_1\mathbf{x}_2; \mathbf{x}_3\mathbf{x}_4; \omega) = \Gamma^m(\mathbf{x}_1\mathbf{x}_3'; \mathbf{x}_3\mathbf{x}_1'; \omega = 0)L^m(\mathbf{x}_1'\mathbf{x}_2'; \mathbf{x}_3'\mathbf{x}_4'; \omega)\Gamma^m(\mathbf{x}_4'\mathbf{x}_2; \mathbf{x}_2'\mathbf{x}_4; \omega = 0). \quad (137b)$$

Here, the density and magnetic irreducible vertices have been assumed to be static by analogy with the static kernel approximation discussed in the main text. Finally, once projected in the spatial orbital basis set, they are given by

$$(\Phi^d)_{pqrs}(\omega) = -\sum_{tuvw} (i\Gamma_{pqrt}^d)(L^d)_{tuvw}(\omega)(i\Gamma_{wqus}^d), \quad (138a)$$

$$(\Phi^m)_{pqrs}(\omega) = -\sum_{tuvw} (i\Gamma_{pqrt}^m)(L^m)_{tuvw}(\omega)(i\Gamma_{wqus}^m). \quad (138b)$$



## B. Irreducible vertices

The aim of this section is to express the spin-adapted irreducible vertices  $\Gamma^d, \Gamma^m, \Gamma^s$  and  $\Gamma^t$  in terms of the reducible ones.

### 1. Density channel

The density irreducible vertex is spin-adapted as

$$\begin{aligned}
& \Gamma^d(\mathbf{rt}_1\mathbf{rt}_2; \mathbf{rt}_3\mathbf{rt}_4) - \Lambda^d(\mathbf{rt}_1\mathbf{rt}_2; \mathbf{rt}_3\mathbf{rt}_4) \\
&= \Phi^{\text{eh}}(1\uparrow 2\uparrow; 3\uparrow 4\uparrow) + \Phi^{\text{eh}}(1\uparrow 2\downarrow; 3\uparrow 4\downarrow) + \Phi^{\text{pp}}(1\uparrow 2\uparrow; 3\uparrow 4\uparrow) + \Phi^{\text{pp}}(1\uparrow 2\downarrow; 3\uparrow 4\downarrow) \\
&= -\Phi^{\text{eh}}(1\uparrow 2\uparrow; 4\uparrow 3\uparrow) - \Phi^{\text{eh}}(1\uparrow 2\downarrow; 4\downarrow 3\uparrow) + \Phi^{\text{pp}}(1\uparrow 2\uparrow; 3\uparrow 4\uparrow) + \Phi^{\text{pp}}(1\uparrow 2\downarrow; 3\uparrow 4\downarrow) \\
&= -\Phi^{\text{eh}}(1\uparrow 2\uparrow; 4\uparrow 3\uparrow) - \Phi^{\text{m}}(\mathbf{rt}_1\mathbf{rt}_2; \mathbf{rt}_4\mathbf{rt}_3) + \Phi^{\text{t}}(\mathbf{rt}_1\mathbf{rt}_2; \mathbf{rt}_3\mathbf{rt}_4) + \Phi^{\text{pp}}(1\uparrow 2\downarrow; 3\uparrow 4\downarrow) \\
&= -\frac{1}{2}\Phi^d(\mathbf{rt}_1\mathbf{rt}_2; \mathbf{rt}_4\mathbf{rt}_3) - \frac{3}{2}\Phi^{\text{m}}(\mathbf{rt}_1\mathbf{rt}_2; \mathbf{rt}_4\mathbf{rt}_3) + \frac{3}{2}\Phi^{\text{t}}(\mathbf{rt}_1\mathbf{rt}_2; \mathbf{rt}_3\mathbf{rt}_4) + \frac{1}{2}\Phi^s(\mathbf{rt}_1\mathbf{rt}_2; \mathbf{rt}_3\mathbf{rt}_4),
\end{aligned} \tag{139}$$

and its static limit in a spatial-orbital basis set reads

$$\Gamma_{pqrs}^d = 2 \langle pq|rs \rangle - \langle pq|sr \rangle - \frac{1}{2}\Phi_{pqsr}^d - \frac{3}{2}\Phi_{pqsr}^{\text{m}} + \frac{1}{2}\Phi_{pqrs}^s + \frac{3}{2}\Phi_{pqrs}^{\text{t}}. \tag{140}$$

### 2. Magnetic channel

The magnetic irreducible vertex is spin-adapted as

$$\begin{aligned}
& \Gamma^{\text{m}}(\mathbf{rt}_1\mathbf{rt}_2; \mathbf{rt}_3\mathbf{rt}_4) - \Lambda^{\text{m}}(\mathbf{rt}_1\mathbf{rt}_2; \mathbf{rt}_3\mathbf{rt}_4) \\
&= \Phi^{\text{eh}}(1\uparrow 2\uparrow; 3\uparrow 4\uparrow) - \Phi^{\text{eh}}(1\uparrow 2\downarrow; 3\uparrow 4\downarrow) + \Phi^{\text{pp}}(1\uparrow 2\uparrow; 3\uparrow 4\uparrow) - \Phi^{\text{pp}}(1\uparrow 2\downarrow; 3\uparrow 4\downarrow) \\
&= -\Phi^{\text{eh}}(1\uparrow 2\uparrow; 4\uparrow 3\uparrow) + \Phi^{\text{eh}}(1\uparrow 2\downarrow; 4\downarrow 3\uparrow) + \Phi^{\text{pp}}(1\uparrow 2\uparrow; 3\uparrow 4\uparrow) - \Phi^{\text{pp}}(1\uparrow 2\downarrow; 3\uparrow 4\downarrow) \\
&= -\Phi^{\text{eh}}(1\uparrow 2\uparrow; 4\uparrow 3\uparrow) + \Phi^{\text{m}}(\mathbf{rt}_1\mathbf{rt}_2; \mathbf{rt}_4\mathbf{rt}_3) + \Phi^{\text{t}}(\mathbf{rt}_1\mathbf{rt}_2; \mathbf{rt}_3\mathbf{rt}_4) - \Phi^{\text{pp}}(1\uparrow 2\downarrow; 3\uparrow 4\downarrow) \\
&= -\frac{1}{2}\Phi^d(\mathbf{rt}_1\mathbf{rt}_2; \mathbf{rt}_4\mathbf{rt}_3) + \frac{1}{2}\Phi^{\text{m}}(\mathbf{rt}_1\mathbf{rt}_2; \mathbf{rt}_4\mathbf{rt}_3) + \frac{1}{2}\Phi^{\text{t}}(\mathbf{rt}_1\mathbf{rt}_2; \mathbf{rt}_3\mathbf{rt}_4) - \frac{1}{2}\Phi^s(\mathbf{rt}_1\mathbf{rt}_2; \mathbf{rt}_3\mathbf{rt}_4),
\end{aligned} \tag{141}$$

and its static limit in a spatial-orbital basis set reads

$$\Gamma_{pqrs}^{\text{m}} = -\langle pq|sr \rangle - \frac{1}{2}\Phi_{pqsr}^d + \frac{1}{2}\Phi_{pqsr}^{\text{m}} - \frac{1}{2}\Phi_{pqrs}^s + \frac{1}{2}\Phi_{pqrs}^{\text{t}}. \tag{142}$$

### 3. Singlet channel

The singlet irreducible vertex is spin-adapted as

$$\begin{aligned}
& \Gamma^s(\mathbf{rt}_1\mathbf{rt}_2; \mathbf{rt}_3\mathbf{rt}_4) - \Lambda^s(\mathbf{rt}_1\mathbf{rt}_2; \mathbf{rt}_3\mathbf{rt}_4) \\
&= \Phi^{\text{eh}}(1\uparrow 2\downarrow; 3\uparrow 4\downarrow) - \Phi^{\text{eh}}(1\uparrow 2\downarrow; 3\downarrow 4\uparrow) + \Phi^{\text{eh}}(1\uparrow 2\downarrow; 3\uparrow 4\downarrow) - \Phi^{\text{eh}}(1\uparrow 2\downarrow; 3\downarrow 4\uparrow) \\
&= \Phi^{\text{eh}}(1\uparrow 2\downarrow; 3\uparrow 4\downarrow) - \Phi^{\text{eh}}(1\uparrow 2\downarrow; 3\downarrow 4\uparrow) - \Phi^{\text{eh}}(1\uparrow 2\downarrow; 4\downarrow 3\uparrow) + \Phi^{\text{eh}}(1\uparrow 2\downarrow; 4\uparrow 3\downarrow) \\
&= \Phi^{\text{eh}}(1\uparrow 2\downarrow; 3\uparrow 4\downarrow) - \Phi^{\text{m}}(\mathbf{rt}_1\mathbf{rt}_2; \mathbf{rt}_3\mathbf{rt}_4) - \Phi^{\text{m}}(\mathbf{rt}_1\mathbf{rt}_2; \mathbf{rt}_4\mathbf{rt}_3) + \Phi^{\text{eh}}(1\uparrow 2\downarrow; 4\uparrow 3\downarrow) \\
&= \frac{1}{2}\Phi^d(\mathbf{rt}_1\mathbf{rt}_2; \mathbf{rt}_3\mathbf{rt}_4) - \frac{3}{2}\Phi^{\text{m}}(\mathbf{rt}_1\mathbf{rt}_2; \mathbf{rt}_3\mathbf{rt}_4) - \frac{3}{2}\Phi^{\text{m}}(\mathbf{rt}_1\mathbf{rt}_2; \mathbf{rt}_4\mathbf{rt}_3) + \frac{1}{2}\Phi^d(\mathbf{rt}_1\mathbf{rt}_2; \mathbf{rt}_4\mathbf{rt}_3),
\end{aligned} \tag{143}$$

and its static limit in a spatial-orbital basis set reads

$$\Gamma_{pqrs}^s = \langle pq|rs \rangle + \langle pq|sr \rangle + \frac{1}{2}\Phi_{pqrs}^d - \frac{3}{2}\Phi_{pqrs}^{\text{m}} + \frac{1}{2}\Phi_{pqsr}^d - \frac{3}{2}\Phi_{pqsr}^{\text{m}}. \tag{144}$$

#### 4. Triplet channel

The triplet irreducible vertex is spin-adapted as

$$\begin{aligned}
\Gamma^t(\mathbf{rt}_1\mathbf{rt}_2; \mathbf{rt}_3\mathbf{rt}_4) - \Lambda_t(\mathbf{rt}_1\mathbf{rt}_2; \mathbf{rt}_3\mathbf{rt}_4) \\
= \Phi^{\text{eh}}(1_\uparrow 2_\downarrow; 3_\uparrow 4_\downarrow) + \Phi^{\text{eh}}(1_\uparrow 2_\downarrow; 3_\downarrow 4_\uparrow) + \Phi^{\overline{\text{eh}}}(1_\uparrow 2_\downarrow; 3_\uparrow 4_\downarrow) + \Phi^{\overline{\text{eh}}}(1_\uparrow 2_\downarrow; 3_\downarrow 4_\uparrow) \\
= \Phi^{\text{eh}}(1_\uparrow 2_\downarrow; 3_\uparrow 4_\downarrow) + \Phi^{\text{eh}}(1_\uparrow 2_\downarrow; 3_\downarrow 4_\uparrow) - \Phi^{\text{eh}}(1_\uparrow 2_\downarrow; 4_\downarrow 3_\uparrow) - \Phi^{\text{eh}}(1_\uparrow 2_\downarrow; 4_\uparrow 3_\downarrow) \\
= \Phi^{\text{eh}}(1_\uparrow 2_\downarrow; 3_\uparrow 4_\downarrow) + \Phi^{\text{m}}(\mathbf{rt}_1\mathbf{rt}_2; \mathbf{rt}_3\mathbf{rt}_4) - \Phi^{\text{m}}(\mathbf{rt}_1\mathbf{rt}_2; \mathbf{rt}_4\mathbf{rt}_3) - \Phi^{\text{eh}}(1_\uparrow 2_\downarrow; 4_\uparrow 3_\downarrow) \\
= \frac{1}{2}\Phi^{\text{d}}(\mathbf{rt}_1\mathbf{rt}_2; \mathbf{rt}_3\mathbf{rt}_4) + \frac{1}{2}\Phi^{\text{m}}(\mathbf{rt}_1\mathbf{rt}_2; \mathbf{rt}_3\mathbf{rt}_4) - \frac{1}{2}\Phi^{\text{m}}(\mathbf{rt}_1\mathbf{rt}_2; \mathbf{rt}_4\mathbf{rt}_3) - \frac{1}{2}\Phi^{\text{d}}(\mathbf{rt}_1\mathbf{rt}_2; \mathbf{rt}_4\mathbf{rt}_3),
\end{aligned} \tag{145}$$

and its static limit in a spatial-orbital basis set reads

$$\Gamma_{pqrs}^{\text{m}} = \langle pq|rs\rangle - \langle pq|sr\rangle + \frac{1}{2}\Phi_{pqrs}^{\text{d}} + \frac{1}{2}\Phi_{pqrs}^{\text{m}} - \frac{1}{2}\Phi_{pqsr}^{\text{d}} - \frac{1}{2}\Phi_{pqsr}^{\text{m}}. \tag{146}$$

#### C. Self-energy

It has been shown in the main manuscript that the correlation part of the self-energy can be expressed in terms of  $\Phi^{\text{eh}}$  and  $\Phi^{\text{pp}}$ . The aim of this section is to express  $\Sigma_{\text{c}}$  in terms of the spin-adapted reducible vertices  $\Phi^{\text{d}}$ ,  $\Phi^{\text{m}}$ ,  $\Phi^{\text{s}}$  and  $\Phi^{\text{t}}$ .

##### 1. eh self-energy

The spin-adaptation of the eh contribution reads

$$\begin{aligned}
\Sigma^{\text{eh}}(1_\uparrow 1'_\uparrow) &= -i \sum_{\substack{\sigma_2\sigma_3\sigma_4 \\ \sigma_2'\sigma_3'\sigma_4'}} \bar{v}(1_\uparrow 2_{\sigma_2}; 3'_{\sigma_3'} 2'_{\sigma_2'}) G(3'_{\sigma_3'} 3_{\sigma_3}) G(4'_{\sigma_4'} 2_{\sigma_2}) G(2'_{\sigma_2'} 4_{\sigma_4}) \Phi^{\text{eh}}(3_{\sigma_3} 4_{\sigma_4}; 4'_{\sigma_4'} 1'_\uparrow) \\
&= -i \sum_{\sigma_2\sigma_3\sigma_4} \bar{v}(1_\uparrow 2_{\sigma_2}; 3'_{\sigma_3} 2'_{\sigma_4}) G(\mathbf{rt}_3'\mathbf{rt}_3) G(\mathbf{rt}_4'\mathbf{rt}_2) G(\mathbf{rt}_2'\mathbf{rt}_4) \Phi^{\text{eh}}(3_{\sigma_3} 4_{\sigma_4}; 4'_{\sigma_2} 1'_\uparrow) \\
&= -i \sum_{\sigma_2\sigma_3} \bar{v}(1_\uparrow 2_{\sigma_2}; 3'_{\sigma_3} 2'_\uparrow) G(\mathbf{rt}_3'\mathbf{rt}_3) G(\mathbf{rt}_4'\mathbf{rt}_2) G(\mathbf{rt}_2'\mathbf{rt}_4) \Phi^{\text{eh}}(3_{\sigma_3} 4_\uparrow; 4'_{\sigma_2} 1'_\uparrow) \\
&\quad - i \sum_{\sigma_2\sigma_3} \bar{v}(1_\uparrow 2_{\sigma_2}; 3'_{\sigma_3} 2'_\downarrow) G(\mathbf{rt}_3'\mathbf{rt}_3) G(\mathbf{rt}_4'\mathbf{rt}_2) G(\mathbf{rt}_2'\mathbf{rt}_4) \Phi^{\text{eh}}(3_{\sigma_3} 4_\downarrow; 4'_{\sigma_2} 1'_\uparrow) \\
&= -i\bar{v}(1_\uparrow 2_\uparrow; 3'_\uparrow 2'_\uparrow) G(\mathbf{rt}_3'\mathbf{rt}_3) G(\mathbf{rt}_4'\mathbf{rt}_2) G(\mathbf{rt}_2'\mathbf{rt}_4) \Phi^{\text{eh}}(3_\uparrow 4_\uparrow; 4'_\uparrow 1'_\uparrow) \\
&\quad - i\bar{v}(1_\uparrow 2_\downarrow; 3'_\downarrow 2'_\uparrow) G(\mathbf{rt}_3'\mathbf{rt}_3) G(\mathbf{rt}_4'\mathbf{rt}_2) G(\mathbf{rt}_2'\mathbf{rt}_4) \Phi^{\text{eh}}(3_\downarrow 4_\uparrow; 4'_\downarrow 1'_\uparrow) \\
&\quad - i\bar{v}(1_\uparrow 2_\downarrow; 3'_\downarrow 2'_\downarrow) G(\mathbf{rt}_3'\mathbf{rt}_3) G(\mathbf{rt}_4'\mathbf{rt}_2) G(\mathbf{rt}_2'\mathbf{rt}_4) \Phi^{\text{eh}}(3_\downarrow 4_\downarrow; 4'_\downarrow 1'_\uparrow) \\
&= -\frac{i}{2} \bar{v}(\mathbf{rt}_1\mathbf{rt}_2; \mathbf{rt}_3'\mathbf{rt}_2') G(\mathbf{rt}_3'\mathbf{rt}_3) G(\mathbf{rt}_4'\mathbf{rt}_2) G(\mathbf{rt}_2'\mathbf{rt}_4) [\Phi^{\text{d}}(\mathbf{rt}_3\mathbf{rt}_4; \mathbf{rt}_4'\mathbf{rt}_1') + \Phi^{\text{m}}(\mathbf{rt}_3\mathbf{rt}_4; \mathbf{rt}_4'\mathbf{rt}_1')] \\
&\quad + \frac{i}{2} v(\mathbf{rt}_1\mathbf{rt}_2; \mathbf{rt}_2'\mathbf{rt}_3') G(\mathbf{rt}_3'\mathbf{rt}_3) G(\mathbf{rt}_4'\mathbf{rt}_2) G(\mathbf{rt}_2'\mathbf{rt}_4) [\Phi^{\text{d}}(\mathbf{rt}_3\mathbf{rt}_4; \mathbf{rt}_4'\mathbf{rt}_1') - \Phi^{\text{m}}(\mathbf{rt}_3\mathbf{rt}_4; \mathbf{rt}_4'\mathbf{rt}_1')] \\
&\quad - i v(\mathbf{rt}_1\mathbf{rt}_2; \mathbf{rt}_3'\mathbf{rt}_2') G(\mathbf{rt}_3'\mathbf{rt}_3) G(\mathbf{rt}_4'\mathbf{rt}_2) G(\mathbf{rt}_2'\mathbf{rt}_4) \Phi^{\text{m}}(\mathbf{rt}_3\mathbf{rt}_4; \mathbf{rt}_4'\mathbf{rt}_1') \\
&= \Sigma^{\text{d}}(\mathbf{rt}_1\mathbf{rt}_1') + \Sigma^{\text{m}}(\mathbf{rt}_1\mathbf{rt}_1').
\end{aligned} \tag{147}$$

The density and magnetic components of the self-energy are defined as

$$\Sigma^{\text{d}}(\mathbf{rt}_1\mathbf{rt}_1') = -\frac{i}{2} [v(\mathbf{rt}_1\mathbf{rt}_2; \mathbf{rt}_3'\mathbf{rt}_2') - 2v(\mathbf{rt}_1\mathbf{rt}_2; \mathbf{rt}_2'\mathbf{rt}_3')] G(\mathbf{rt}_3'\mathbf{rt}_3) G(\mathbf{rt}_4'\mathbf{rt}_2) G(\mathbf{rt}_2'\mathbf{rt}_4) \Phi^{\text{d}}(\mathbf{rt}_3\mathbf{rt}_4; \mathbf{rt}_4'\mathbf{rt}_1'), \tag{148a}$$

$$\Sigma^{\text{m}}(\mathbf{rt}_1\mathbf{rt}_1') = -\frac{3i}{2} v(\mathbf{rt}_1\mathbf{rt}_2; \mathbf{rt}_3'\mathbf{rt}_2') G(\mathbf{rt}_3'\mathbf{rt}_3) G(\mathbf{rt}_4'\mathbf{rt}_2) G(\mathbf{rt}_2'\mathbf{rt}_4) \Phi^{\text{m}}(\mathbf{rt}_3\mathbf{rt}_4; \mathbf{rt}_4'\mathbf{rt}_1'). \tag{148b}$$

It can be shown similarly that  $\Sigma^{\text{eh}}(1_\uparrow 1'_\downarrow)$  is zero.

## 2. *pp* self-energy

The spin-adaptation of the *pp* contribution reads

$$\begin{aligned}
\Sigma^{\text{PP}}(1_\uparrow 1'_\uparrow) &= -\frac{i}{2} \sum_{\substack{\sigma_2 \sigma_3 \sigma_4 \\ \sigma_2' \sigma_3' \sigma_4'}} \bar{v}(1_\uparrow 2_{\sigma_2}; 3'_{\sigma_3'} 2'_{\sigma_2'}) G(3'_{\sigma_3'} 3_{\sigma_3}) G(4'_{\sigma_4'} 2_{\sigma_2}) G(2'_{\sigma_2'} 4_{\sigma_4}) \Phi^{\text{PP}}(3_{\sigma_3} 4_{\sigma_4}; 4'_{\sigma_4'} 1'_\uparrow) \\
&= -\frac{i}{2} \sum_{\sigma_2 \sigma_3 \sigma_4} \bar{v}(1_\uparrow 2_{\sigma_2}; 3'_{\sigma_3} 2'_{\sigma_4}) G(\mathbf{rt}_3' \mathbf{rt}_3) G(\mathbf{rt}_4' \mathbf{rt}_2) G(\mathbf{rt}_2' \mathbf{rt}_4) \Phi^{\text{PP}}(3_{\sigma_3} 4_{\sigma_4}; 4'_{\sigma_4'} 1'_\uparrow) \\
&= -\frac{i}{2} \sum_{\sigma_2 \sigma_3} \bar{v}(1_\uparrow 2_{\sigma_2}; 3'_{\sigma_3} 2'_\uparrow) G(\mathbf{rt}_3' \mathbf{rt}_3) G(\mathbf{rt}_4' \mathbf{rt}_2) G(\mathbf{rt}_2' \mathbf{rt}_4) \Phi^{\text{PP}}(3_{\sigma_3} 4_\uparrow; 4'_{\sigma_2} 1'_\uparrow) \\
&\quad - \frac{i}{2} \sum_{\sigma_2 \sigma_3} \bar{v}(1_\uparrow 2_{\sigma_2}; 3'_{\sigma_3} 2'_\downarrow) G(\mathbf{rt}_3' \mathbf{rt}_3) G(\mathbf{rt}_4' \mathbf{rt}_2) G(\mathbf{rt}_2' \mathbf{rt}_4) \Phi^{\text{PP}}(3_{\sigma_3} 4_\downarrow; 4'_{\sigma_2} 1'_\uparrow) \\
&= -\frac{i}{2} \bar{v}(1_\uparrow 2_\uparrow; 3'_\uparrow 2'_\uparrow) G(\mathbf{rt}_3' \mathbf{rt}_3) G(\mathbf{rt}_4' \mathbf{rt}_2) G(\mathbf{rt}_2' \mathbf{rt}_4) \Phi^{\text{PP}}(3_\uparrow 4_\uparrow; 4'_\uparrow 1'_\uparrow) \\
&\quad - \frac{i}{2} \bar{v}(1_\uparrow 2_\downarrow; 3'_\downarrow 2'_\uparrow) G(\mathbf{rt}_3' \mathbf{rt}_3) G(\mathbf{rt}_4' \mathbf{rt}_2) G(\mathbf{rt}_2' \mathbf{rt}_4) \Phi^{\text{PP}}(3_\downarrow 4_\uparrow; 4'_\downarrow 1'_\uparrow) \\
&\quad - \frac{i}{2} \bar{v}(1_\uparrow 2_\downarrow; 3'_\uparrow 2'_\downarrow) G(\mathbf{rt}_3' \mathbf{rt}_3) G(\mathbf{rt}_4' \mathbf{rt}_2) G(\mathbf{rt}_2' \mathbf{rt}_4) \Phi^{\text{PP}}(3_\uparrow 4_\downarrow; 4'_\downarrow 1'_\uparrow) \\
&= -\frac{i}{2} \bar{v}(\mathbf{rt}_1 \mathbf{rt}_2; \mathbf{rt}_3' \mathbf{rt}_2') G(\mathbf{rt}_3' \mathbf{rt}_3) G(\mathbf{rt}_4' \mathbf{rt}_2) G(\mathbf{rt}_2' \mathbf{rt}_4) \Phi^{\text{t}}(\mathbf{rt}_3 \mathbf{rt}_4; \mathbf{rt}_4' \mathbf{rt}_1') \\
&\quad + \frac{i}{4} v(\mathbf{rt}_1 \mathbf{rt}_2; \mathbf{rt}_2' \mathbf{rt}_3') G(\mathbf{rt}_3' \mathbf{rt}_3) G(\mathbf{rt}_4' \mathbf{rt}_2) G(\mathbf{rt}_2' \mathbf{rt}_4) [\Phi^{\text{t}}(\mathbf{rt}_3 \mathbf{rt}_4; \mathbf{rt}_4' \mathbf{rt}_1') + \Phi^{\text{s}}(\mathbf{rt}_3 \mathbf{rt}_4; \mathbf{rt}_4' \mathbf{rt}_1')] \\
&\quad - \frac{i}{4} v(\mathbf{rt}_1 \mathbf{rt}_2; \mathbf{rt}_3' \mathbf{rt}_2') G(\mathbf{rt}_3' \mathbf{rt}_3) G(\mathbf{rt}_4' \mathbf{rt}_2) G(\mathbf{rt}_2' \mathbf{rt}_4) [\Phi^{\text{t}}(\mathbf{rt}_3 \mathbf{rt}_4; \mathbf{rt}_4' \mathbf{rt}_1') - \Phi^{\text{s}}(\mathbf{rt}_3 \mathbf{rt}_4; \mathbf{rt}_4' \mathbf{rt}_1')] \\
&= \Sigma^{\text{s}}(\mathbf{rt}_1 \mathbf{rt}_1') + \Sigma^{\text{t}}(\mathbf{rt}_1 \mathbf{rt}_1').
\end{aligned} \tag{149}$$

The singlet and triplet components of the self-energy are defined as

$$\Sigma^{\text{s}}(\mathbf{rt}_1 \mathbf{rt}_1') = +\frac{i}{4} [v(\mathbf{rt}_1 \mathbf{rt}_2; \mathbf{rt}_3' \mathbf{rt}_2') + v(\mathbf{rt}_1 \mathbf{rt}_2; \mathbf{rt}_2' \mathbf{rt}_3')] G(\mathbf{rt}_3' \mathbf{rt}_3) G(\mathbf{rt}_4' \mathbf{rt}_2) G(\mathbf{rt}_2' \mathbf{rt}_4) \Phi^{\text{s}}(\mathbf{rt}_3 \mathbf{rt}_4; \mathbf{rt}_4' \mathbf{rt}_1'), \tag{150a}$$

$$\Sigma^{\text{t}}(\mathbf{rt}_1 \mathbf{rt}_1') = -\frac{3i}{4} [v(\mathbf{rt}_1 \mathbf{rt}_2; \mathbf{rt}_3' \mathbf{rt}_2') - v(\mathbf{rt}_1 \mathbf{rt}_2; \mathbf{rt}_2' \mathbf{rt}_3')] G(\mathbf{rt}_3' \mathbf{rt}_3) G(\mathbf{rt}_4' \mathbf{rt}_2) G(\mathbf{rt}_2' \mathbf{rt}_4) \Phi^{\text{t}}(\mathbf{rt}_3 \mathbf{rt}_4; \mathbf{rt}_4' \mathbf{rt}_1'). \tag{150b}$$

It can be shown similarly that  $\Sigma^{\text{PP}}(1_\uparrow 1'_\downarrow)$  is zero.

## 3. *Fourier transform*

We can easily deduce the Fourier transform of the spin-adapted self-energy using the results of the spin-orbital section

$$\Sigma^{\text{d}}(\mathbf{r}_1 \mathbf{r}_{1'}; \omega) = -\frac{i}{2(2\pi)^2} \left[ v(\mathbf{r}_1 \mathbf{r}_2; \mathbf{r}_3' \mathbf{r}_{2'}) - 2v(\mathbf{r}_1 \mathbf{r}_2; \mathbf{r}_2' \mathbf{r}_{3'}) \right] \tag{151a}$$

$$\begin{aligned} &\int d(\omega_1 \omega_2) G(\mathbf{r}_3' \mathbf{r}_3; \omega_1) G(\mathbf{r}_4' \mathbf{r}_2; \omega_2) G(\mathbf{r}_2' \mathbf{r}_4; \omega - \omega_1 + \omega_2) \Phi^{\text{d}}(\mathbf{r}_3 \mathbf{r}_4; \mathbf{r}_4' \mathbf{r}_{1'}; \omega_2 - \omega_1), \\ \Sigma^{\text{m}}(\mathbf{r}_1 \mathbf{r}_{1'}; \omega) &= -\frac{3i}{2(2\pi)^2} \left[ v(\mathbf{r}_1 \mathbf{r}_2; \mathbf{r}_3' \mathbf{r}_{2'}) \right] \end{aligned} \tag{151b}$$

$$\begin{aligned} &\int d(\omega_1 \omega_2) G(\mathbf{r}_3' \mathbf{r}_3; \omega_1) G(\mathbf{r}_4' \mathbf{r}_2; \omega_2) G(\mathbf{r}_2' \mathbf{r}_4; \omega - \omega_1 + \omega_2) \Phi^{\text{m}}(\mathbf{r}_3 \mathbf{r}_4; \mathbf{r}_4' \mathbf{r}_{1'}; \omega_2 - \omega_1), \\ \Sigma^{\text{s}}(\mathbf{r}_1 \mathbf{r}_{1'}; \omega) &= \frac{i}{4(2\pi)^2} \left[ v(\mathbf{r}_1 \mathbf{r}_2; \mathbf{r}_3' \mathbf{r}_{2'}) + v(\mathbf{r}_1 \mathbf{r}_2; \mathbf{r}_2' \mathbf{r}_{3'}) \right] \end{aligned} \tag{151c}$$

$$\int d(\omega_1 \omega_2) G(\mathbf{r}_3' \mathbf{r}_3; \omega_1) G(\mathbf{r}_4' \mathbf{r}_2; \omega_2) G(\mathbf{r}_2' \mathbf{r}_4; \omega - \omega_1 + \omega_2) \Phi^{\text{s}}(\mathbf{r}_3 \mathbf{r}_4; \mathbf{r}_4' \mathbf{r}_{1'}; \omega_2 + \omega),$$

$$\Sigma^t(\mathbf{r}_1\mathbf{r}_1';\omega) = -\frac{3i}{4(2\pi)^2} \left[ v(\mathbf{r}_1\mathbf{r}_2;\mathbf{r}_3'\mathbf{r}_2') - v(\mathbf{r}_1\mathbf{r}_2;\mathbf{r}_2'\mathbf{r}_3') \right] \int d\omega_1 d\omega_2 G(\mathbf{r}_3'\mathbf{r}_3;\omega_1) G(\mathbf{r}_4'\mathbf{r}_2;\omega_2) G(\mathbf{r}_2'\mathbf{r}_4;\omega - \omega_1 + \omega_2) \Phi_P^t(\mathbf{r}_3\mathbf{r}_4;\mathbf{r}_4'\mathbf{r}_1';\omega_2 + \omega). \quad (151d)$$

#### 4. Self-energy expressions

The above integrals can be computed analytically in a similar way to the spin-orbital ones. The expression of the density part of the self-energy in a spatial orbital basis is

$$\begin{aligned} \Sigma_{pq}^d(\omega) = & + \frac{1}{2} \sum_{ij an} \frac{(\langle pa|ij\rangle - 2\langle pa|ji\rangle)}{\epsilon_a - \epsilon_i - \Omega_n^d - i\eta} \frac{M_{ia,n}^d M_{qj,n}^{d,*}}{\omega - (\epsilon_j - \Omega_n^d + 2i\eta)} - \frac{1}{2} \sum_{ij an} \frac{(\langle pa|ij\rangle - 2\langle pa|ji\rangle)}{\epsilon_a - \epsilon_i - \Omega_n^d - i\eta} \frac{M_{ia,n}^d M_{qj,n}^{d,*}}{\omega - (\epsilon_i + \epsilon_j - \epsilon_a + 3i\eta)} \\ & + \frac{1}{2} \sum_{ij an} \frac{(\langle pa|ij\rangle - 2\langle pa|ji\rangle)}{\epsilon_a - \epsilon_i + \Omega_n^d - 3i\eta} \frac{M_{ai,n}^{d,*} M_{jq,n}^d}{\omega - (\epsilon_i + \epsilon_j - \epsilon_a + 3i\eta)} + \frac{1}{2} \sum_{ij an} \frac{(\langle pi|aj\rangle - 2\langle pi|ja\rangle)}{\epsilon_a - \epsilon_i + \Omega_n^d - 3i\eta} \frac{M_{ai,n}^d M_{qj,n}^{d,*}}{\omega - (\epsilon_j - \Omega_n^d + 2i\eta)} \\ & + \frac{1}{2} \sum_{iabn} \frac{(\langle pi|ab\rangle - 2\langle pi|ba\rangle)}{\epsilon_a - \epsilon_i - \Omega_n^d - i\eta} \frac{M_{ia,n}^{d,*} M_{bq,n}^d}{\omega - (\epsilon_b + \Omega_n^d - 2i\eta)} - \frac{1}{2} \sum_{iabn} \frac{(\langle pi|ab\rangle - 2\langle pi|ba\rangle)}{\epsilon_a - \epsilon_i - \Omega_n^d - i\eta} \frac{M_{ia,n}^{d,*} M_{bq,n}^d}{\omega - (\epsilon_a + \epsilon_b - \epsilon_i - 3i\eta)} \\ & + \frac{1}{2} \sum_{iabn} \frac{(\langle pi|ab\rangle - 2\langle pi|ba\rangle)}{\epsilon_a - \epsilon_i + \Omega_n^d - 3i\eta} \frac{M_{ai,n}^d M_{qb,n}^{d,*}}{\omega - (\epsilon_a + \epsilon_b - \epsilon_i - 3i\eta)} + \frac{1}{2} \sum_{iabn} \frac{(\langle pa|ib\rangle - 2\langle pa|bi\rangle)}{\epsilon_a - \epsilon_i + \Omega_n^d - 3i\eta} \frac{M_{ai,n}^{d,*} M_{bq,n}^d}{\omega - (\epsilon_b + \Omega_n^d - 2i\eta)}. \end{aligned} \quad (152)$$

The expression of the magnetic part of the self-energy in a spatial orbital basis is

$$\begin{aligned} \Sigma_{pq}^m(\omega) = & + \frac{3}{2} \sum_{ij an} \frac{\langle pa|ij\rangle}{\epsilon_a - \epsilon_i - \Omega_n^m - i\eta} \frac{M_{ia,n}^m M_{qj,n}^{m,*}}{\omega - (\epsilon_j - \Omega_n^m + 2i\eta)} - \frac{3}{2} \sum_{ij an} \frac{\langle pa|ij\rangle}{\epsilon_a - \epsilon_i - \Omega_n^m - i\eta} \frac{M_{ia,n}^m M_{qj,n}^{m,*}}{\omega - (\epsilon_i + \epsilon_j - \epsilon_a + 3i\eta)} \\ & + \frac{3}{2} \sum_{ij an} \frac{\langle pa|ij\rangle}{\epsilon_a - \epsilon_i + \Omega_n^m - 3i\eta} \frac{M_{ai,n}^{m,*} M_{jq,n}^m}{\omega - (\epsilon_i + \epsilon_j - \epsilon_a + 3i\eta)} + \frac{3}{2} \sum_{ij an} \frac{\langle pi|aj\rangle}{\epsilon_a - \epsilon_i + \Omega_n^m - 3i\eta} \frac{M_{ai,n}^m M_{qj,n}^{m,*}}{\omega - (\epsilon_j - \Omega_n^m + 2i\eta)} \\ & + \frac{3}{2} \sum_{iabn} \frac{\langle pi|ab\rangle}{\epsilon_a - \epsilon_i - \Omega_n^m - i\eta} \frac{M_{ia,n}^{m,*} M_{bq,n}^m}{\omega - (\epsilon_b + \Omega_n^m - 2i\eta)} - \frac{3}{2} \sum_{iabn} \frac{\langle pi|ab\rangle}{\epsilon_a - \epsilon_i - \Omega_n^m - i\eta} \frac{M_{ia,n}^{m,*} M_{bq,n}^m}{\omega - (\epsilon_a + \epsilon_b - \epsilon_i - 3i\eta)} \\ & + \frac{3}{2} \sum_{iabn} \frac{\langle pi|ab\rangle}{\epsilon_a - \epsilon_i + \Omega_n^m - 3i\eta} \frac{M_{ai,n}^m M_{qb,n}^{m,*}}{\omega - (\epsilon_a + \epsilon_b - \epsilon_i - 3i\eta)} + \frac{3}{2} \sum_{iabn} \frac{\langle pa|ib\rangle}{\epsilon_a - \epsilon_i + \Omega_n^m - 3i\eta} \frac{M_{ai,n}^{m,*} M_{bq,n}^m}{\omega - (\epsilon_b + \Omega_n^m - 2i\eta)}. \end{aligned} \quad (153)$$

The expression of the singlet part of the self-energy in a spatial orbital basis is

$$\begin{aligned} \Sigma_{pq}^s(\omega) = & - \frac{1}{4} \sum_{ajkm} \frac{(\langle pa|jk\rangle + \langle pa|kj\rangle)}{\Omega_m^{hh,s} - \epsilon_j - \epsilon_k - i\eta} \frac{M_{jk,m}^{hh,s,*} M_{aq,m}^{hh,s}}{\omega - (\Omega_m^{hh,s} - \epsilon_a + 2i\eta)} + \frac{1}{4} \sum_{ajkm} \frac{(\langle pa|jk\rangle + \langle pa|kj\rangle)}{\Omega_m^{hh,s} - \epsilon_j - \epsilon_k - i\eta} \frac{M_{jk,m}^{hh,s,*} M_{aq,m}^{hh,s}}{\omega - (\epsilon_j + \epsilon_k - \epsilon_a + 3i\eta)} \\ & - \frac{1}{4} \sum_{ajkm} \frac{(\langle pa|jk\rangle + \langle pa|kj\rangle)}{\Omega_m^{ee,s} - \epsilon_j - \epsilon_k - 3i\eta} \frac{M_{jk,m}^{ee,s,*} M_{aq,m}^{ee,s}}{\omega - (\epsilon_j + \epsilon_k - \epsilon_a + 3i\eta)} - \frac{1}{4} \sum_{abcm} \frac{(\langle pa|bc\rangle + \langle pa|cb\rangle)}{\epsilon_b + \epsilon_c - \Omega_m^{hh,s} - 3i\eta} \frac{M_{bc,m}^{hh,s,*} M_{aq,m}^{hh,s}}{\omega - (\Omega_m^{hh,s} - \epsilon_a + 2i\eta)} \\ & - \frac{1}{4} \sum_{ibcm} \frac{(\langle pi|bc\rangle + \langle pi|cb\rangle)}{\epsilon_b + \epsilon_c - \Omega_m^{ee,s} - i\eta} \frac{M_{bc,m}^{ee,s,*} M_{iq,m}^{ee,s}}{\omega - (\Omega_m^{ee,s} - \epsilon_i - 2i\eta)} + \frac{1}{4} \sum_{ibcm} \frac{(\langle pi|bc\rangle + \langle pi|cb\rangle)}{\epsilon_b + \epsilon_c - \Omega_m^{ee,s} - i\eta} \frac{M_{bc,m}^{ee,s,*} M_{iq,m}^{ee,s}}{\omega - (\epsilon_b + \epsilon_c - \epsilon_i - 3i\eta)} \\ & - \frac{1}{4} \sum_{ibcm} \frac{(\langle pi|bc\rangle + \langle pi|cb\rangle)}{\epsilon_b + \epsilon_c - \Omega_m^{hh,s} - 3i\eta} \frac{M_{bc,m}^{hh,s,*} M_{iq,m}^{hh,s}}{\omega - (\epsilon_b + \epsilon_c - \epsilon_i - 3i\eta)} - \frac{1}{4} \sum_{ijkm} \frac{(\langle pi|jk\rangle + \langle pi|kj\rangle)}{\Omega_m^{ee,s} - \epsilon_j - \epsilon_k - 2i\eta} \frac{M_{jk,m}^{ee,s,*} M_{iq,m}^{ee,s}}{\omega - (\Omega_m^{ee,s} - \epsilon_i - 2i\eta)}. \end{aligned} \quad (154)$$

The expression of the triplet part of the self-energy in a spatial orbital basis is ([TODO: WRONG SIGN IN COULOMB](#))

$$\begin{aligned}
\Sigma_{pq}^t(\omega) = & \\
& + \frac{3}{4} \sum_{ajkm} \frac{(\langle pa|jk\rangle + \langle pa|kj\rangle)}{\Omega_m^{\text{hh},t} - \epsilon_j - \epsilon_k - i\eta} \frac{M_{jk,m}^{\text{hh},t,*} M_{aq,m}^{\text{hh},t}}{\omega - (\Omega_m^{\text{hh},t} - \epsilon_a + 2i\eta)} - \frac{3}{4} \sum_{ajkm} \frac{(\langle pa|jk\rangle + \langle pa|kj\rangle)}{\Omega_m^{\text{hh},t} - \epsilon_j - \epsilon_k - i\eta} \frac{M_{jk,m}^{\text{hh},t,*} M_{aq,m}^{\text{hh},t}}{\omega - (\epsilon_j + \epsilon_k - \epsilon_a + 3i\eta)} \\
& + \frac{3}{4} \sum_{ajkm} \frac{(\langle pa|jk\rangle + \langle pa|kj\rangle)}{\Omega_m^{\text{ee},t} - \epsilon_j - \epsilon_k - 3i\eta} \frac{M_{jk,m}^{\text{ee},t} M_{aq,m}^{\text{ee},t,*}}{\omega - (\epsilon_j + \epsilon_k - \epsilon_a + 3i\eta)} + \frac{3}{4} \sum_{abcm} \frac{(\langle pa|bc\rangle + \langle pa|cb\rangle)}{\epsilon_b + \epsilon_c - \Omega_m^{\text{hh},t} - 3i\eta} \frac{M_{bc,m}^{\text{hh},t,*} M_{aq,m}^{\text{hh},t}}{\omega - (\Omega_m^{\text{hh},t} - \epsilon_a + 2i\eta)} \quad (155) \\
& + \frac{3}{4} \sum_{ibcm} \frac{(\langle pi|bc\rangle + \langle pi|cb\rangle)}{\epsilon_b + \epsilon_c - \Omega_m^{\text{ee},t} - i\eta} \frac{M_{bc,m}^{\text{ee},t} M_{iq,m}^{\text{ee},t,*}}{\omega - (\Omega_m^{\text{ee},t} - \epsilon_i - 2i\eta)} - \frac{3}{4} \sum_{ibcm} \frac{(\langle pi|bc\rangle + \langle pi|cb\rangle)}{\epsilon_b + \epsilon_c - \Omega_m^{\text{ee},t} - i\eta} \frac{M_{bc,m}^{\text{ee},t} M_{iq,m}^{\text{ee},t,*}}{\omega - (\epsilon_b + \epsilon_c - \epsilon_i - 3i\eta)} \\
& + \frac{3}{4} \sum_{ibcm} \frac{(\langle pi|bc\rangle + \langle pi|cb\rangle)}{\epsilon_b + \epsilon_c - \Omega_m^{\text{hh},t} - 3i\eta} \frac{M_{bc,m}^{\text{hh},t,*} M_{iq,m}^{\text{hh},t}}{\omega - (\epsilon_b + \epsilon_c - \epsilon_i - 3i\eta)} + \frac{3}{4} \sum_{ijkm} \frac{(\langle pi|jk\rangle + \langle pi|kj\rangle)}{\Omega_m^{\text{ee},t} - \epsilon_j - \epsilon_k - 2i\eta} \frac{M_{jk,m}^{\text{ee},t} M_{iq,m}^{\text{ee},t,*}}{\omega - (\Omega_m^{\text{ee},t} - \epsilon_i - 2i\eta)}.
\end{aligned}$$

<sup>1</sup>G. Rohringer, A. Valli, and A. Toschi, “Local electronic correlation at the two-particle level,” *Phys. Rev. B* **86**, 125114 (2012).

<sup>2</sup>R. M. Martin, L. Reining, and D. M. Ceperley, *Interacting Electrons: Theory and Computational Approaches* (Cambridge University Press, 2016).

<sup>3</sup>D. Sangalli, P. Romaniello, G. Onida, and A. Marini, “Double excitations in correlated systems: A many-body approach,” *J. Chem. Phys.* **134**, 034115 (2011).

<sup>4</sup>A. Marie, P. Romaniello, X. Blase, and P.-F. Loos, “Anomalous propagators and the particle–particle channel: Bethe–Salpeter equation,” *J. Chem. Phys.* **162**, 134105 (2025).

<sup>5</sup>E. Monino and P.-F. Loos, “Connections and performances of Green’s function methods for charged and neutral excitations,” *J. Chem. Phys.* **159**, 034105 (2023).

<sup>6</sup>P.-F. Loos and P. Romaniello, “Static and dynamic Bethe–Salpeter equations in the  $T$ -matrix approximation,” *J. Chem. Phys.* **156**, 164101 (2022).
